# Supplementary material for: A Time-Series Model for Areal Data Using Area-Specific Gaussian Processes with Spatially Correlated Hyperparameters
Source: arXiv:2509.01604 ancillary file (2026-08-20)
Supplement: Supplementary file 1 [file SupplementaryMaterial.pdf]

# Supplementary Material for A Time-Series Model for Areal Data Using Spatially Correlated Gaussian Processes

## 1 A spatially correlated Gaussian-process time-series model for areal data

This section provides a detailed description of the multivariate spatio-temporal model we propose, focusing specifically on the case where the response variable follows a Gaussian distribution. While the proposed modeling framework is flexible and can accommodate other distributional assumptions, we restricted our attention here to the Gaussian case. Let  $Y_{it}$  denote the response at region  $i$  and time  $t$ , with the corresponding linear predictor

$$\eta_{it} = \mathbf{X}_i \boldsymbol{\beta}_i + Z_{it} + \epsilon_{it}, \quad (1)$$

where  $\mathbf{X}_i$  denotes the design matrix containing the covariates of interest,  $\boldsymbol{\beta}_i$  the region-specific regression coefficients, and  $\mathbf{Z}_i = (Z_{i1}, \dots, Z_{iT})$  the temporal Gaussian process at region  $i$ , assumed stationary and isotropic, and  $\epsilon_i \sim \mathcal{N}(0, \tau_i^2)$  is a Gaussian noise term representing measurement error or fine-scale variability not captured by the structured components of the model. The Gaussian process is modeled as a zero-mean process with covariance function of the form,

$$\gamma_i(h) = \text{cov}(Z_{it}, Z_{it'}) = \sigma_i^2 \rho_i(h), \quad (2)$$

where  $h$  denotes the Euclidean distance between time points  $t$  and  $t'$ , and  $\rho_i(h)$  is a Matérn correlation function given by

$$\rho_i(h) = \{2^{(\kappa-1)}\Gamma(\kappa)\}^{-1} \left(\frac{h}{\phi_i}\right)^\kappa \kappa_\kappa\left(\frac{h}{\phi_i}\right), h > 0 \quad (3)$$

Here,  $\kappa$  controls the smoothness of the process and it is assumed fixed;  $\phi_i$  is a temporal scale parameter that determines the range of the temporal correlation;  $\Gamma(\cdot)$  is the gamma function; and  $K_\kappa(\cdot)$  is the modified Bessel function of the second kind.

To introduce spatial dependence, we specified spatial priors in a Bayesian context on two key parameters: (i) the log-transformed temporal variance parameters  $(\log(\sigma_1^2), \dots, \log(\sigma_I^2))$  and (ii) the log-transformed range parameter  $\log(\phi_i)$ . Note that in this model, each area  $i$  has associated parameters  $\theta_i = (\beta_i, \sigma_i^2, \phi_i, \nu_i^2)$ , where  $\nu_i^2 = \tau_i^2/\sigma_i^2$  is a signal-to-noise ratio.

## 1.1 Priors definition

We estimate the variance parameters on the log scale to allow the specification of prior distributions supported on the entire real line. Specifically, we assume that the vector of log-variances, denoted by  $\mathbf{log}(\boldsymbol{\sigma}^2) = (\log(\sigma_1^2), \dots, \log(\sigma_I^2))$ , follows a conditionally autoregressive (CAR) prior, specified as

$$\mathbf{log}(\boldsymbol{\sigma}^2) \sim \mathcal{N}(\mathbf{0}, \mathbf{Q}^{-1}), \quad (4)$$

where the precision matrix is defined as  $\mathbf{Q} = \delta^2 \mathbf{K} (\mathbf{I} - \alpha \mathbf{B})$ . Here,  $\delta^2$  is a scalar hyperparameter controlling the overall precision scale and is assumed to follow a Gamma distribution with shape 1 and rate 0.001. The matrix  $\mathbf{K}$  is diagonal, with entries corresponding to the number of neighbors for each spatial unit;  $\mathbf{I}$  denotes the identity matrix; and  $\alpha$  is a spatial smoothing parameter, fixed at 0.9 based on the results of a Besag–York–Mollié (BYM) model fitted to the area-specific variances obtained from independent Gaussian

process models. The matrix  $\mathbf{B} = \mathbf{K}^{-1}\mathbf{W}$ , where  $\mathbf{W}$  is the binary spatial adjacency matrix constructed using Queen contiguity.

The prior distribution associated to  $\log(\phi_i)$  is conditional to  $\log(\sigma_i^2)$ , and it is defined as follows,

$$\log(\phi_i)|\log(\sigma_i^2) \sim N(\mu_{\log(\phi_i)|\log(\sigma_i^2)}, \Sigma_{\phi_i|\log(\sigma_i^2)}), \quad (5)$$

with

$$\mu_{\log(\phi_i)|\log(\sigma_i^2)} = \widehat{\log(\phi_{i_{mle}})} + \frac{\widehat{\text{Cov}}(\log(\phi_i), \log(\sigma_i^2))}{\widehat{\text{Var}}(\log(\sigma_i^2))} (\log(\sigma_i^2) - \widehat{\log(\sigma_{i_{mle}}^2)}), \quad (6)$$

and

$$\Sigma_{\phi_i|\log(\sigma_i^2)} = \widehat{\text{Var}}(\log(\phi_i)) - \frac{\widehat{\text{Cov}}(\log(\phi_i), \log(\sigma_i^2))^2}{\widehat{\text{Var}}(\log(\sigma_i^2))}, \quad (7)$$

where  $\widehat{\log(\phi)}_{i_{mle}}$  and  $\widehat{\log(\sigma_i^2)}_{i_{mle}}$  represent the maximum likelihood estimates of those parameters from the independent Gaussian-process models applied for each of the areas  $i$ . Additionally, the variance and covariance terms in expressions 6 and 7 were also estimated through these area-specific models.

The prior distribution of  $\log(\nu_i^2)$  is defined as follows,

$$\log(\nu_i^2) \sim \mathcal{N}(\mu_{i\nu}, \sigma_{i\nu}^2), \quad (8)$$

where  $\mu_\nu = \widehat{\log(\nu_{i_{mle}})}$  and  $\sigma_{i\nu}^2 = \widehat{\sigma_{i\nu_{mle}}^2}$ . These two values were also obtained from the area-specific Gaussian process models. We opted to use informative prior distributions for the parameters  $\log(\phi_i)$  and  $\log(\nu_i^2)$  as these parameters are known to exhibit slow mixing and potential convergence issues in MCMC sampling.

Finally, the prior distribution associated with the coefficients of the covariates,  $\log(\beta_i) = (\beta_0, \beta_1, \dots, \beta_p)$ , is a non-informative multivariate Gaussian prior  $\log(\beta_i) \sim \mathcal{N}_{p+1}(0, \delta_\beta I_{p+1})$ , with  $p$  denoting the number of covariates and  $\delta_\beta \sim \text{InvGamma}(0.01, 0.01)$ .

## 1.2 Estimation

We perform inference on the parameters of interest  $\boldsymbol{\theta} = (\theta_1, \dots, \theta_I)$  within a Bayesian framework, we treat  $\boldsymbol{\Theta}$  as an unobserved random variable. Inference is based on the posterior distribution  $p(\boldsymbol{\theta} \mid y)$ , which represents the distribution of the parameters given the observed data  $y$ . As is typically the case in hierarchical models, the posterior distribution does not have a closed-form expression. We therefore make use of approximations via posterior sampling, specifically using Markov chain Monte Carlo (MCMC) methods.

Given the hierarchical structure of the model, different sampling strategies are employed depending on the form of the full conditional distributions. The MCMC algorithm proceeds iteratively, with each iteration  $k + 1$  consisting of the following components.

**Step 1 – Sampling variance parameters:** At the beginning of each MCMC iteration, we update the Gaussian processes’ variance parameters,  $\mathbf{log}(\boldsymbol{\sigma}^2) = (\log(\sigma_1^2), \dots, \log(\sigma_I^2))$ , using the Metropolis–adjusted Langevin Algorithm (MALA).

Let  $\mathbf{log}(\boldsymbol{\sigma}^2)^{(k)}$  denote the current state of the chain at iteration  $k$ . Under MALA, a new proposal  $\widetilde{\mathbf{log}(\boldsymbol{\sigma}^2)}$  for iteration  $k + 1$  is generated using both the gradient of the log-posterior and a random perturbation. The update proceeds in two sub-steps:

1. Compute the gradient of the log-posterior distribution with respect to  $\mathbf{log}(\boldsymbol{\sigma}^2)$ , evaluated at  $\mathbf{log}(\boldsymbol{\sigma}^2)^{(k)}$ .
2. Generate the proposal  $\widetilde{\mathbf{log}(\boldsymbol{\sigma}^2)}$  by combining a deterministic term and a stochastic noise term:

$$\widetilde{\mathbf{log}(\boldsymbol{\sigma}^2)} = \mathbf{log}(\boldsymbol{\sigma}^2)^{(k)} + \frac{\epsilon^2}{2} \nabla \log \pi(\mathbf{log}(\boldsymbol{\sigma}^2)^{(k)}) + \iota \mathbf{z},$$

where  $\iota$  is the step size,  $\mathbf{z} \sim \mathcal{N}(\mathbf{0}, \mathbf{I})$ , and  $\nabla \log \pi(\cdot)$  denotes the gradient of the log-posterior density with respect to  $\log(\boldsymbol{\sigma}^2)$ .

The acceptance probability,  $\alpha_\sigma$ , is then computed using the standard MALA acceptance ratio, accounting for the asymmetric proposal distribution. As a final step, a random

number  $u$  is generated from an uniform distribution  $U(0, 1)$ ; we accept the proposal value if  $u < \alpha_\sigma$  and reject it otherwise.

To ensure the relatively high efficiency of the algorithm, the overall acceptance rate should be around 0.57. The step size,  $\iota$ , should be tuned to reach this acceptance probability. We opt for automatic tuning, at each iteration  $k$ , where we calculate the value of  $\iota$  at iteration  $k + 1$ , as follows,

$$\sqrt{\iota^{(k+1)}} = H\left(\sqrt{\iota^{(k)}} + \gamma^{(k)}(\alpha_\sigma^k - 0.57)\right), \quad (9)$$

with

$$H(\omega) = \begin{cases} v & \text{if } \omega < v \\ \omega & \text{if } \omega \in (v, A) \\ A & \text{if } \omega > A, \end{cases} \quad (10)$$

with  $v$  being a small number, precisely  $10^{-4}$  and  $A$  being a large number,  $10^4$ . The series  $\{\gamma^{(k)}\}$  is a non-increasing sequence of positive real numbers such that  $|\gamma^{(k)} - \gamma^{(k-1)}| \leq k^{-1}$ .

We chose  $\gamma^{(k)} = k^{-1}$ .

**Step 2 – Sampling remaining area-specific parameters:** For each spatial unit  $i = 1, \dots, I$ , the remaining parameters are updated conditional on the current values at iteration  $k$ , in the following order: (i) the log-range parameter,  $\log(\phi_i)$ , sampled using MALA conditional on  $\sigma_i^2$ ; (ii) the log signal-to-noise ratio,  $\log(\nu_i^2)$ , sampled via an independent Metropolis–Hastings (MH) step; (iii) the regression coefficients,  $\beta_i$ , sampled from their multivariate Gaussian full conditional distribution using a Gibbs sampler; and (iv) the temporal Gaussian process  $\Delta_i$ , also sampled via Gibbs sampling.

The log-range parameter  $\log(\phi_i)$  is sampled using the Metropolis–adjusted Langevin Algorithm (MALA), following the same steps and structure as used for updating  $\log(\sigma_i^2)$ . This includes using the gradient of the log-posterior with respect to  $\log(\phi_i)$  and construct-

ing the proposal that incorporates both a deterministic and stochastic term to improve convergence and mixing. We also opt for automatic tuning of the step size to reach the overall acceptance rate of 0.57.

To sample from the full conditional posterior distribution of  $\log(\nu_i^2)$ , we adopt an independent Metropolis–Hastings algorithm. Let  $\log(\nu_i^2)^{(k)}$  denote the current state of the chain at iteration  $k$ . The proposal  $\widetilde{\log(\nu_i^2)}$  at iteration  $k + 1$  is drawn from a normal distribution centered at the mode of the posterior, given by the maximum a posteriori (MAP) estimate. The proposal distribution is specified as:

$$\widetilde{\log(\nu_i^2)} \sim \mathcal{N}(\log(\nu_i^2)_{MAP}, -\mathcal{H}^{-1}), \quad (11)$$

where  $\log(\nu_i^2)_{MAP}$  is the MAP estimate, and  $\mathcal{H}$  is the Hessian matrix of the log-posterior evaluated at the MAP. This proposal exploits curvature information from the posterior to improve mixing.

For the regression coefficients  $\beta_i$  and the temporal random effects  $\Delta_i$ , we use Gibbs sampling, as their full conditional distributions are available in closed form. Similarly, we sample the temporal Gaussian process  $\Delta_i$  using Gibbs sampling due to the tractability of their full conditionals. Similarly, the temporal Gaussian process  $\Delta_i$  are updated via Gibbs sampling from their full conditional distribution.

## 2 Results

### 2.1 Malaria incidence in Niassa, Mozambique - Results by district

Figures S1, S2, S3, S4, S5, S6, S7, S8, and S9 present the convergence diagnostic plots for Lichinga. These diagnostics include the trace plot, histogram, autocorrelogram, and running Geweke plot.

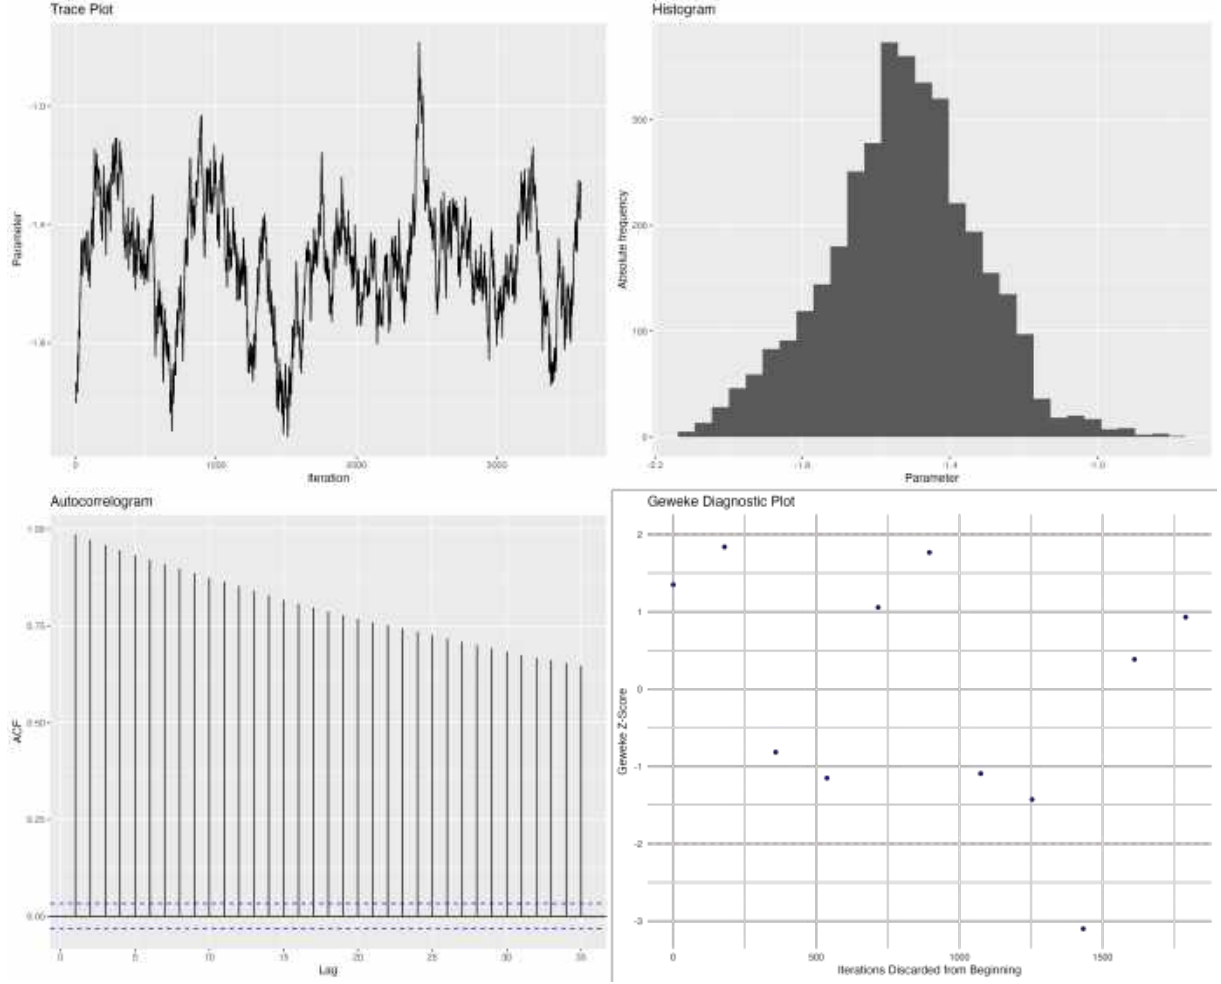

Figure S1: Convergence diagnostic plots for the parameter  $\log(\sigma^2)$  in the district of Lichinga. The panels display: trace plot (top-left), histogram (top-right), autocorrelogram (bottom-left), and running Geweke plot (bottom-right).

Similarly, Figures S10, S11, S12, S13, S14, S15, S16, S17, and S18 show the convergence diagnostics for Majune.

Figures S19, S20, S21, S22, S23, S24, S25, S26, and S27 correspond to Mecanhelas.

Figures S28, S29, S30, S31, S32, S33, S34, S35, and S36 to Sanga.

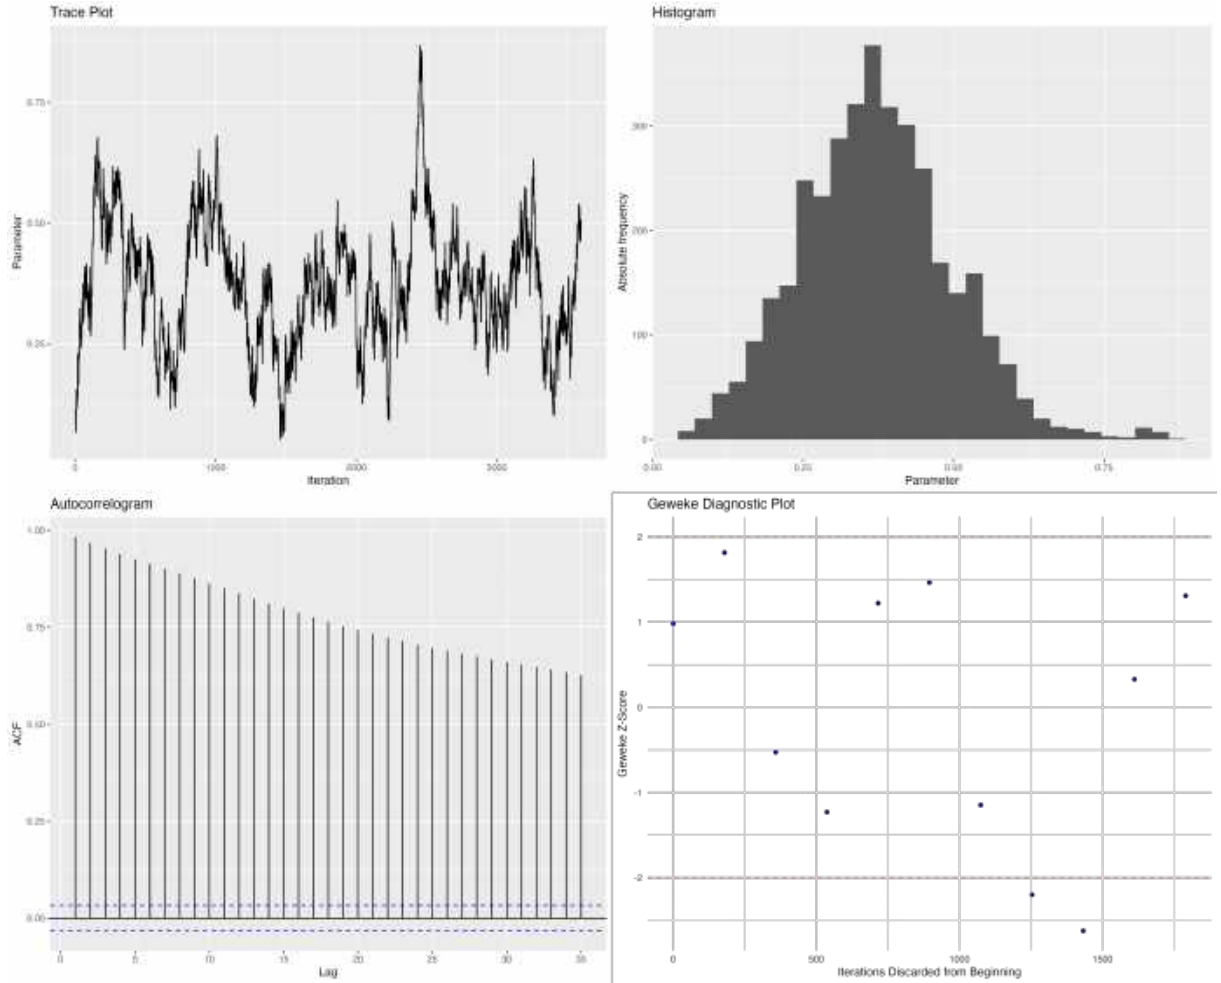

Figure S2: Convergence diagnostic plots for the parameter  $\log(\phi)$  in the district of Lichinga. The panels display: trace plot (top-left), histogram (top-right), autocorrelogram (bottom-left), and running Geweke plot (bottom-right).



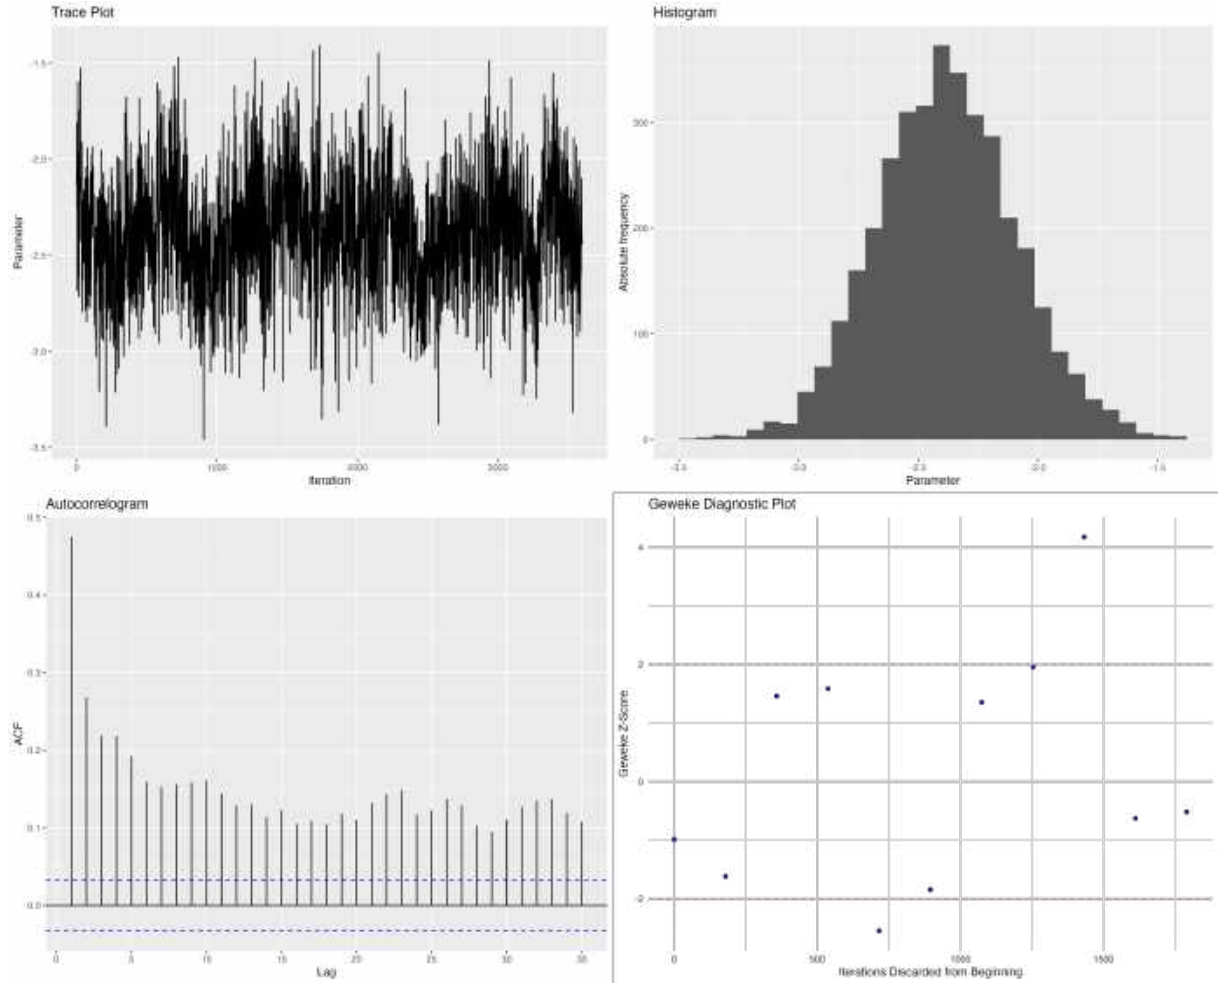

Figure S3: Convergence diagnostic plots for the parameter  $\log(\nu^2)$  in the district of Lichinga. The panels display: trace plot (top-left), histogram (top-right), autocorrelogram (bottom-left), and running Geweke plot (bottom-right).

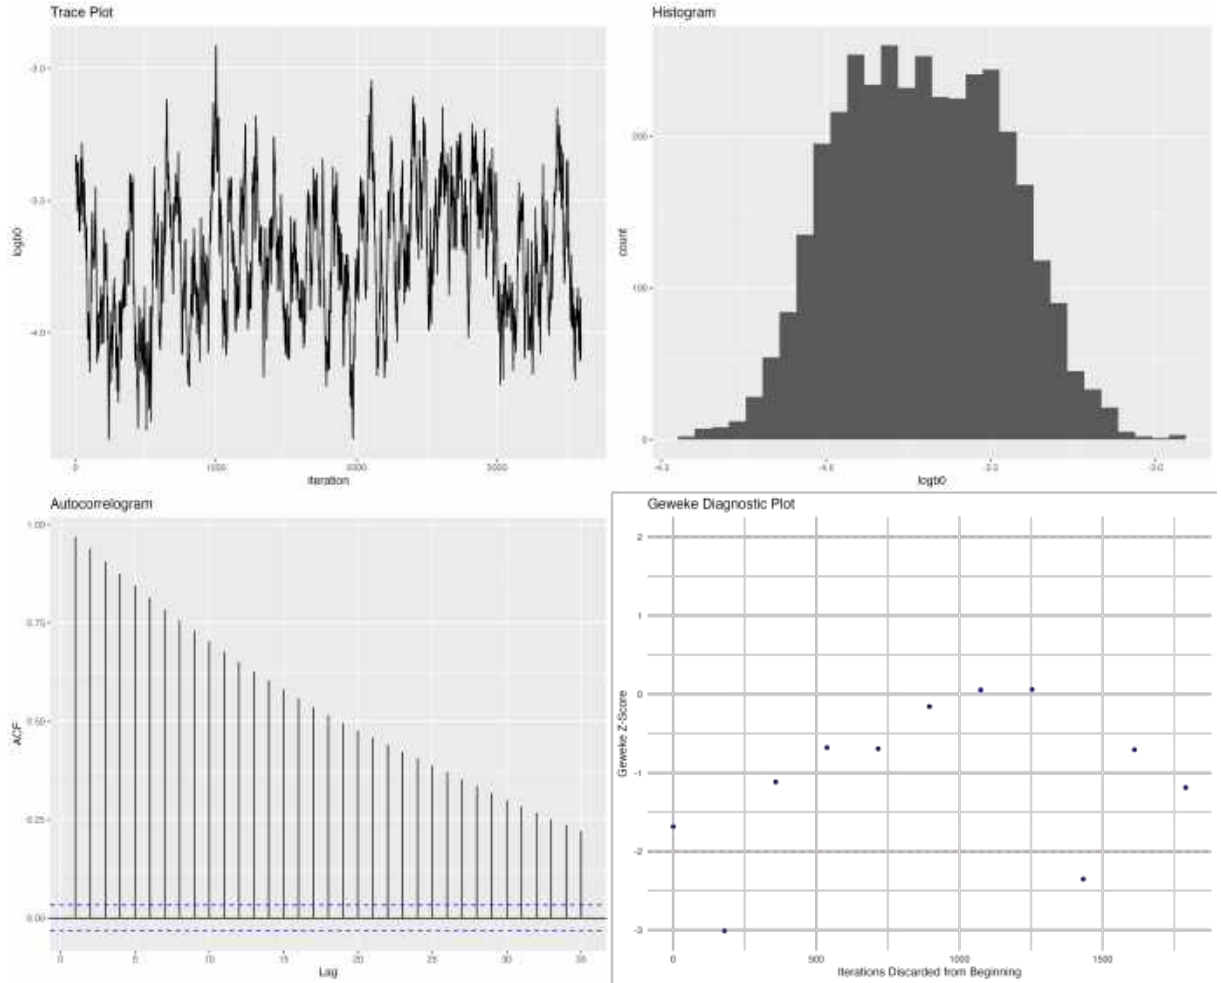

Figure S4: Convergence diagnostic plots for the parameter  $\log(\beta_0)$  in the district of Lichinga. The panels display: trace plot (top-left), histogram (top-right), autocorrelogram (bottom-left), and running Geweke plot (bottom-right).

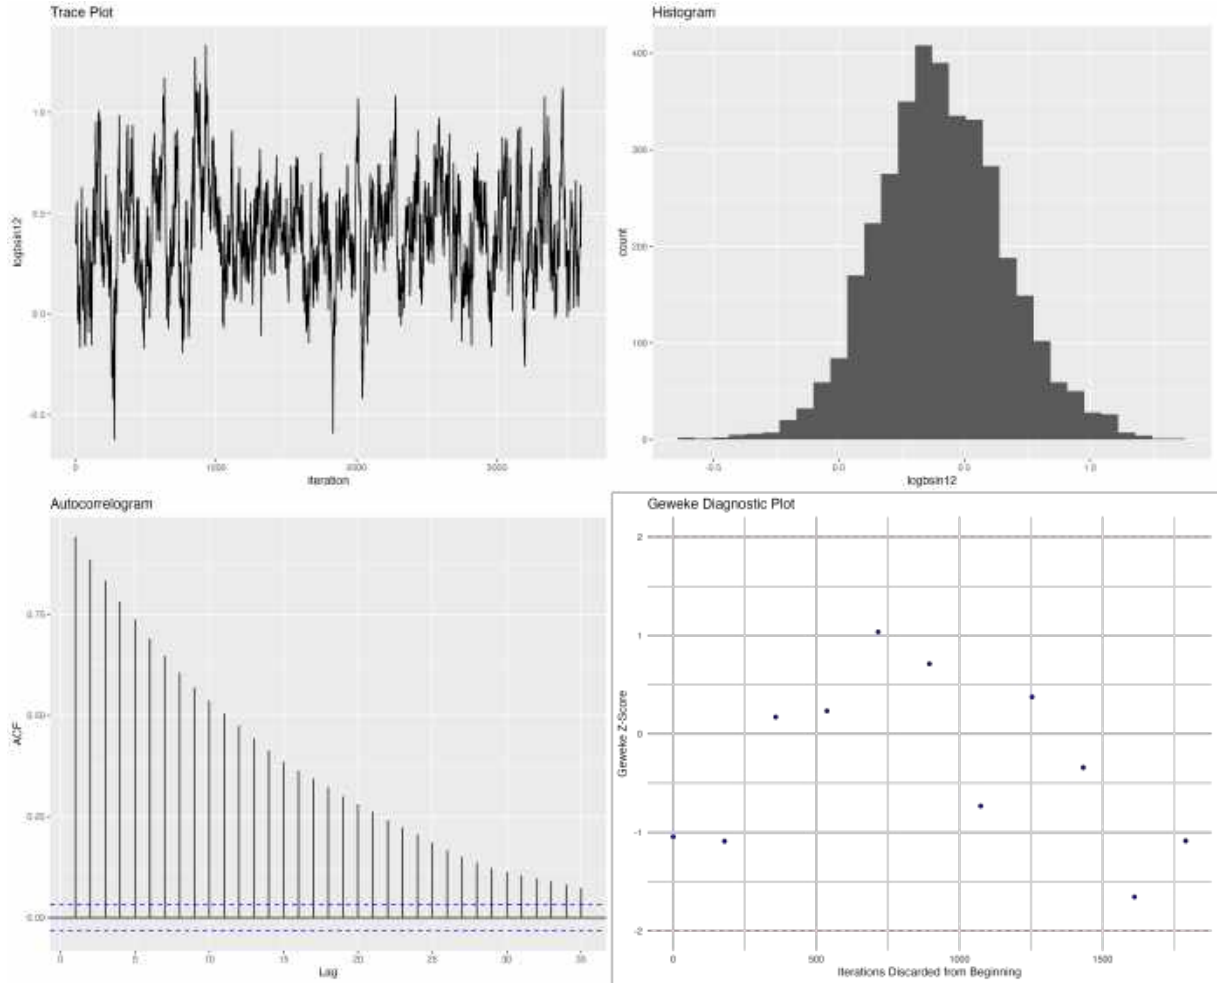

Figure S5: Convergence diagnostic plots for the parameter  $\log(\beta_1)$  in the district of Lichinga. The panels display: trace plot (top-left), histogram (top-right), autocorrelogram (bottom-left), and running Geweke plot (bottom-right).

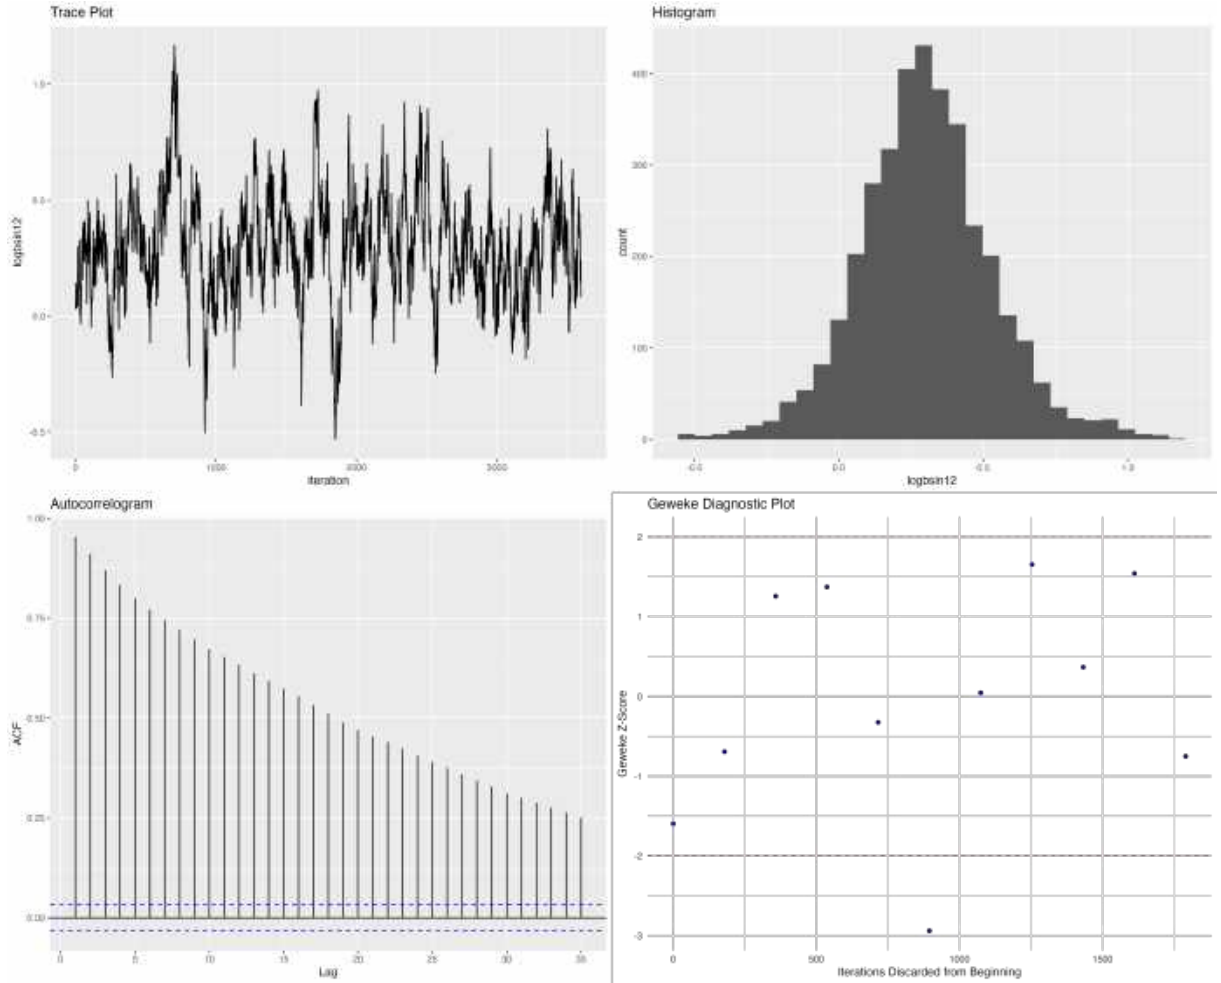

Figure S6: Convergence diagnostic plots for the parameter  $\log(\beta_2)$  in the district of Lichinga. The panels display: trace plot (top-left), histogram (top-right), autocorrelogram (bottom-left), and running Geweke plot (bottom-right).

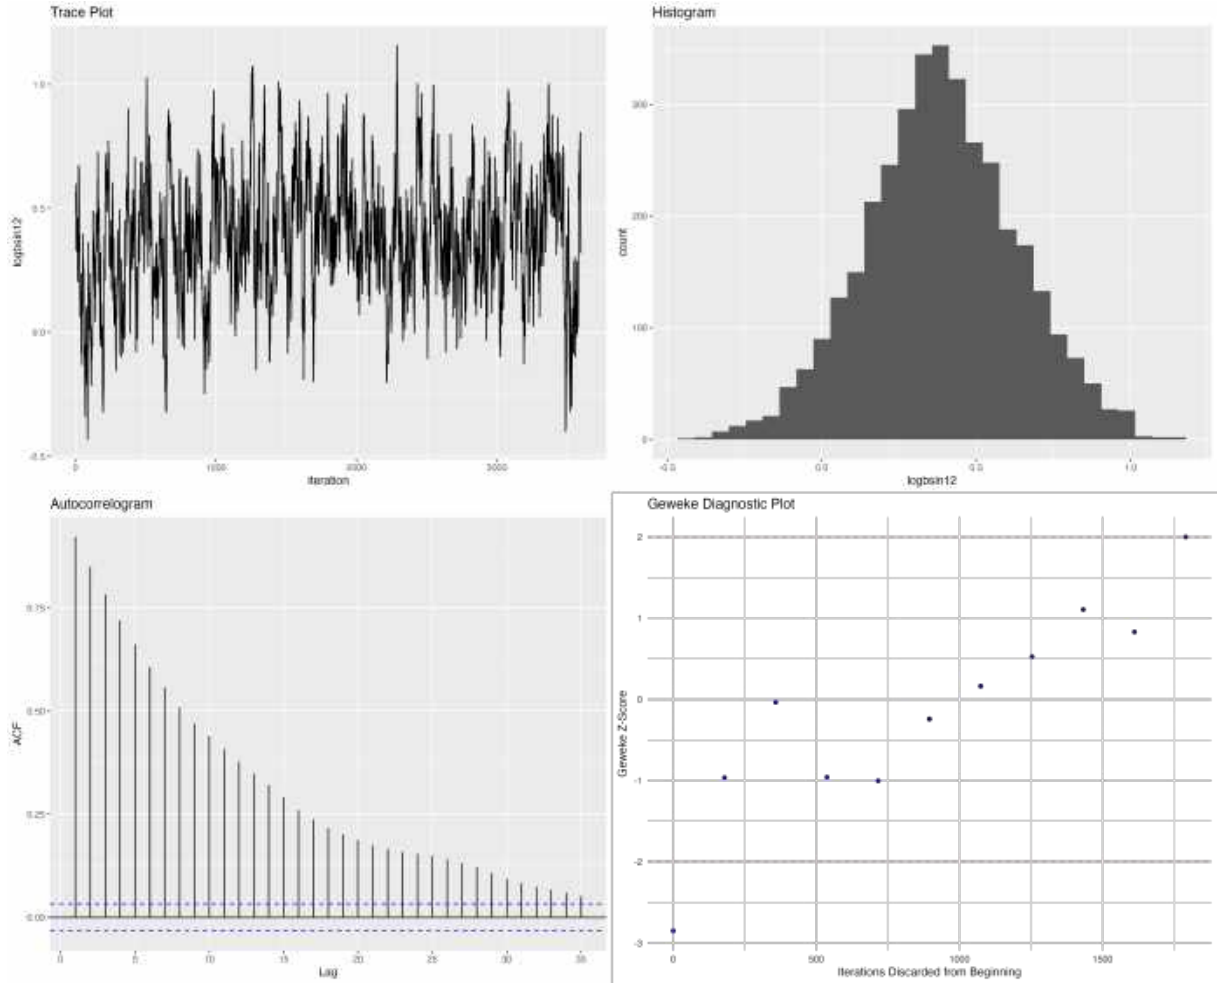

Figure S7: Convergence diagnostic plots for the parameter  $\log(\beta_3)$  in the district of Lichinga. The panels display: trace plot (top-left), histogram (top-right), autocorrelogram (bottom-left), and running Geweke plot (bottom-right).

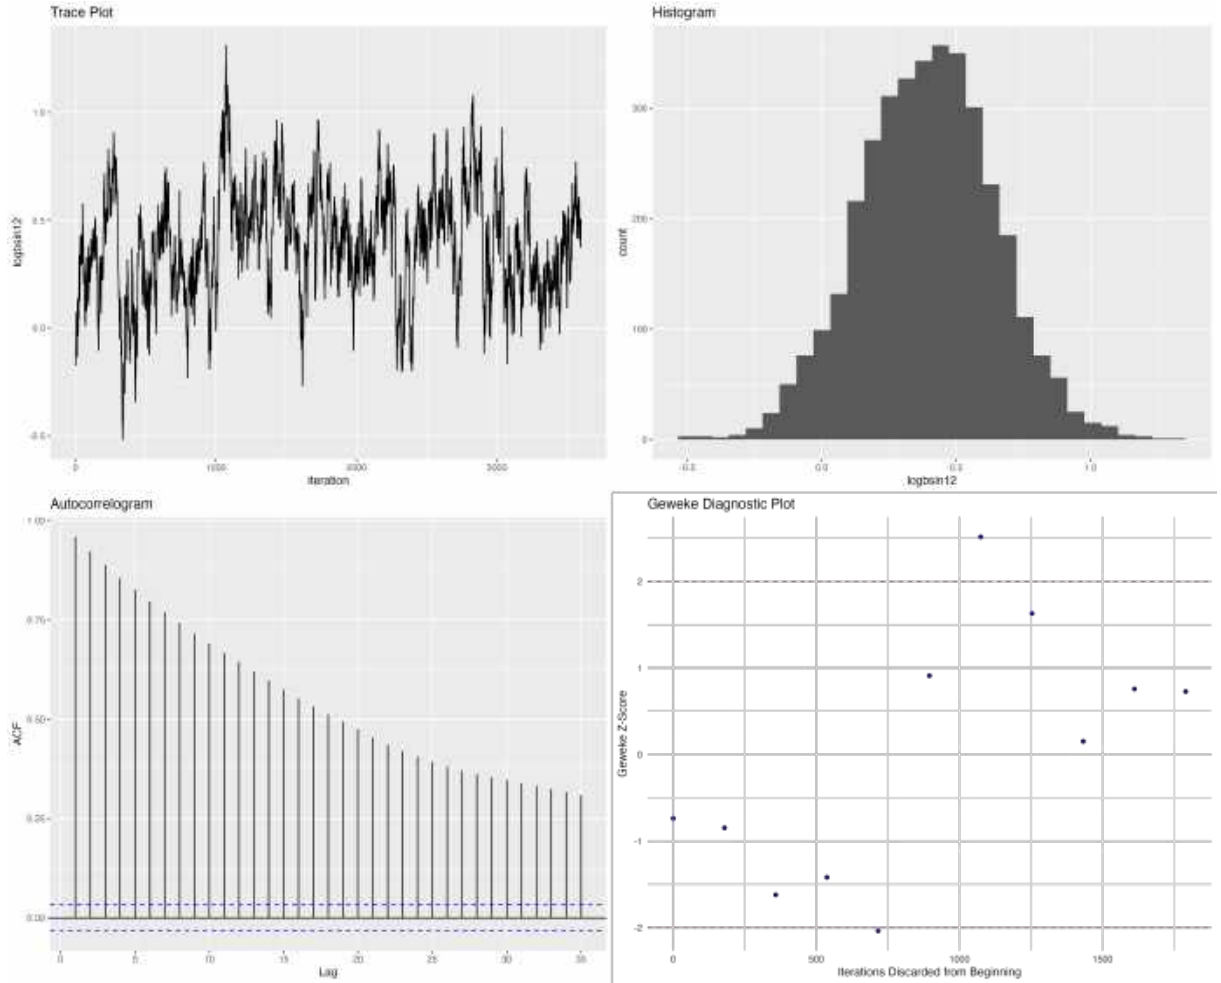

Figure S8: Convergence diagnostic plots for the parameter  $\log(\beta_4)$  in the district of Lichinga. The panels display: trace plot (top-left), histogram (top-right), autocorrelogram (bottom-left), and running Geweke plot (bottom-right).

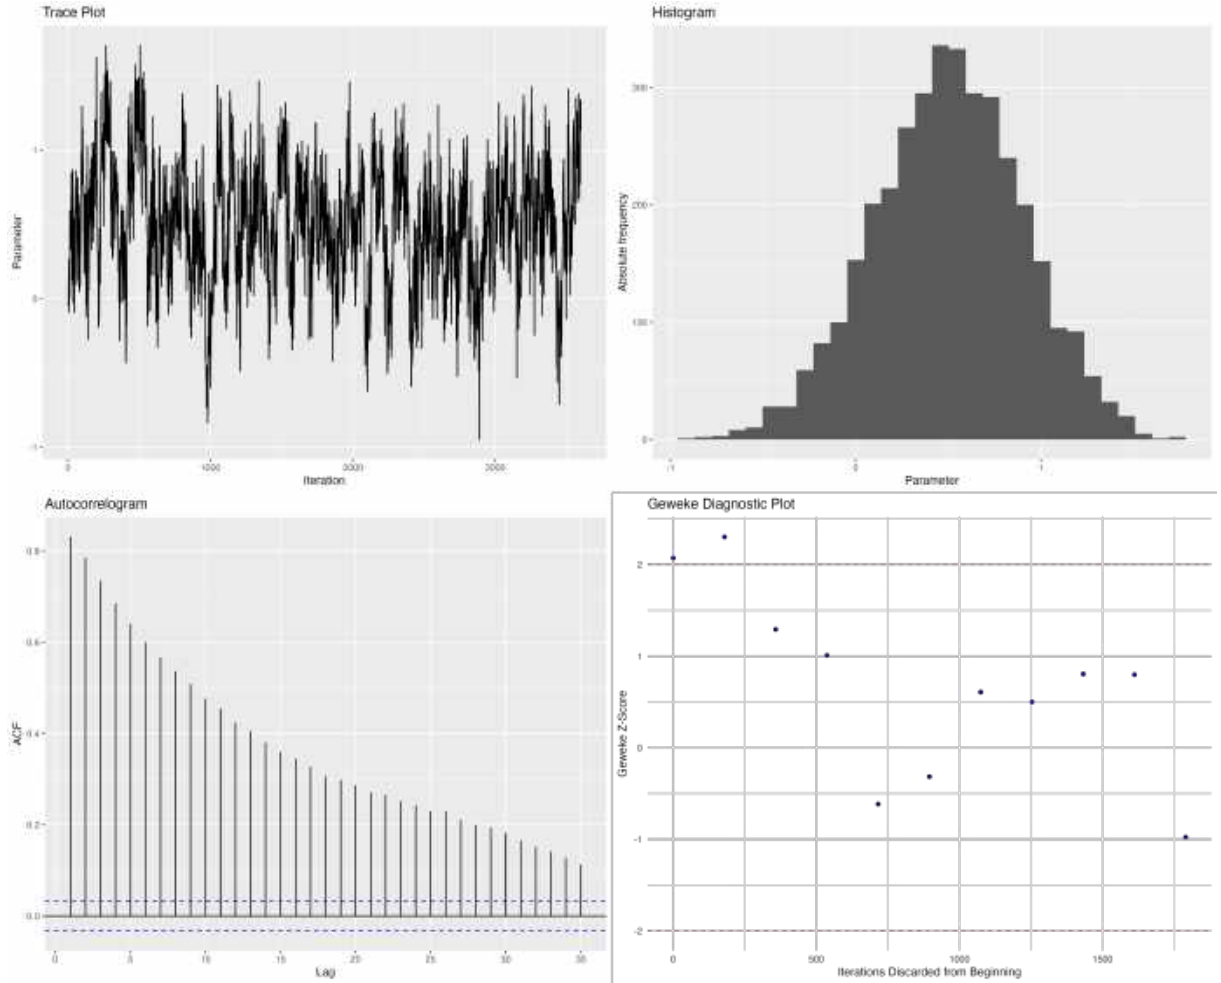

Figure S9: Convergence diagnostic plots for the parameter  $S_{11}$  in the district of Lichinga. The panels display: trace plot (top-left), histogram (top-right), autocorrelogram (bottom-left), and running Geweke plot (bottom-right).

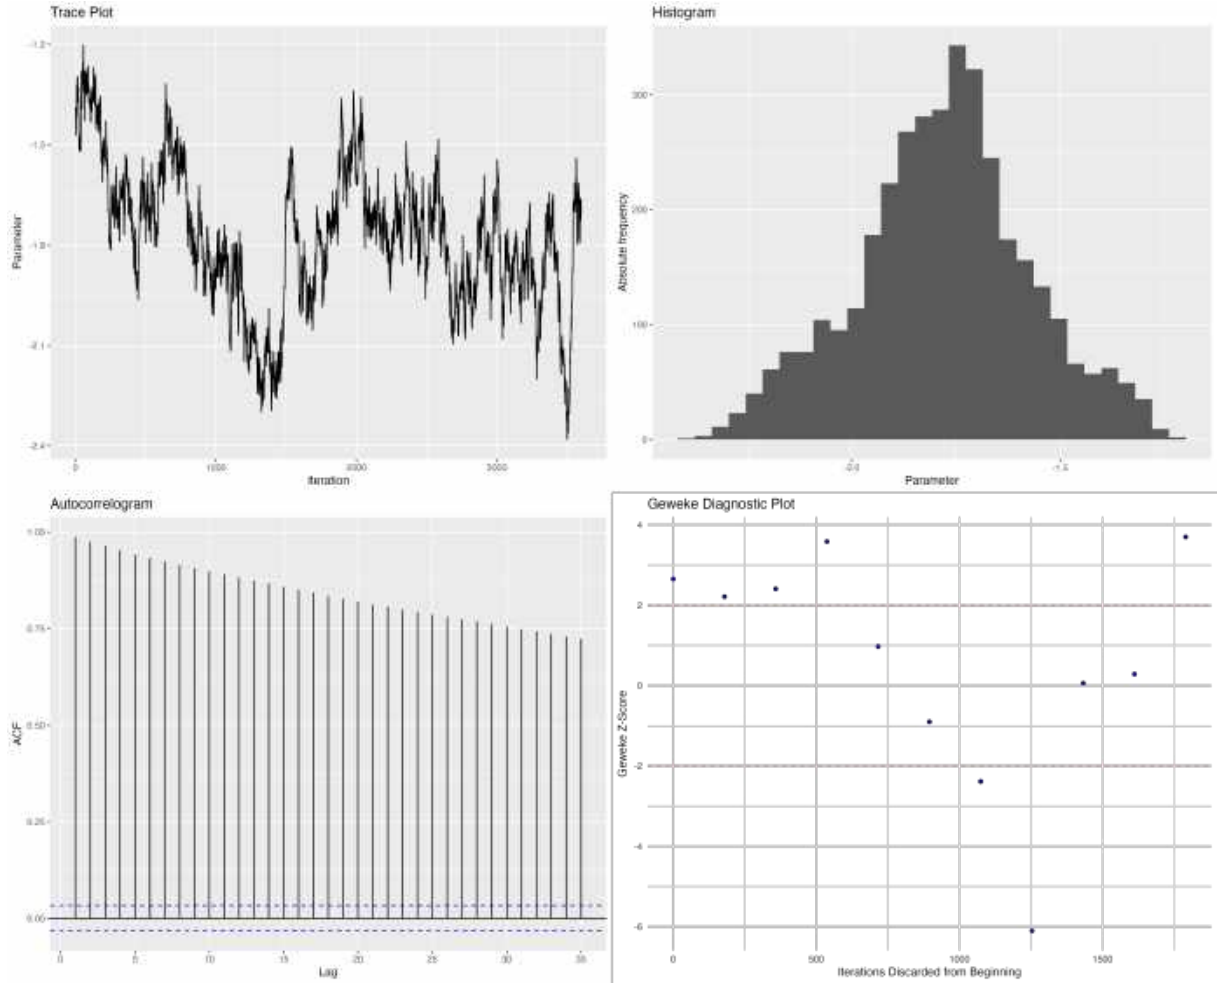

Figure S10: Convergence diagnostic plots for the parameter  $\log(\sigma^2)$  in the district of Majune. The panels display: trace plot (top-left), histogram (top-right), autocorrelogram (bottom-left), and running Geweke plot (bottom-right).



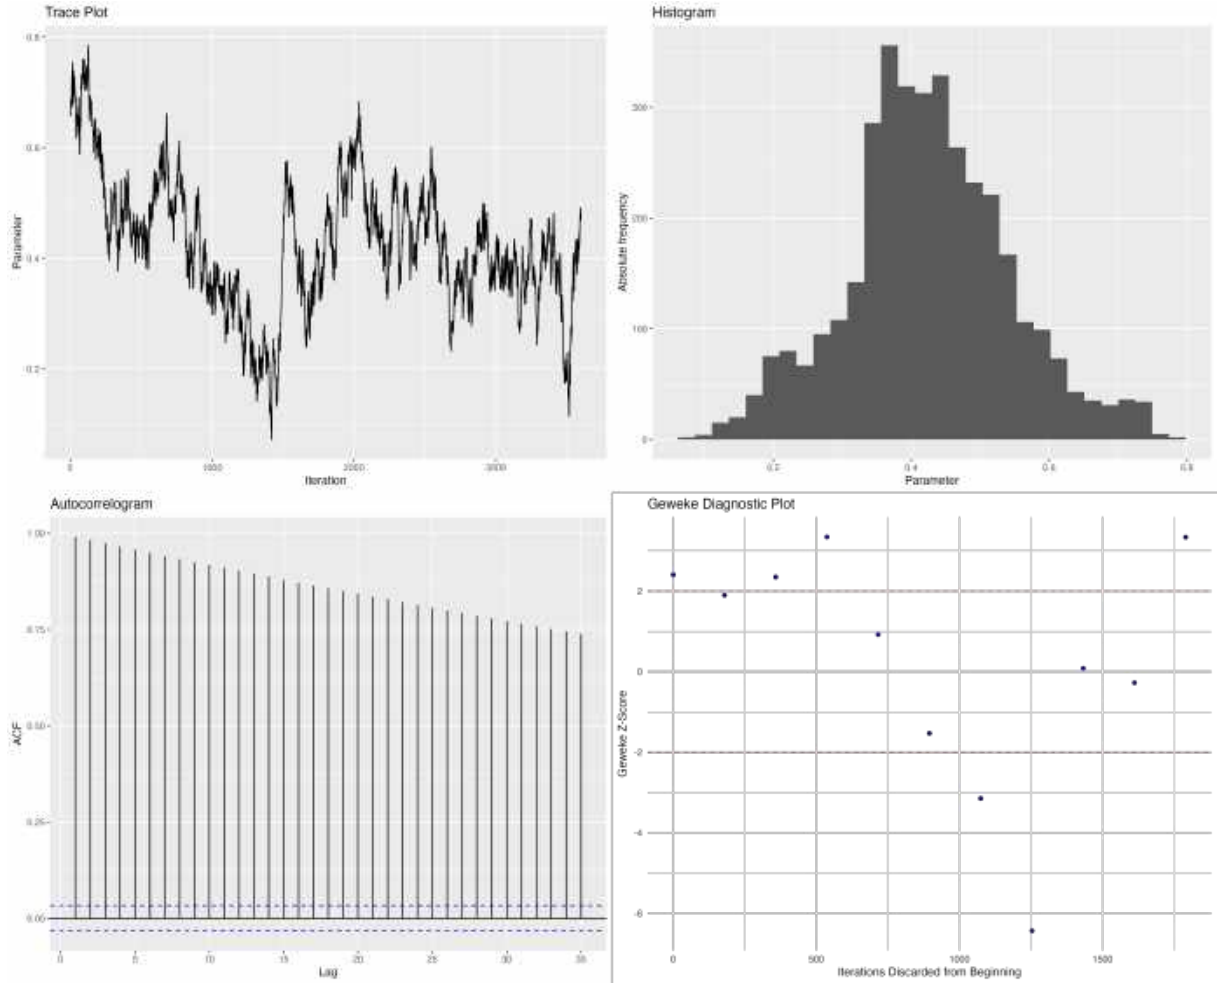

Figure S11: Convergence diagnostic plots for the parameter  $\log(\phi)$  in the district of Majune. The panels display: trace plot (top-left), histogram (top-right), autocorrelogram (bottom-left), and running Geweke plot (bottom-right).

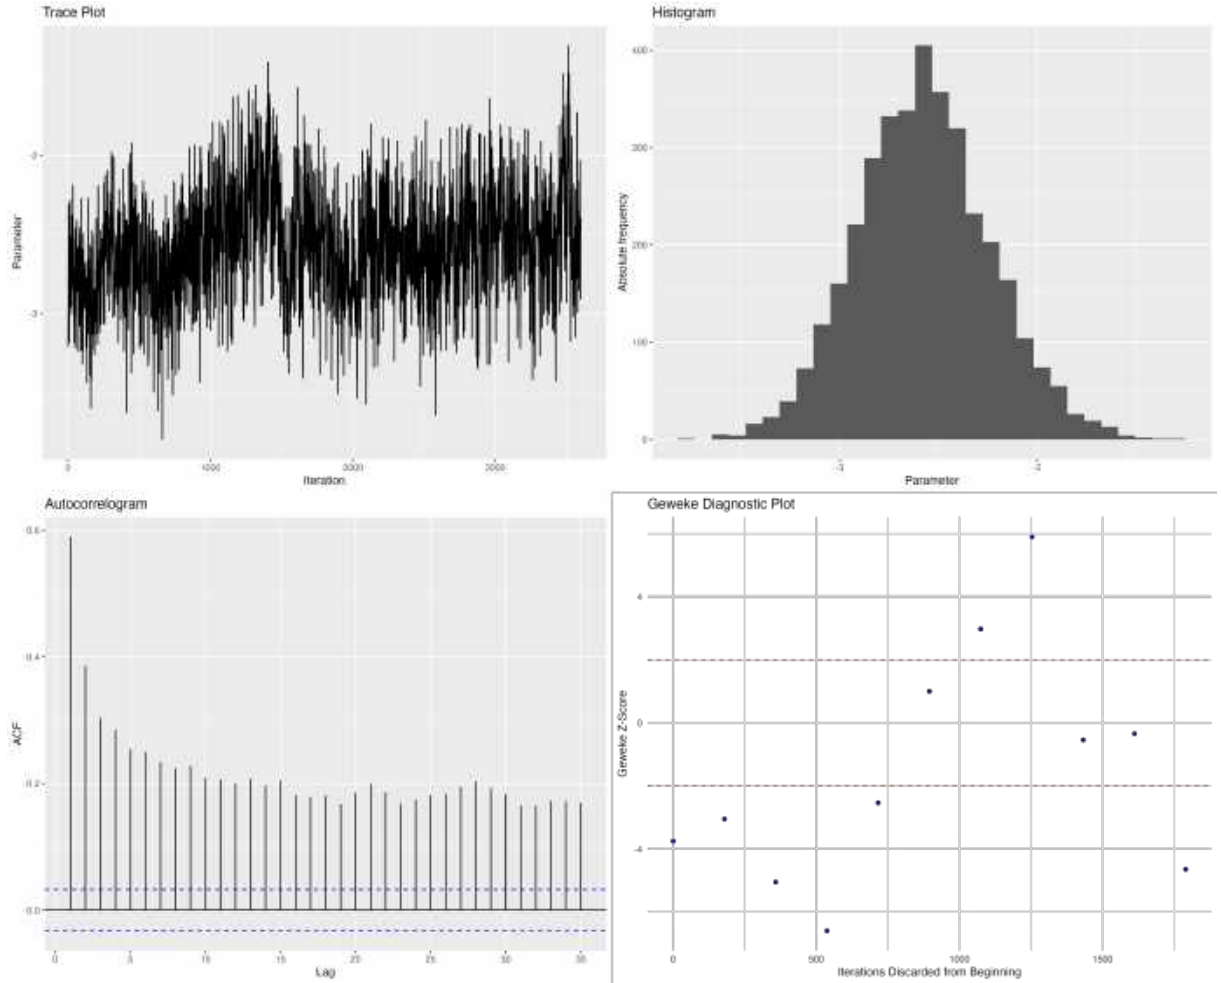

Figure S12: Convergence diagnostic plots for the parameter  $\log(\nu^2)$  in the district of Majune. The panels display: trace plot (top-left), histogram (top-right), autocorrelogram (bottom-left), and running Geweke plot (bottom-right).

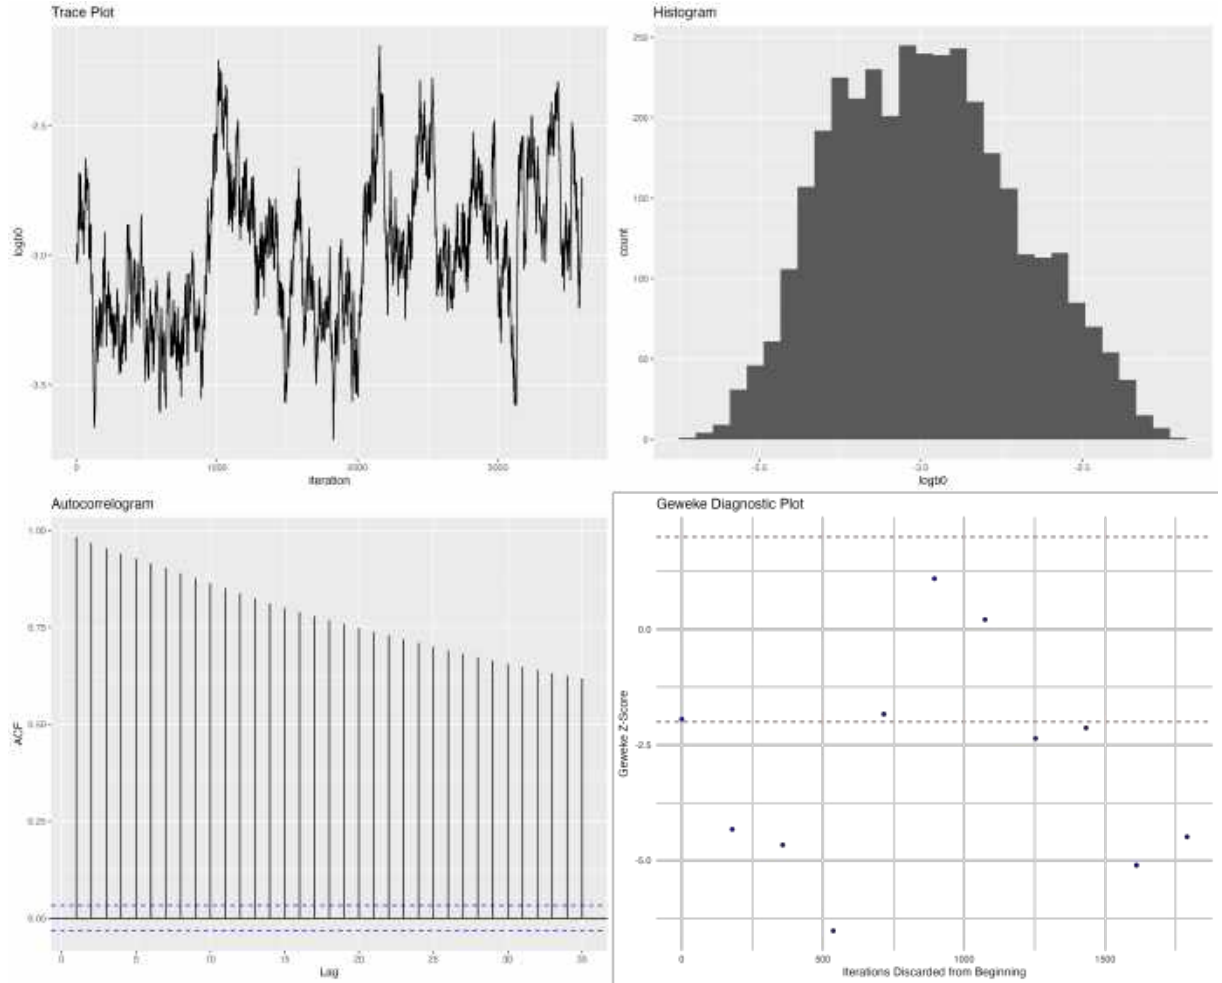

Figure S13: Convergence diagnostic plots for the parameter  $\log(\beta_0)$  in the district of Majune. The panels display: trace plot (top-left), histogram (top-right), autocorrelogram (bottom-left), and running Geweke plot (bottom-right).

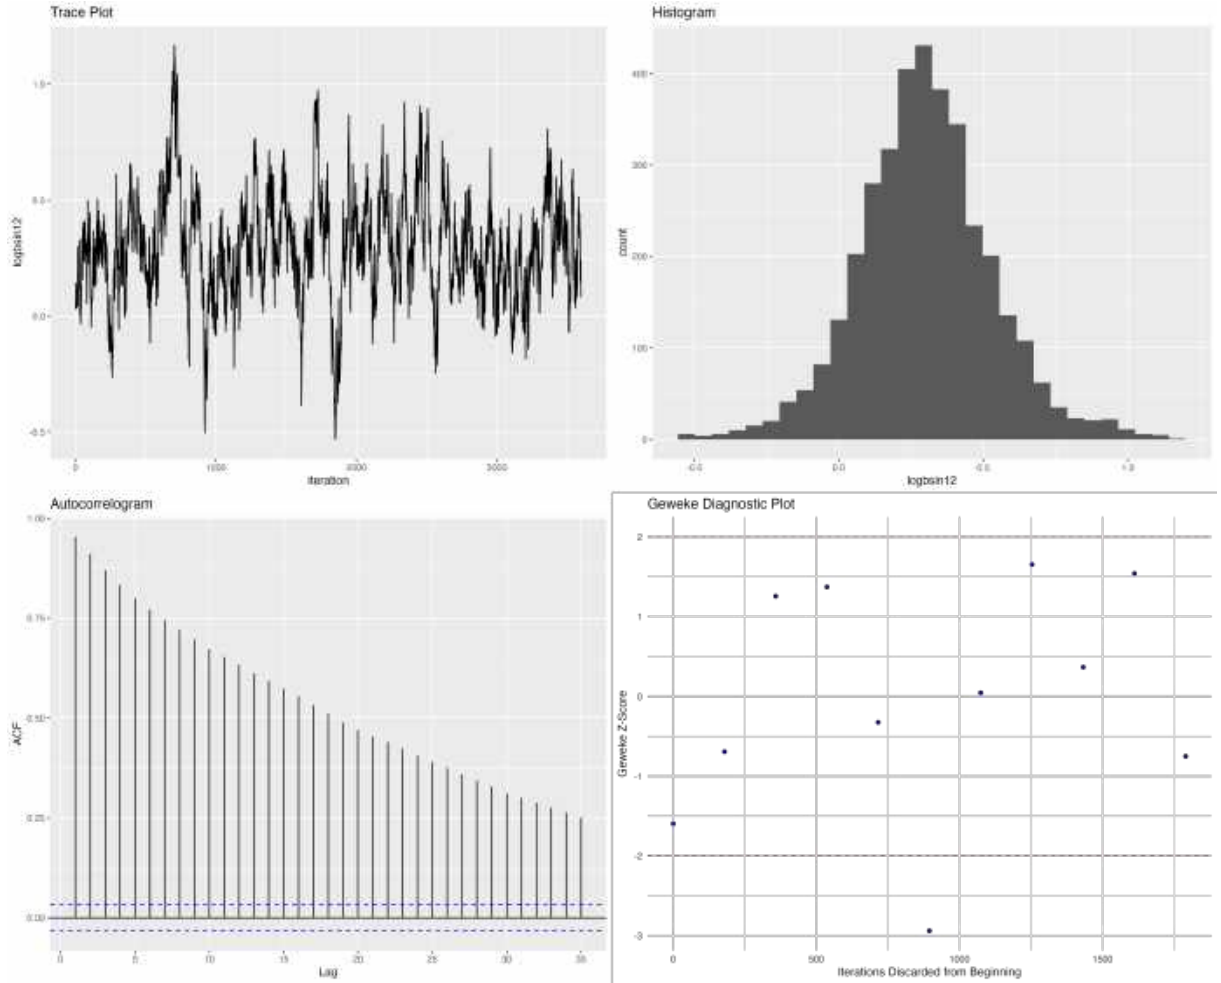

Figure S14: Convergence diagnostic plots for the parameter  $\log(\beta_1)$  in the district of Majune. The panels display: trace plot (top-left), histogram (top-right), autocorrelogram (bottom-left), and running Geweke plot (bottom-right).

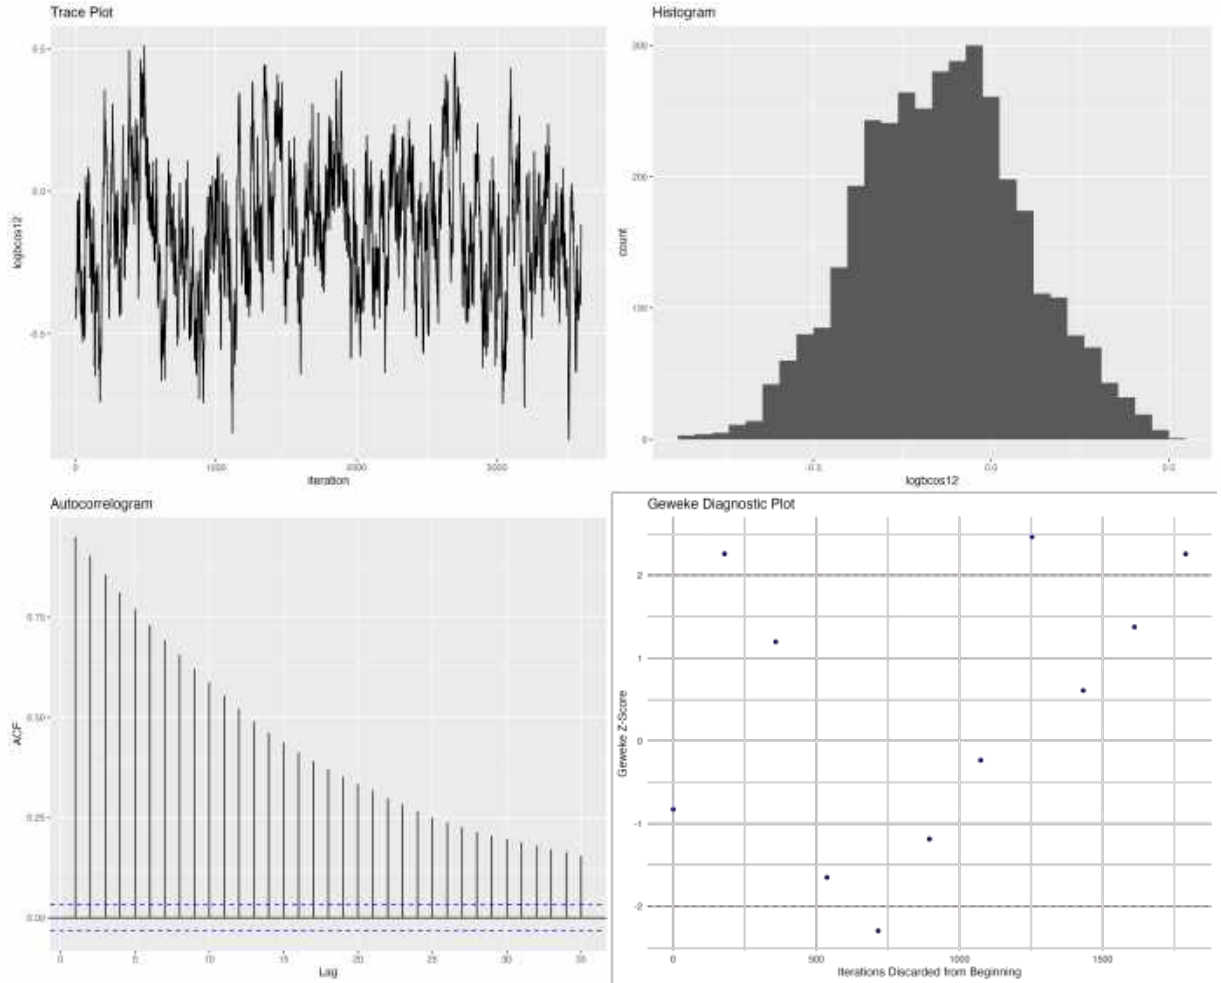

Figure S15: Convergence diagnostic plots for the parameter  $\log(\beta_2)$  in the district of Majune. The panels display: trace plot (top-left), histogram (top-right), autocorrelogram (bottom-left), and running Geweke plot (bottom-right).

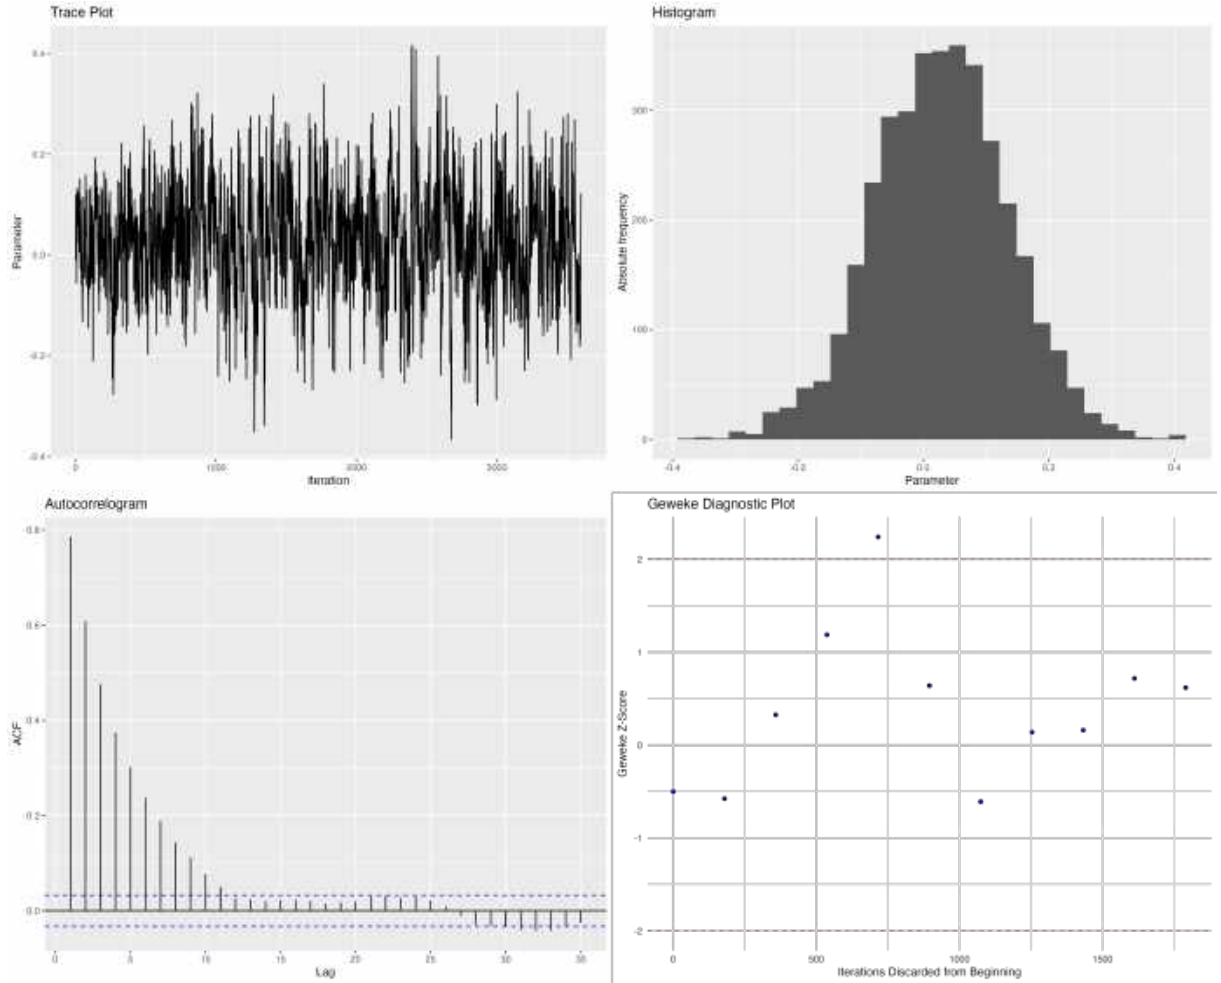

Figure S16: Convergence diagnostic plots for the parameter  $\log(\beta_3)$  in the district of Majune. The panels display: trace plot (top-left), histogram (top-right), autocorrelogram (bottom-left), and running Geweke plot (bottom-right).

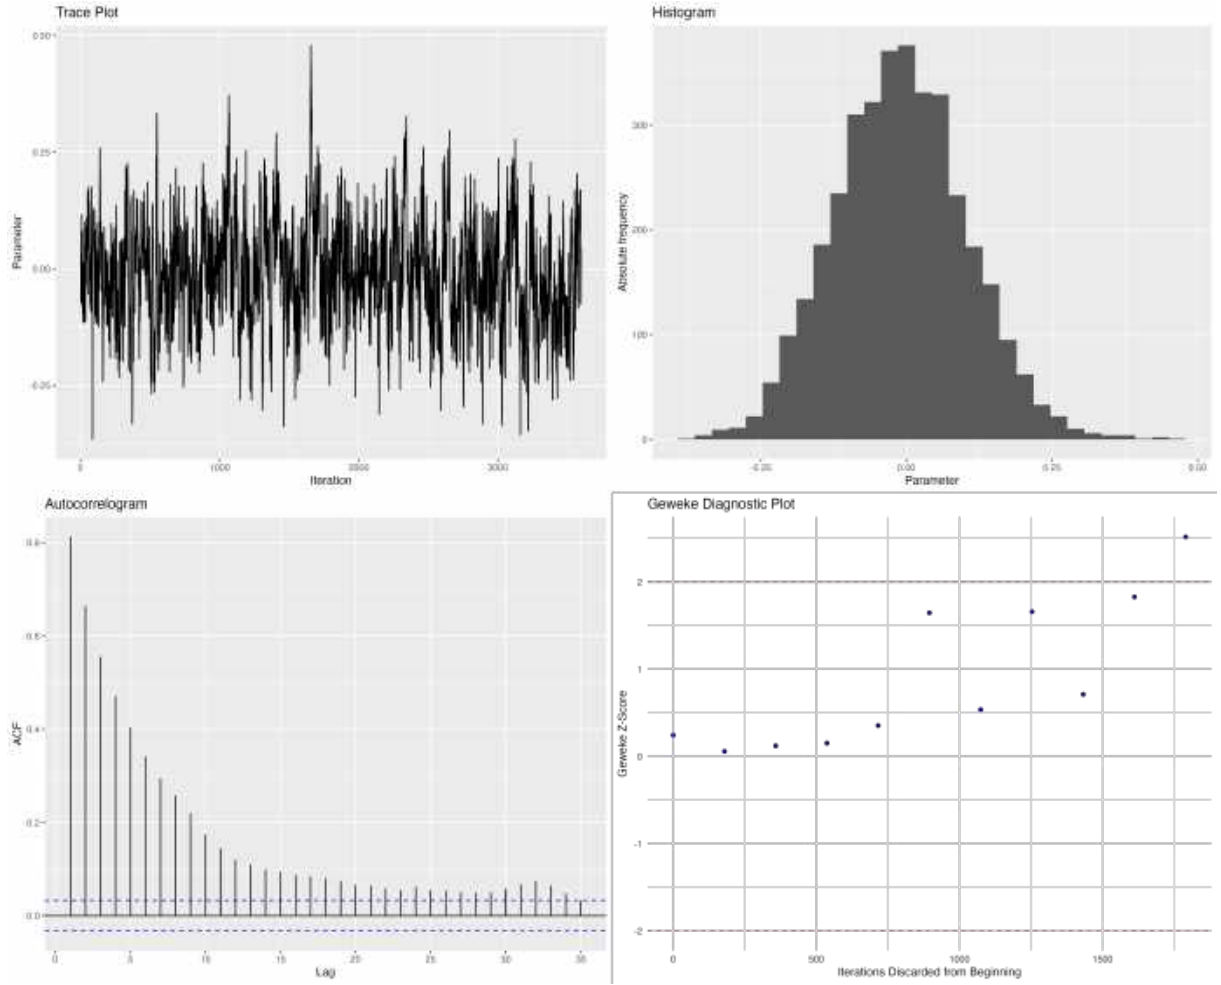

Figure S17: Convergence diagnostic plots for the parameter  $\log(\beta_4)$  in the district of Majune. The panels display: trace plot (top-left), histogram (top-right), autocorrelogram (bottom-left), and running Geweke plot (bottom-right).

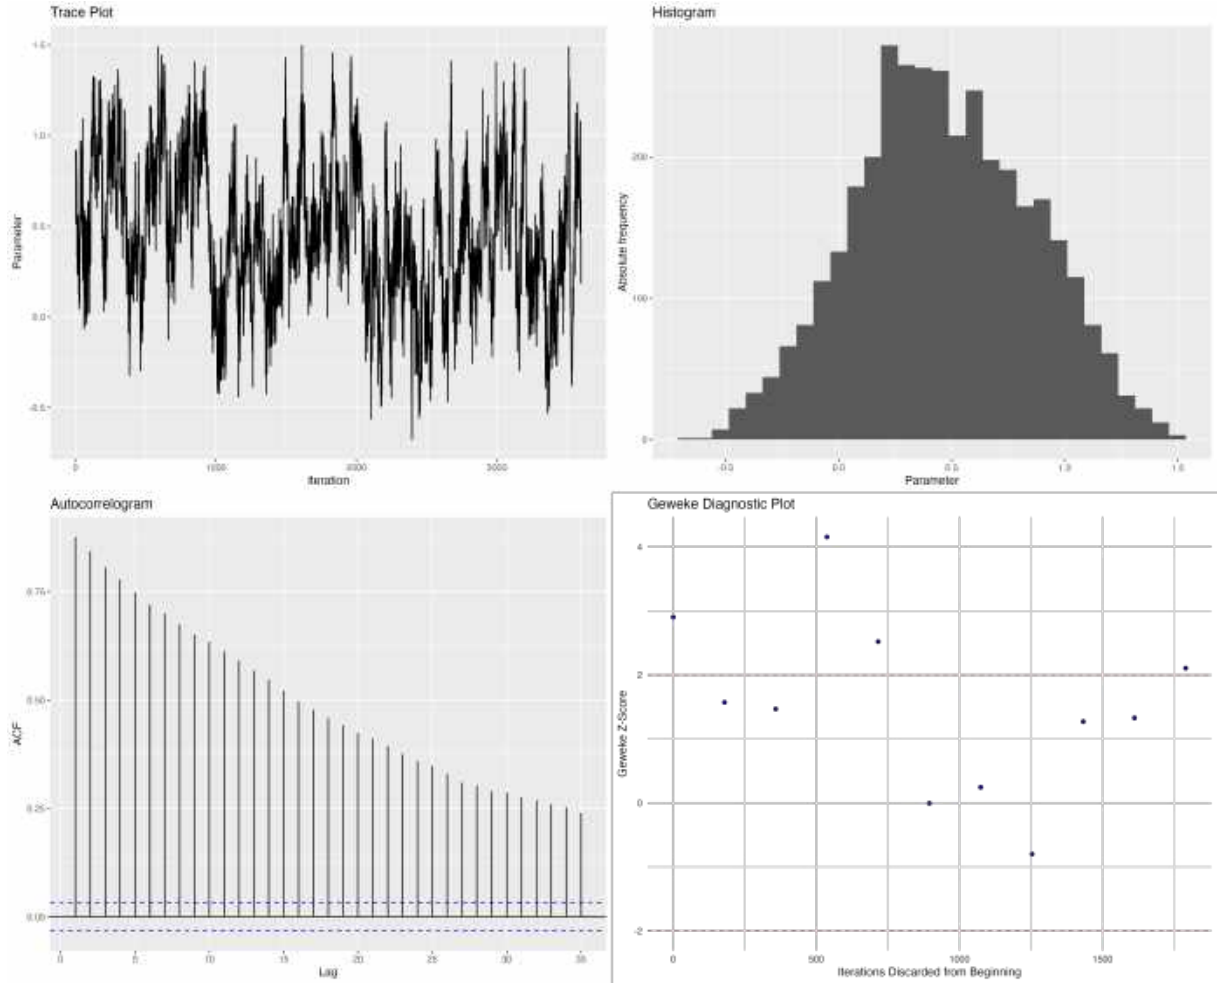

Figure S18: Convergence diagnostic plots for the parameter  $S_{11}$  in the district of Majune. The panels display: trace plot (top-left), histogram (top-right), autocorrelogram (bottom-left), and running Geweke plot (bottom-right).



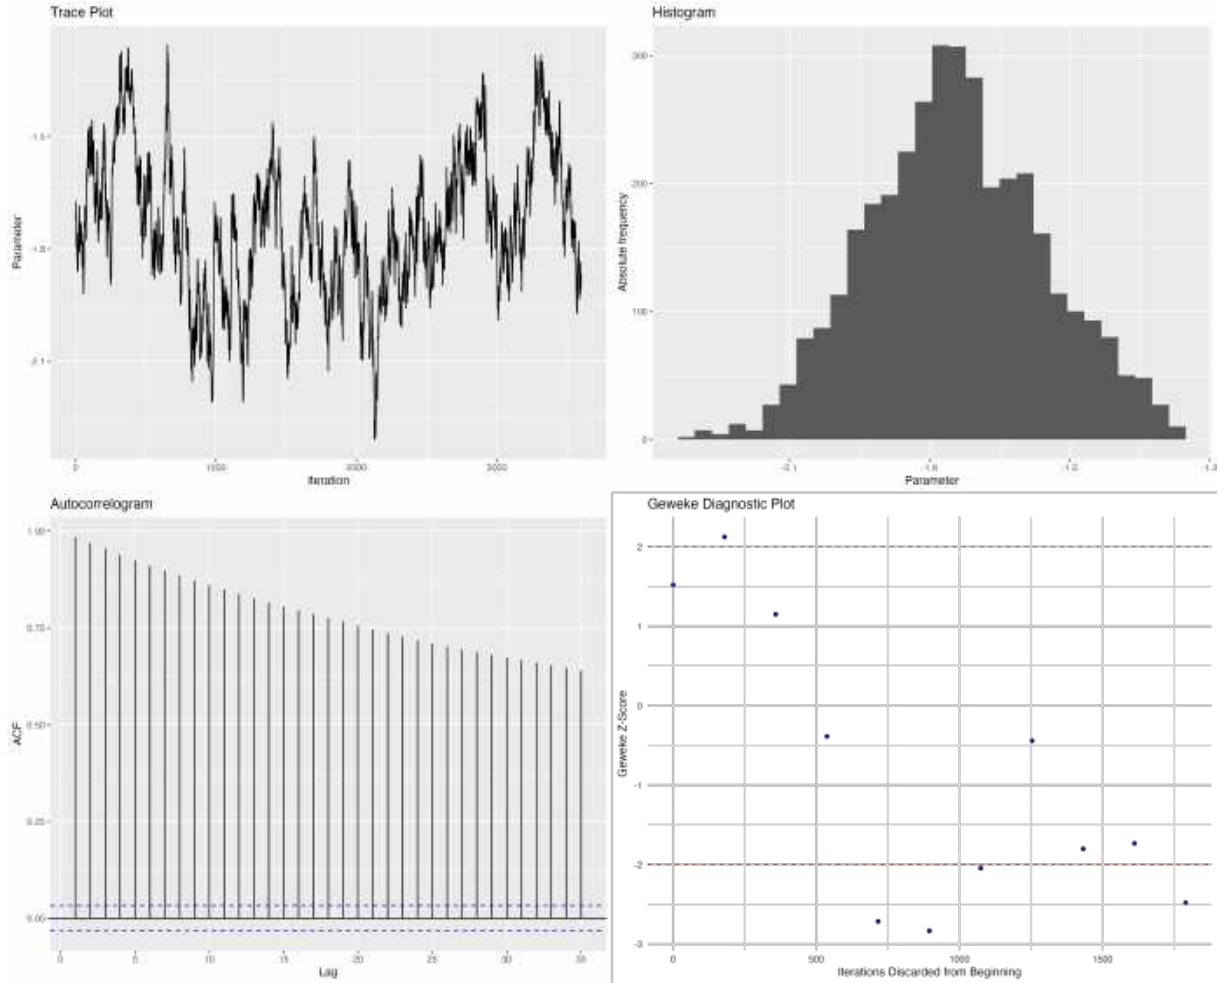

Figure S19: Convergence diagnostic plots for the parameter  $\log(\sigma^2)$  in the district of Mecnhelas. The panels display: trace plot (top-left), histogram (top-right), autocorrelation plot (bottom-left), and running Geweke plot (bottom-right).

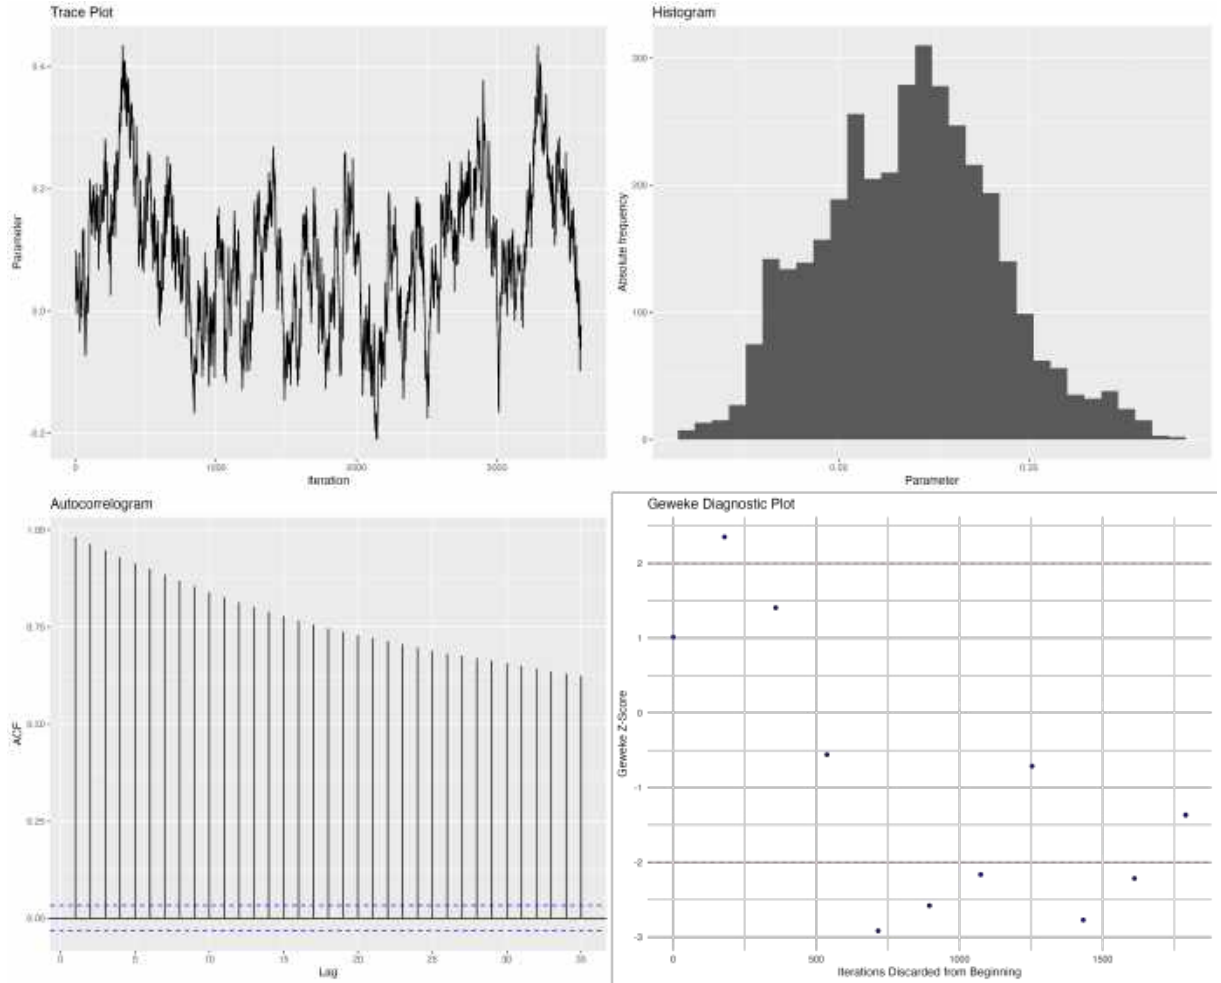

Figure S20: Convergence diagnostic plots for the parameter  $\log(\phi)$  in the district of Mecan-helas. The panels display: trace plot (top-left), histogram (top-right), autocorrelogram (bottom-left), and running Geweke plot (bottom-right).

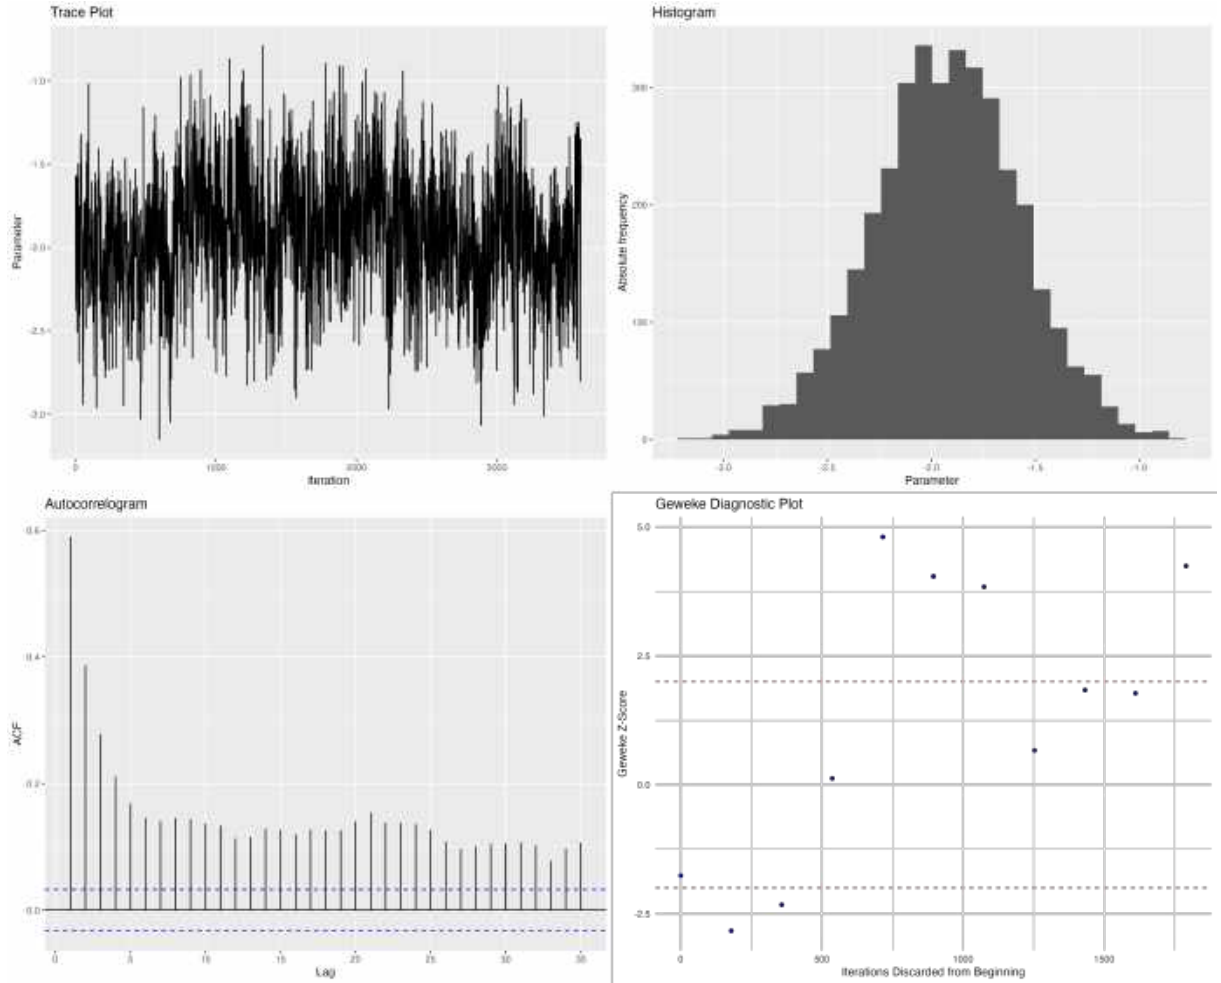

Figure S21: Convergence diagnostic plots for the parameter  $\log(\nu^2)$  in the district of Mecnhehas. The panels display: trace plot (top-left), histogram (top-right), autocorrellogram (bottom-left), and running Geweke plot (bottom-right).

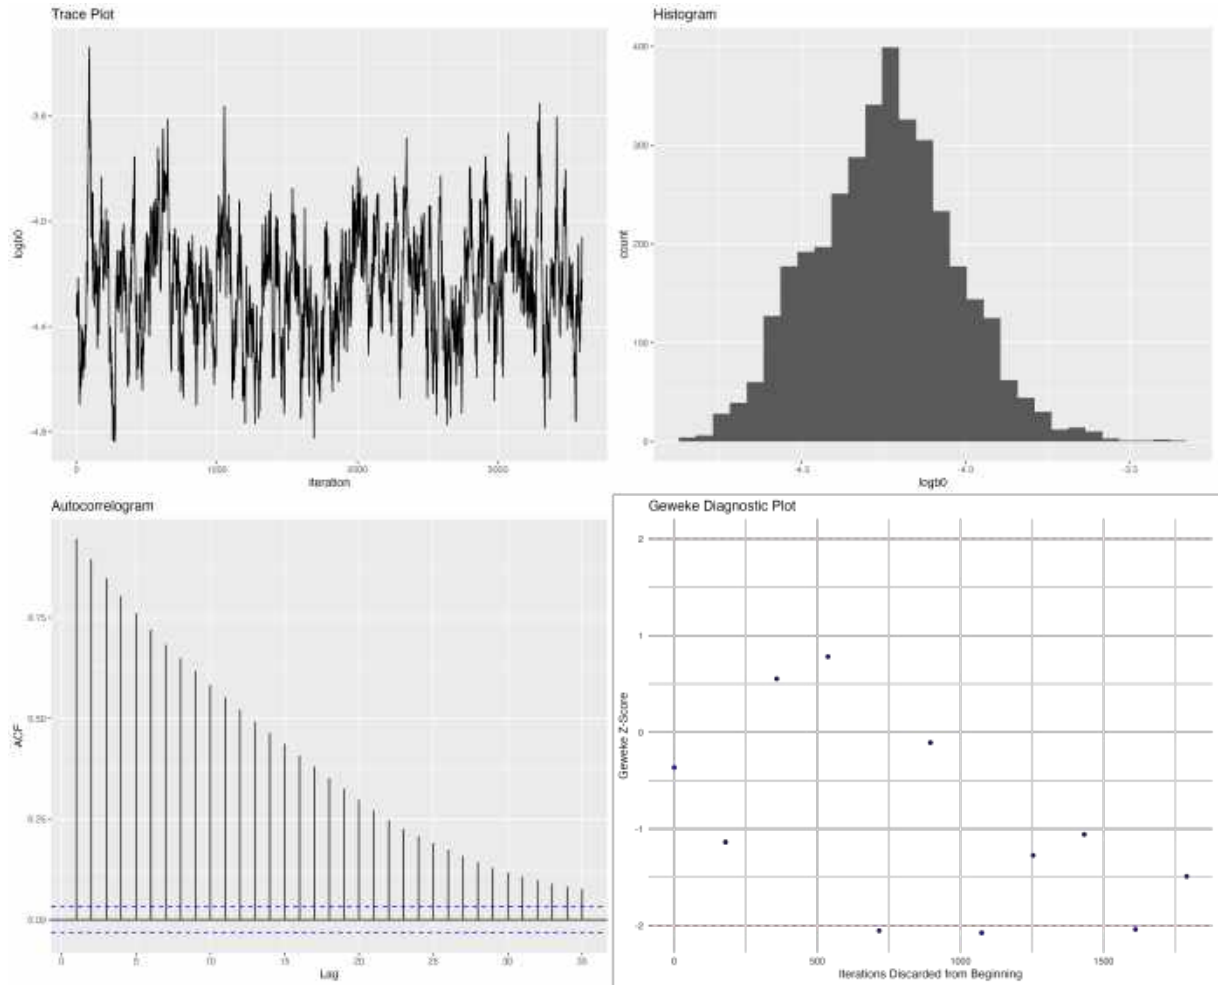

Figure S22: Convergence diagnostic plots for the parameter  $\log(\beta_0)$  in the district of Mecnhelas. The panels display: trace plot (top-left), histogram (top-right), autocorrelogram (bottom-left), and running Geweke plot (bottom-right).

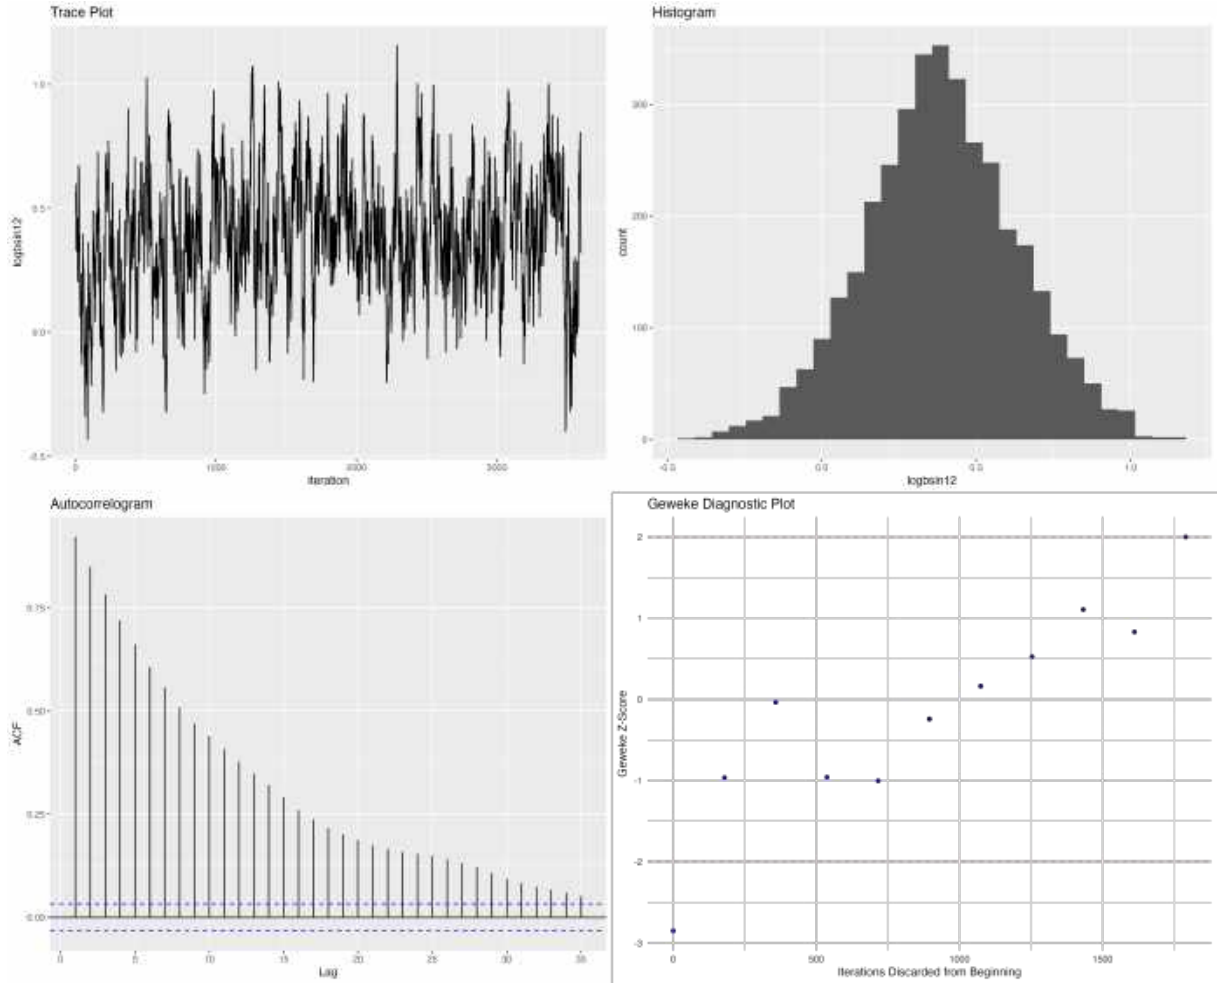

Figure S23: Convergence diagnostic plots for the parameter  $\log(\beta_1)$  in the district of Mecnhelas. The panels display: trace plot (top-left), histogram (top-right), autocorrelation plot (bottom-left), and running Geweke plot (bottom-right).

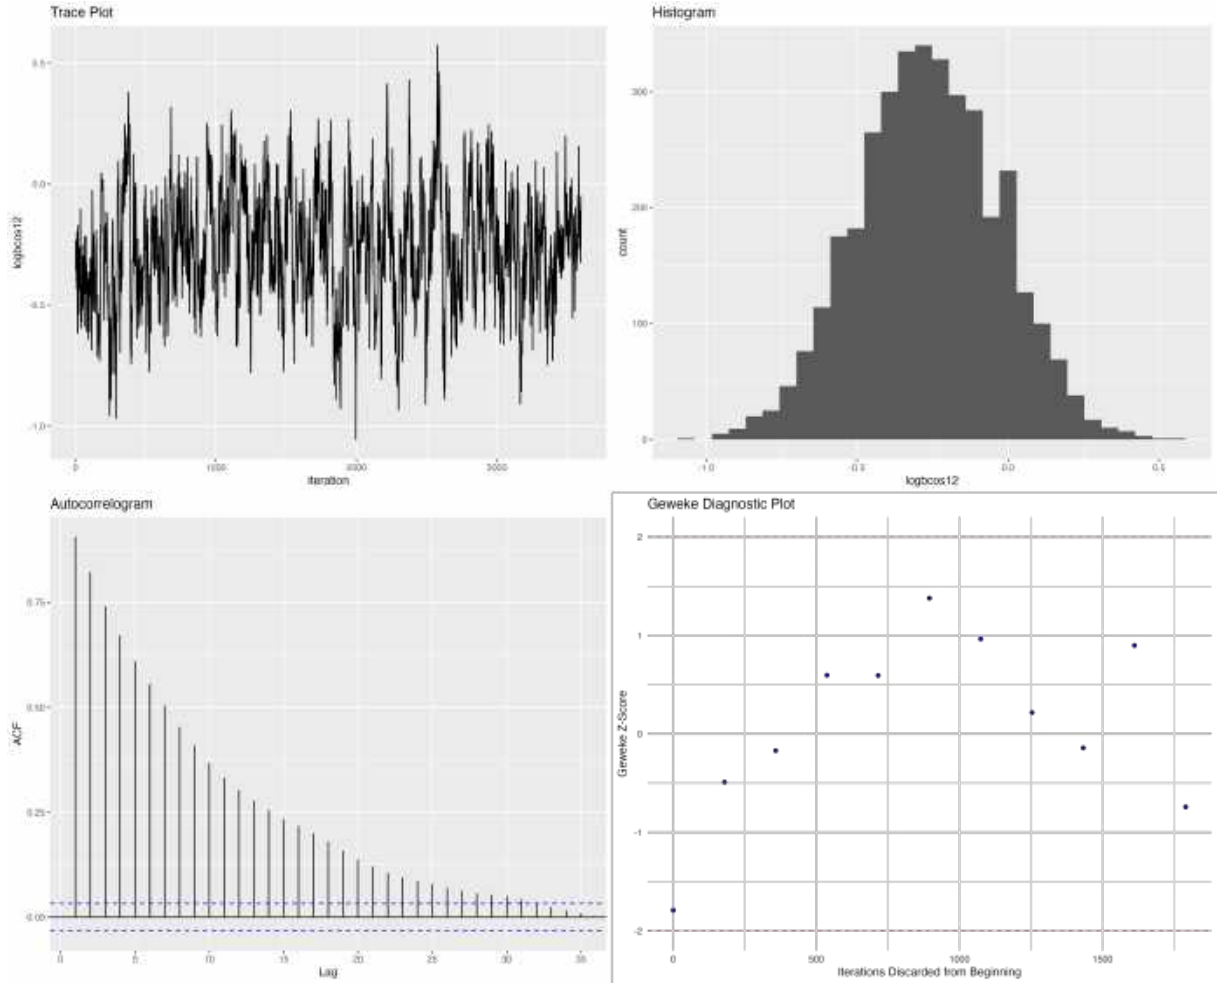

Figure S24: Convergence diagnostic plots for the parameter  $\log(\beta_2)$  in the district of Mecnhelas. The panels display: trace plot (top-left), histogram (top-right), autocorrellogram (bottom-left), and running Geweke plot (bottom-right).

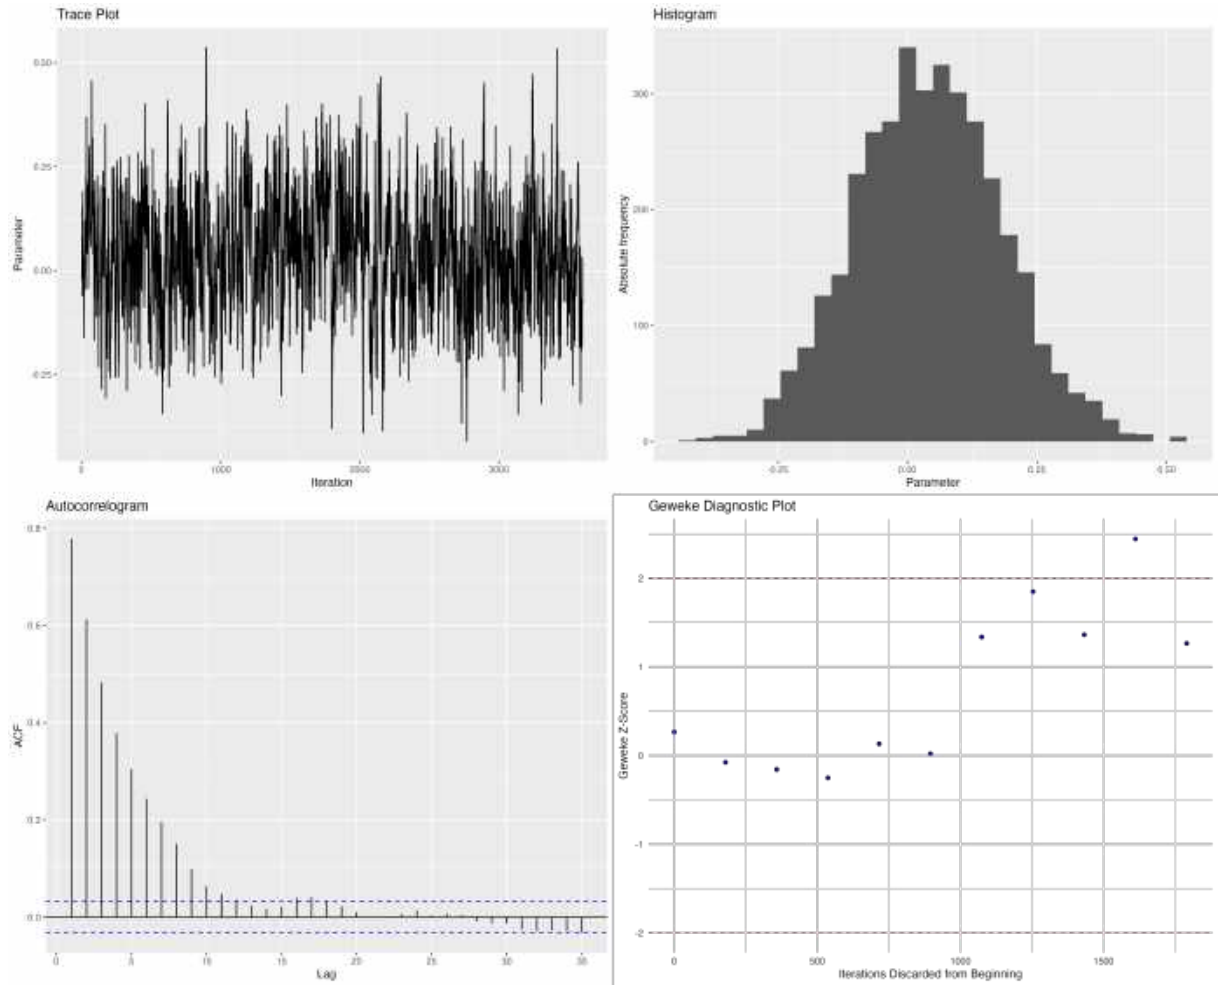

Figure S25: Convergence diagnostic plots for the parameter  $\log(\beta_3)$  in the district of Mecnhelas. The panels display: trace plot (top-left), histogram (top-right), autocorrelogram (bottom-left), and running Geweke plot (bottom-right).

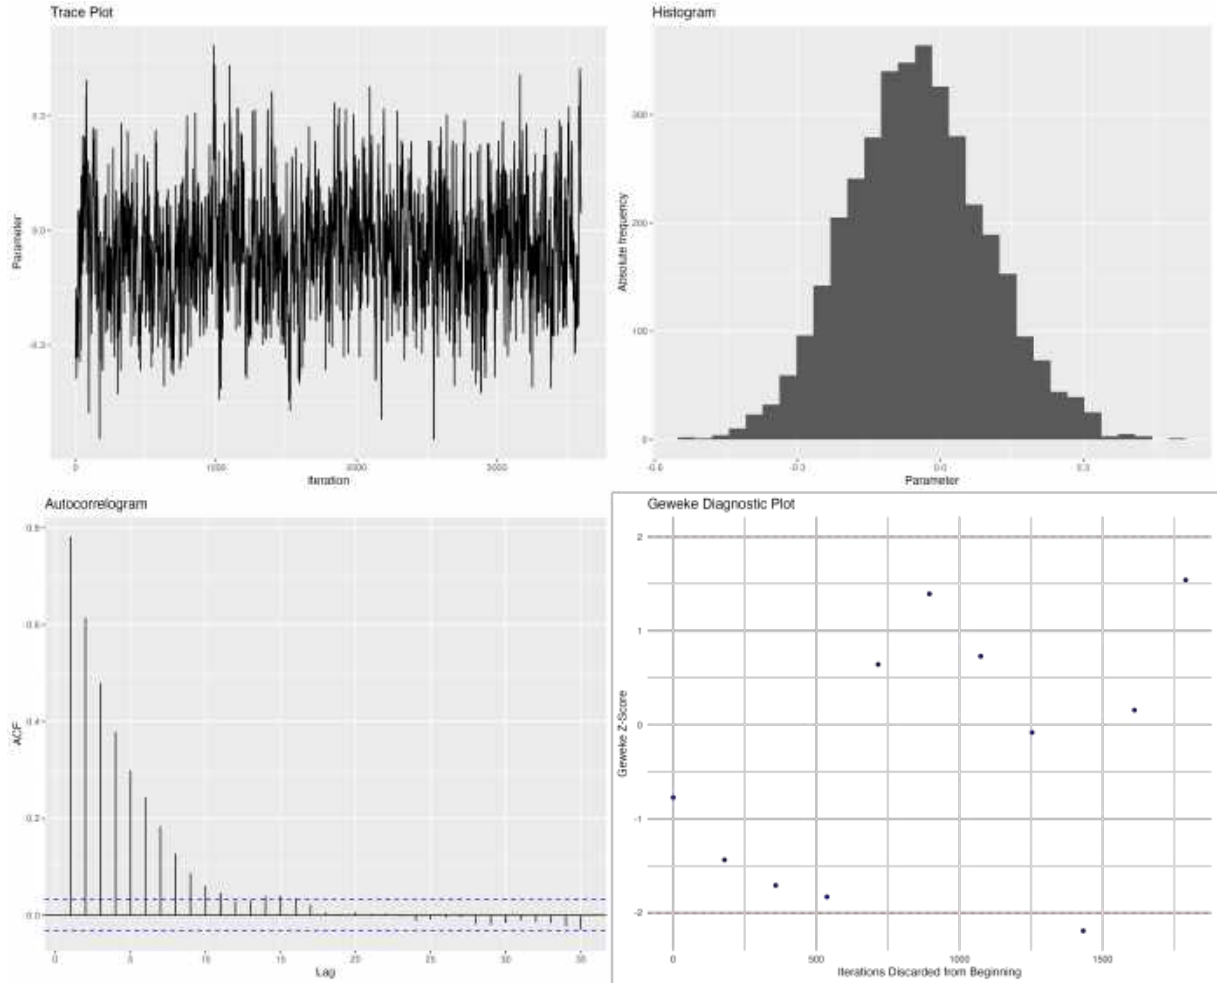

Figure S26: Convergence diagnostic plots for the parameter  $\log(\beta_4)$  in the district of Mecnhelas. The panels display: trace plot (top-left), histogram (top-right), autocorrelation plot (bottom-left), and running Geweke plot (bottom-right).



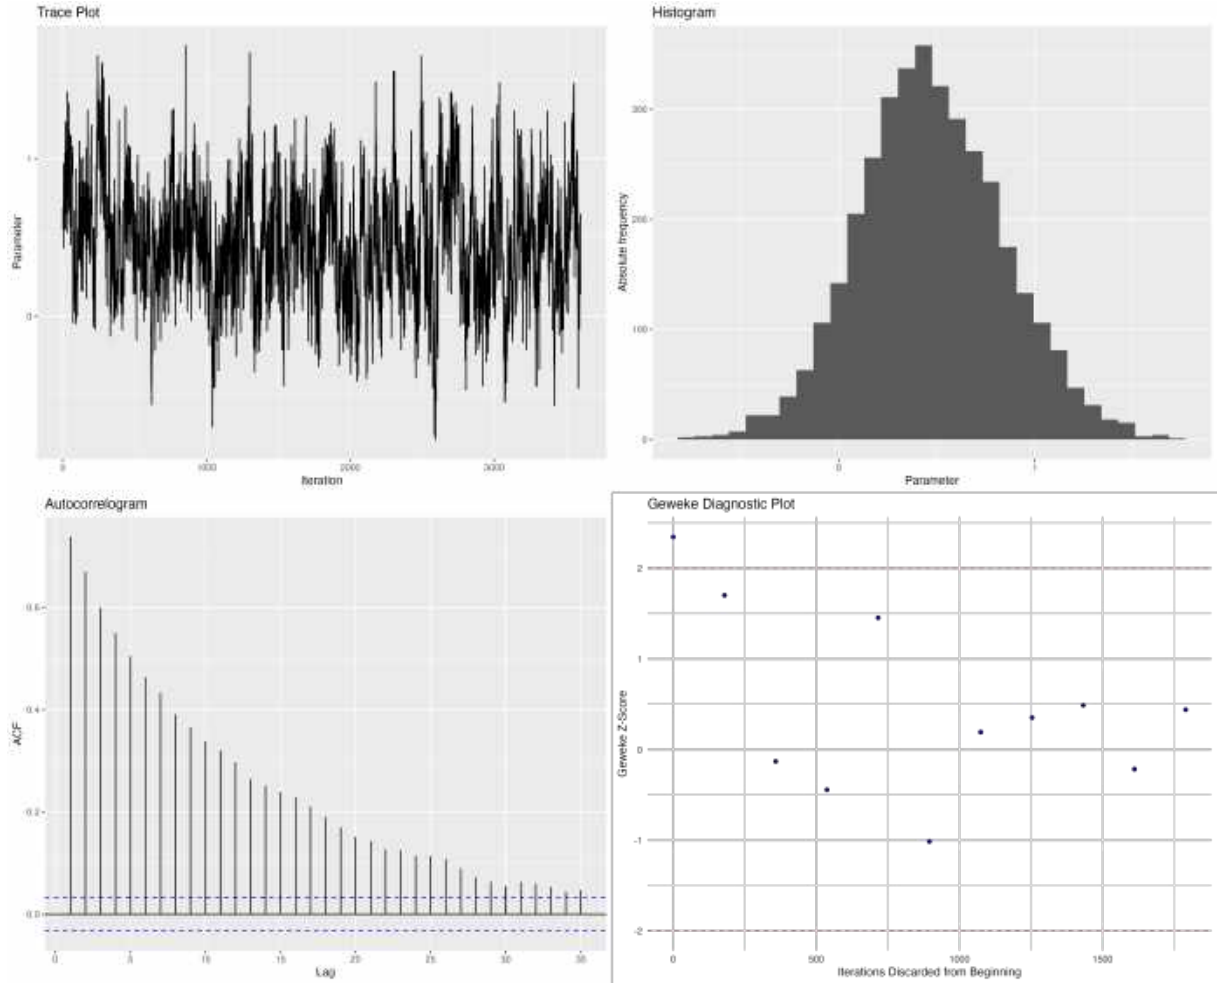

Figure S27: Convergence diagnostic plots for the parameter  $S_{11}$  in the district of Mecan-helas. The panels display: trace plot (top-left), histogram (top-right), autocorrelogram (bottom-left), and running Geweke plot (bottom-right).

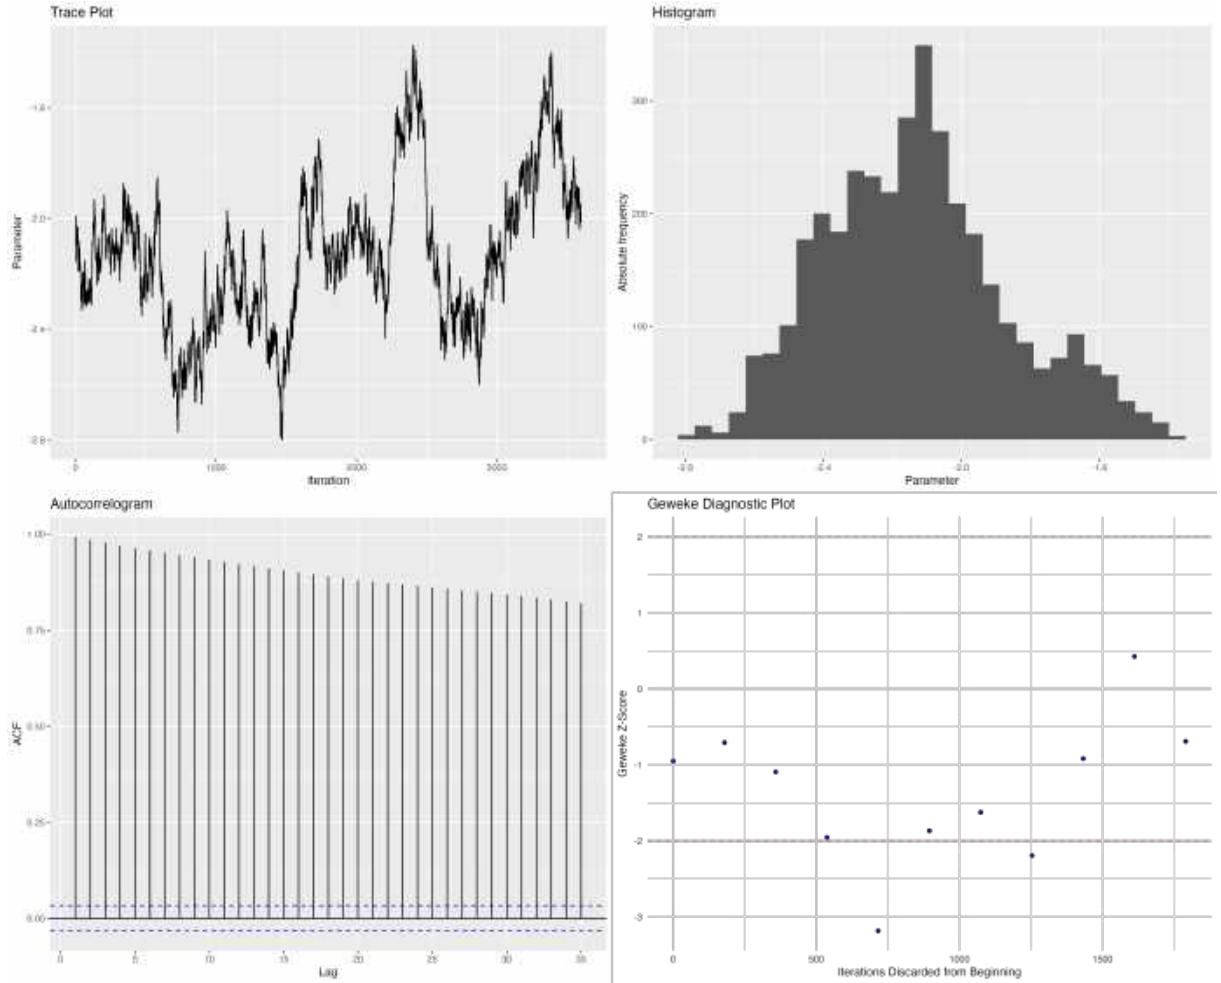

Figure S28: Convergence diagnostic plots for the parameter  $\log(\sigma^2)$  in the district of Sanga. The panels display: trace plot (top-left), histogram (top-right), autocorrelogram (bottom-left), and running Geweke plot (bottom-right).

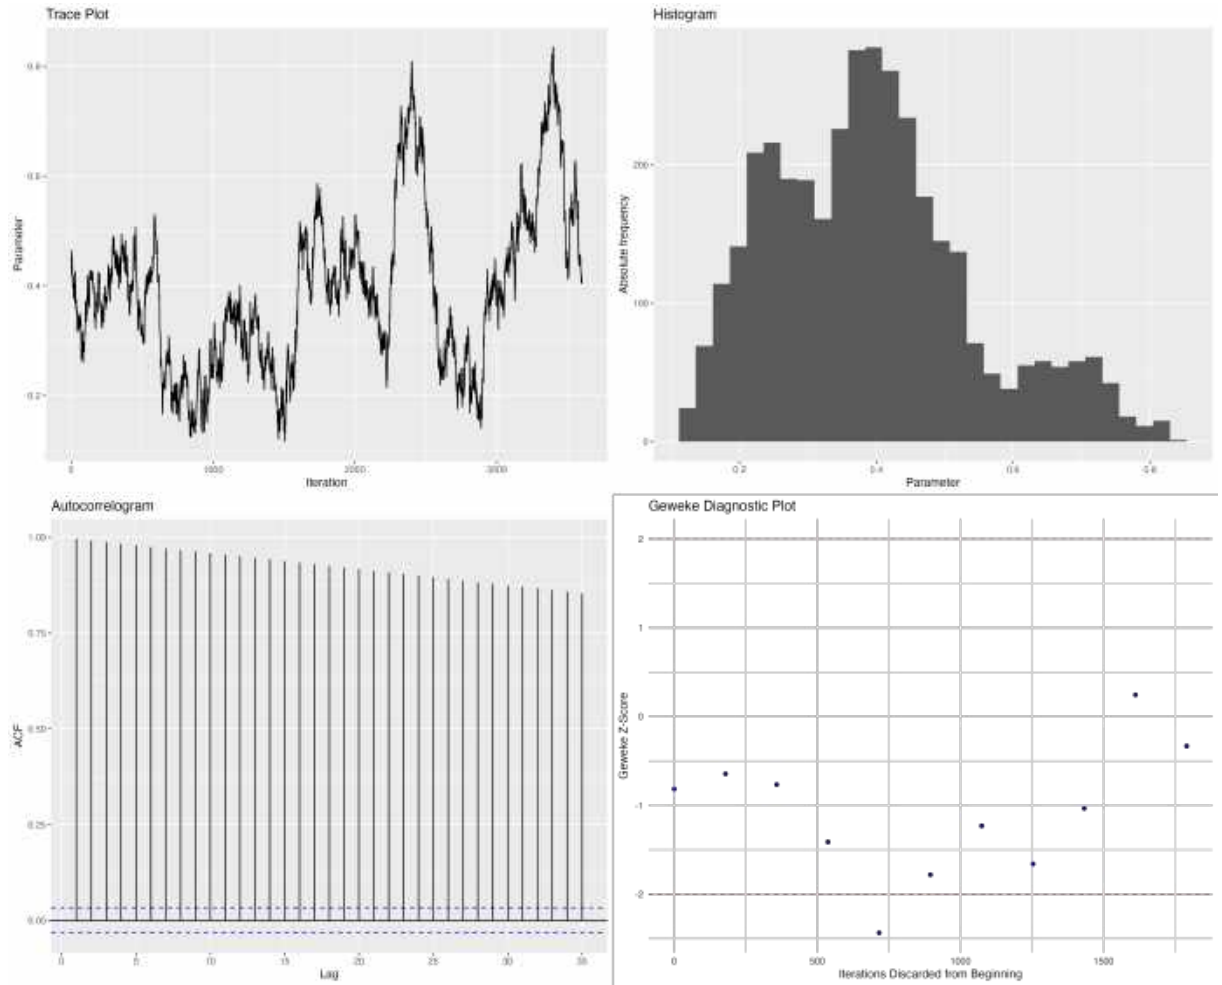

Figure S29: Convergence diagnostic plots for the parameter  $\log(\phi)$  in the district of Sanga. The panels display: trace plot (top-left), histogram (top-right), autocorrelogram (bottom-left), and running Geweke plot (bottom-right).

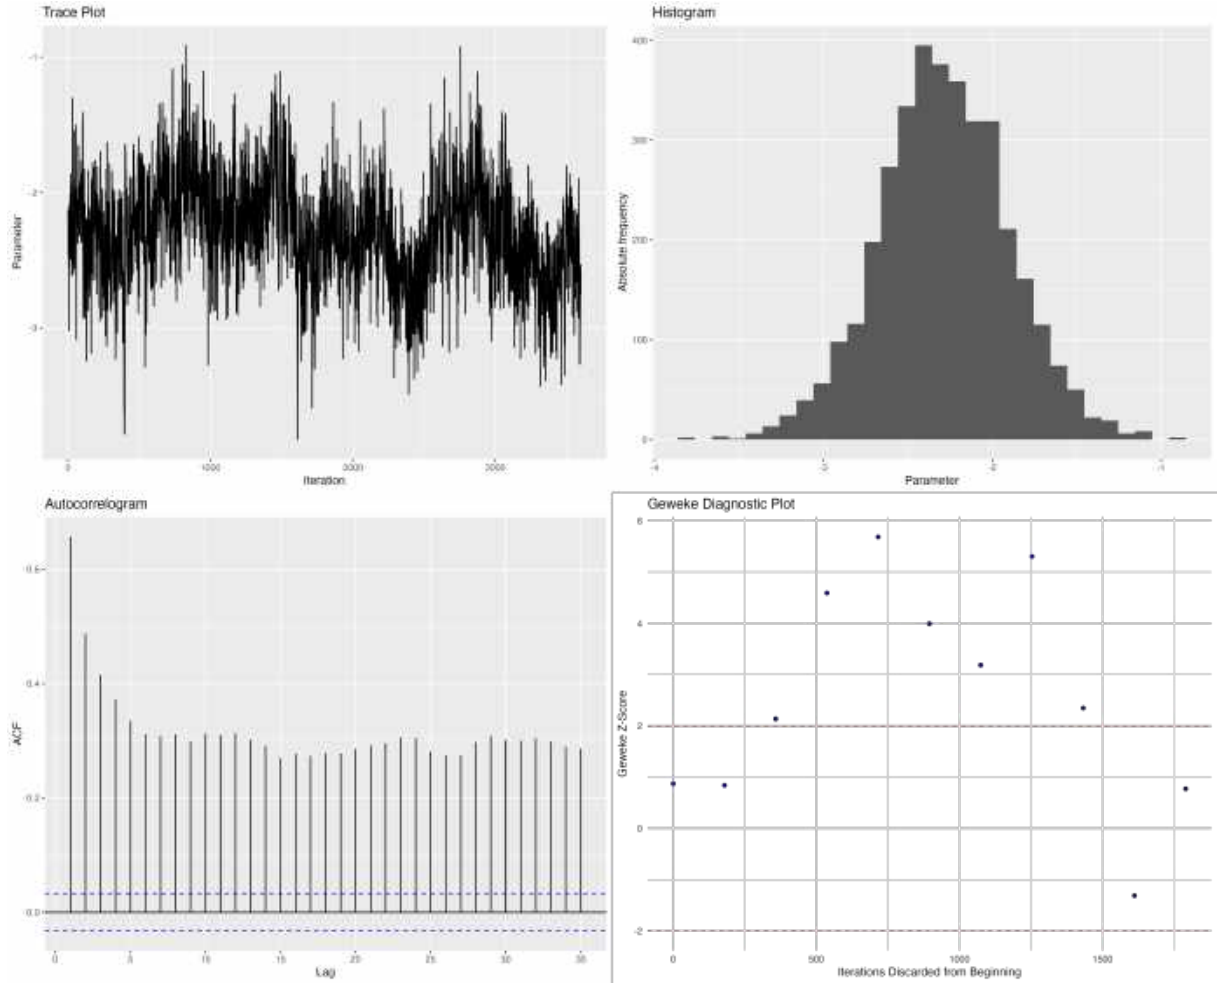

Figure S30: Convergence diagnostic plots for the parameter  $\log(\nu^2)$  in the district of Sanga. The panels display: trace plot (top-left), histogram (top-right), autocorrelogram (bottom-left), and running Geweke plot (bottom-right).

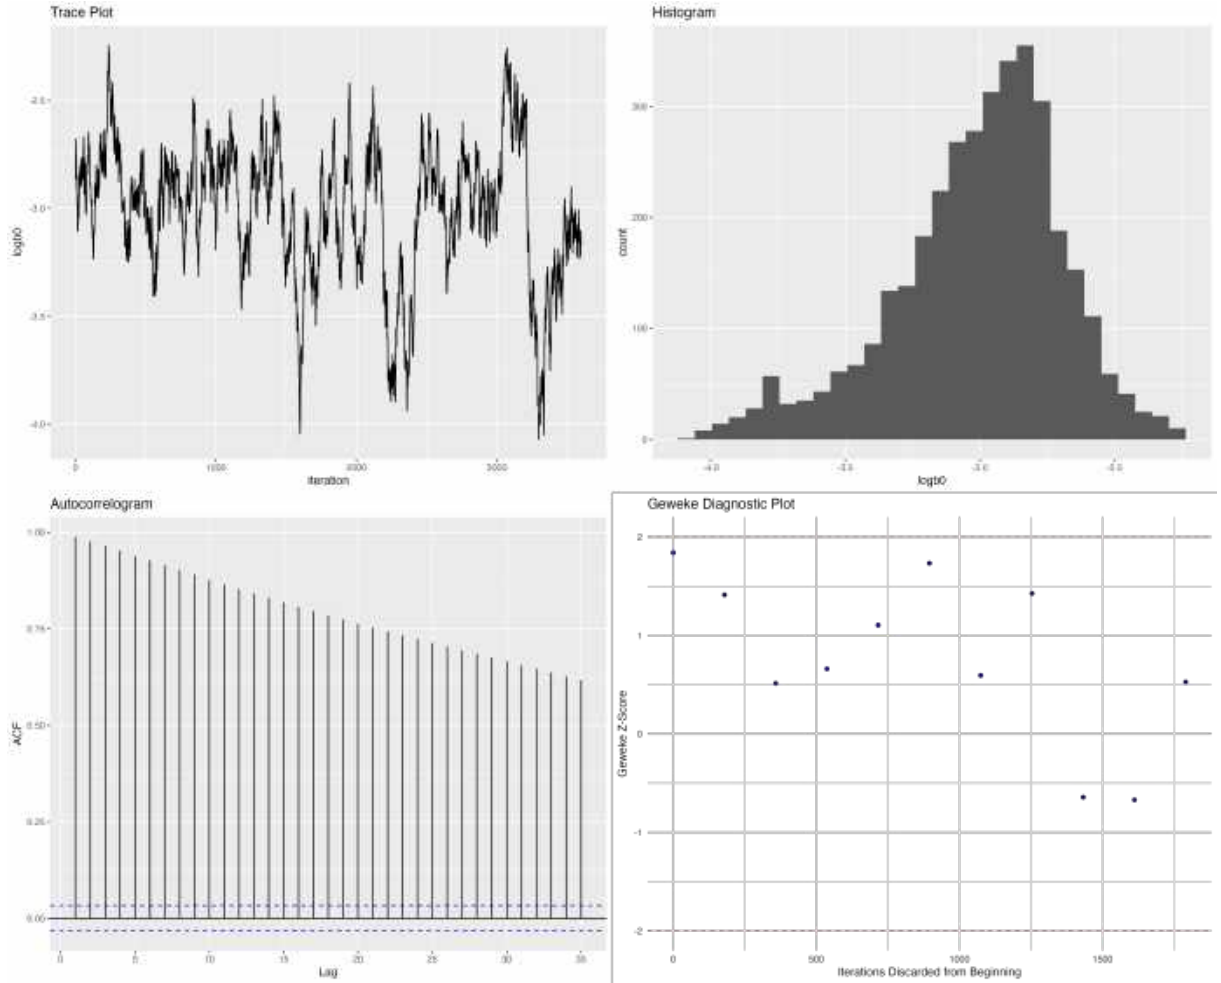

Figure S31: Convergence diagnostic plots for the parameter  $\log(\beta_0)$  in the district of Sanga. The panels display: trace plot (top-left), histogram (top-right), autocorrelogram (bottom-left), and running Geweke plot (bottom-right).

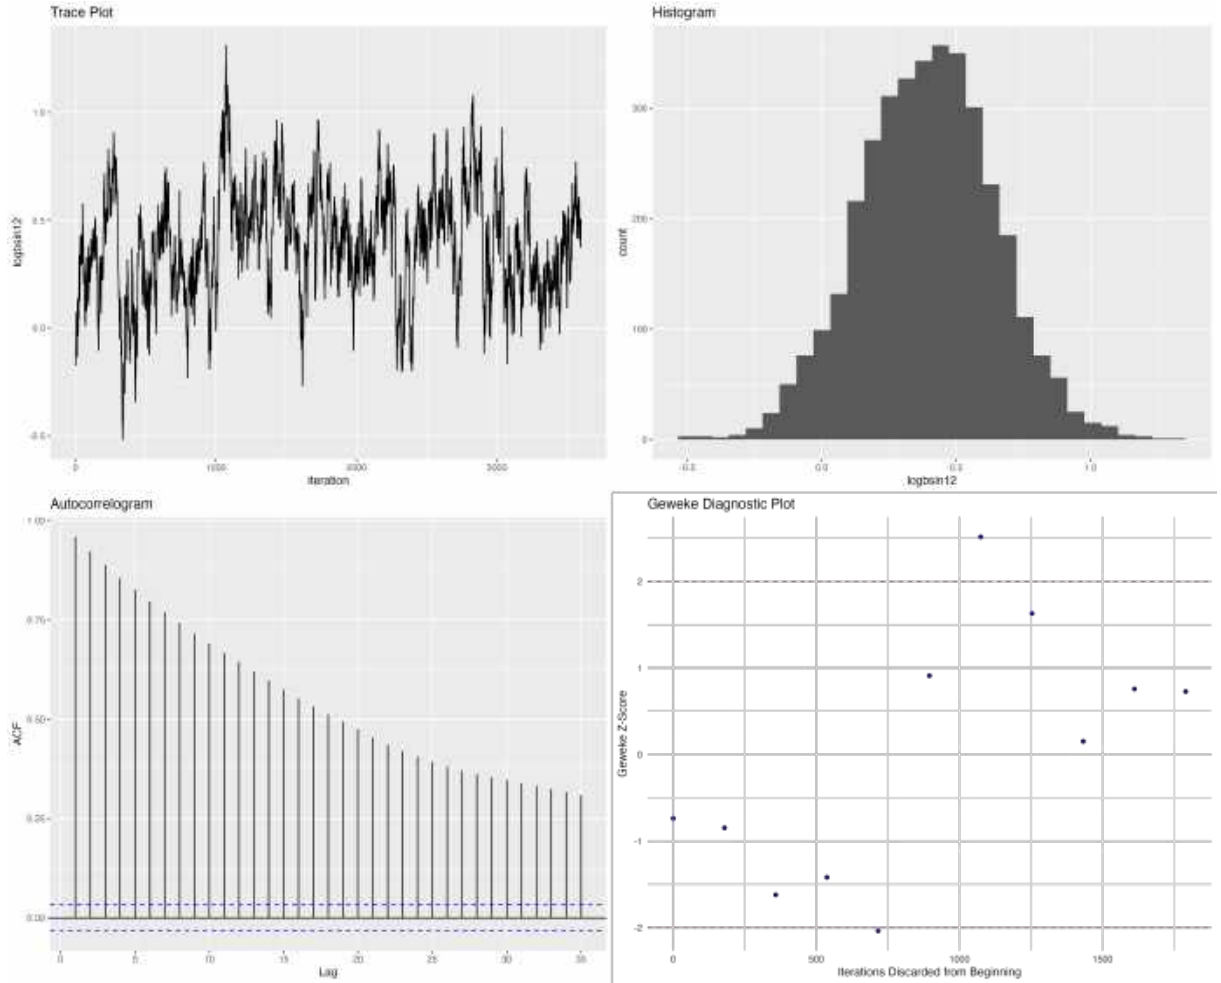

Figure S32: Convergence diagnostic plots for the parameter  $\log(\beta_1)$  in the district of Sanga. The panels display: trace plot (top-left), histogram (top-right), autocorrelogram (bottom-left), and running Geweke plot (bottom-right).

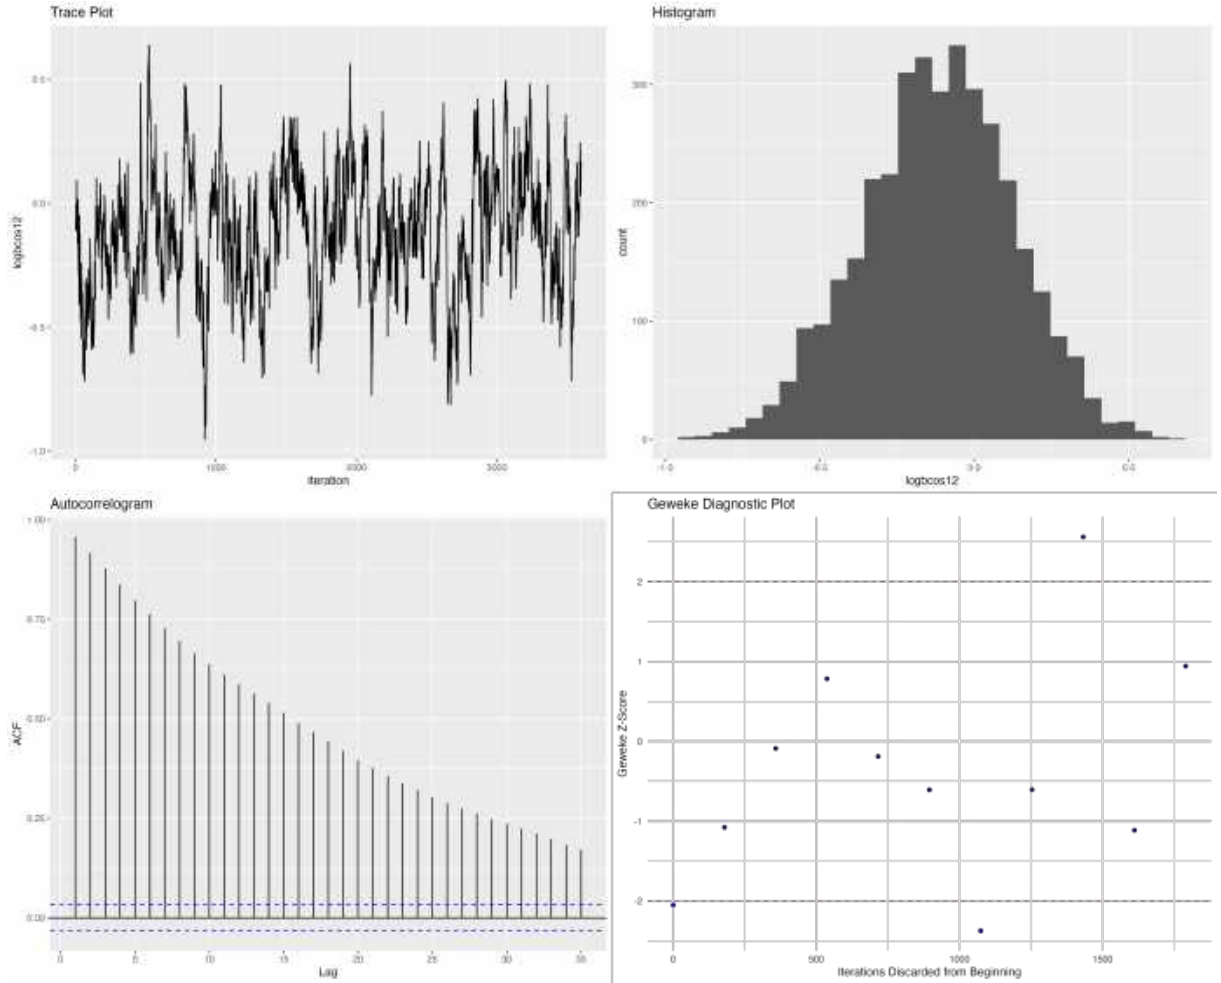

Figure S33: Convergence diagnostic plots for the parameter  $\log(\beta_2)$  in the district of Sanga. The panels display: trace plot (top-left), histogram (top-right), autocorrelogram (bottom-left), and running Geweke plot (bottom-right).

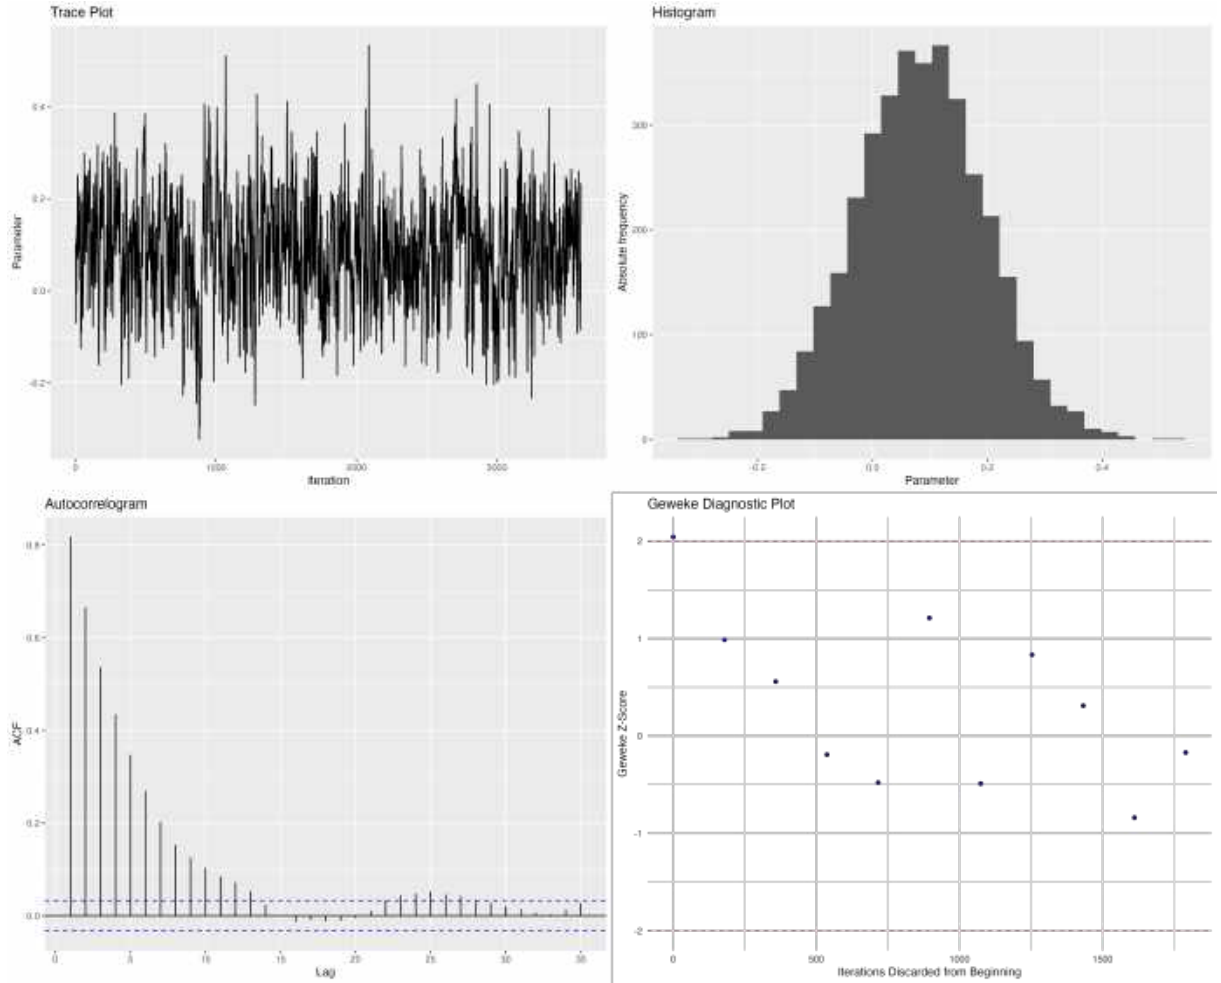

Figure S34: Convergence diagnostic plots for the parameter  $\log(\beta_3)$  in the district of Sanga. The panels display: trace plot (top-left), histogram (top-right), autocorrelogram (bottom-left), and running Geweke plot (bottom-right).



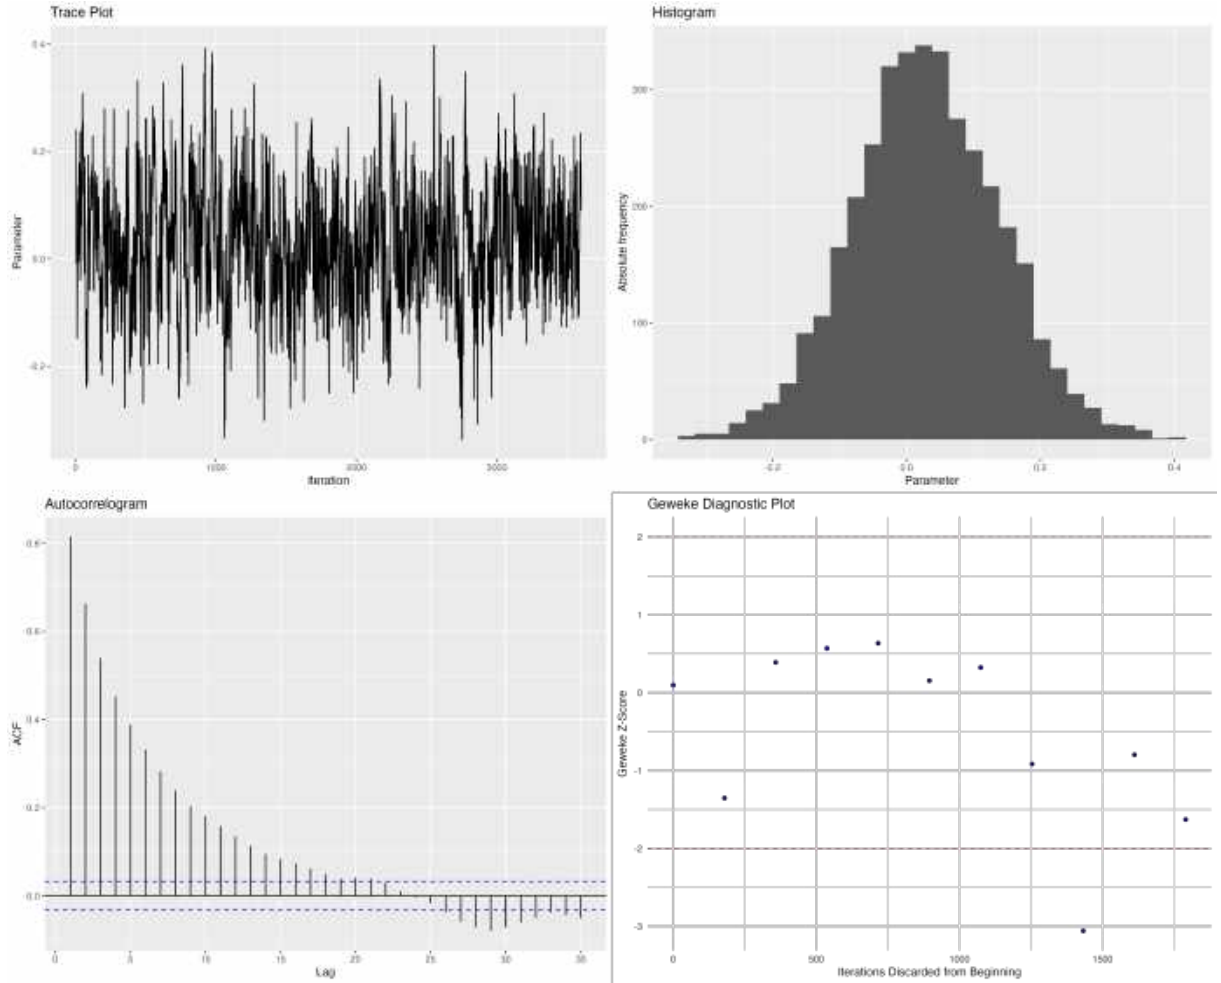

Figure S35: Convergence diagnostic plots for the parameter  $\log(\beta_4)$  in the district of Sanga. The panels display: trace plot (top-left), histogram (top-right), autocorrelogram (bottom-left), and running Geweke plot (bottom-right).

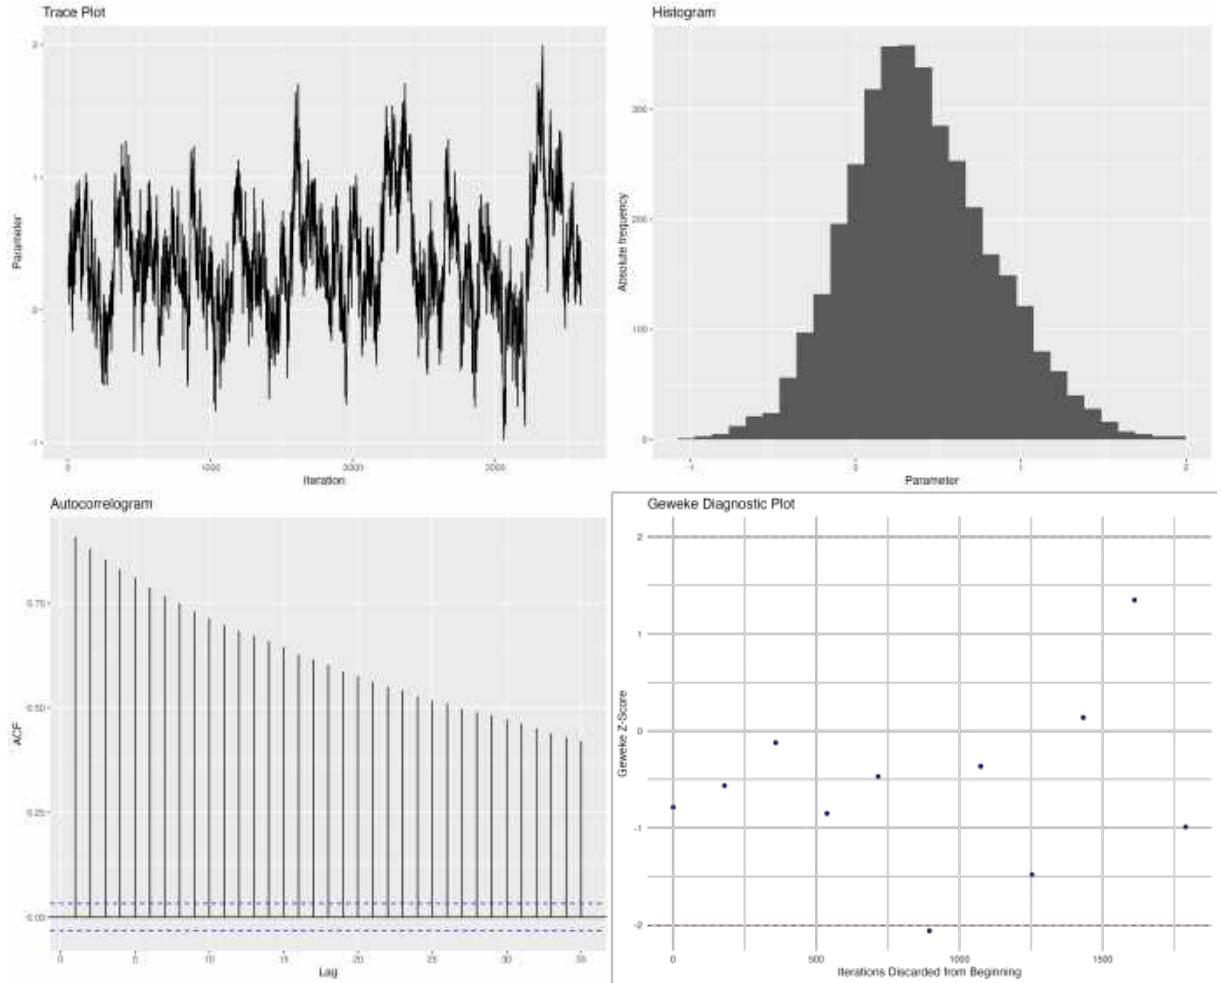

Figure S36: Convergence diagnostic plots for the parameter  $S_{11}$  in the district of Sanga. The panels display: trace plot (top-left), histogram (top-right), autocorrelogram (bottom-left), and running Geweke plot (bottom-right).

## 2.2 Malaria incidence in Niassa, Mozambique - Model comparison

Figure S37 and S38 compare the performance of the models in the training and test set using the Root Mean Squared Error (RMSE) and the Mean Absolute Error (MAE) respectively.

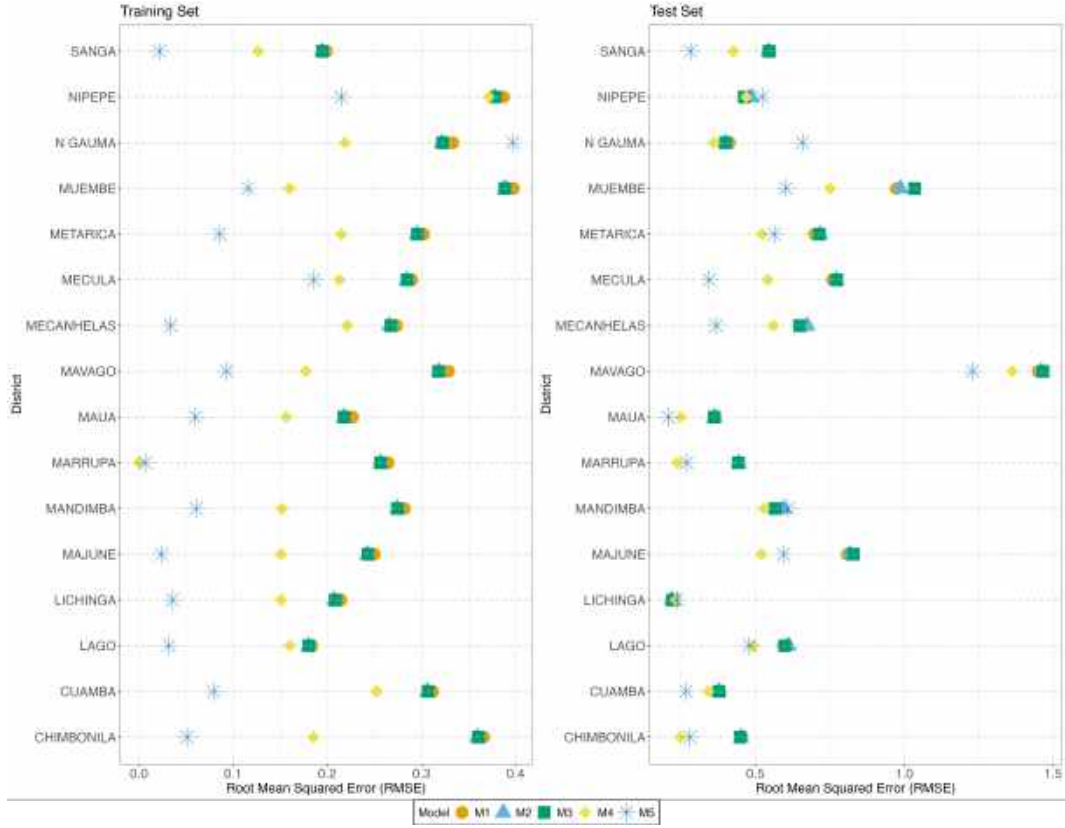

Figure S37: Comparison of model performance on the **training set** and **test set** for malaria incidence in Niassa, Mozambique, using the Root Mean Squared Error.

Figure S39 displays the district-level distribution of CRPS values for the districts of Lichinga and Chimbonila.

Figure S40 displays the district-level distribution of CRPS values for the districts of Mavago and Metarica.

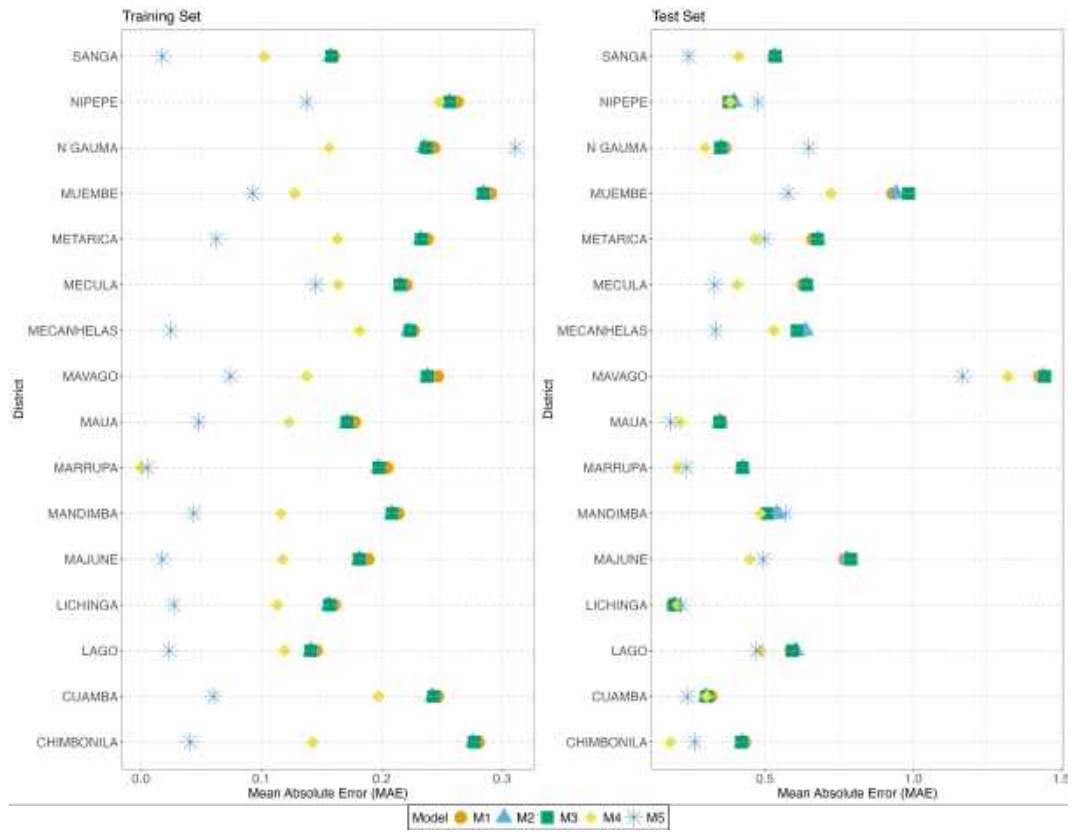

Figure S38: Comparison of model performance on the **training set** and **test set** for malaria incidence in Niassa, Mozambique, using the Mean Absolute Error.

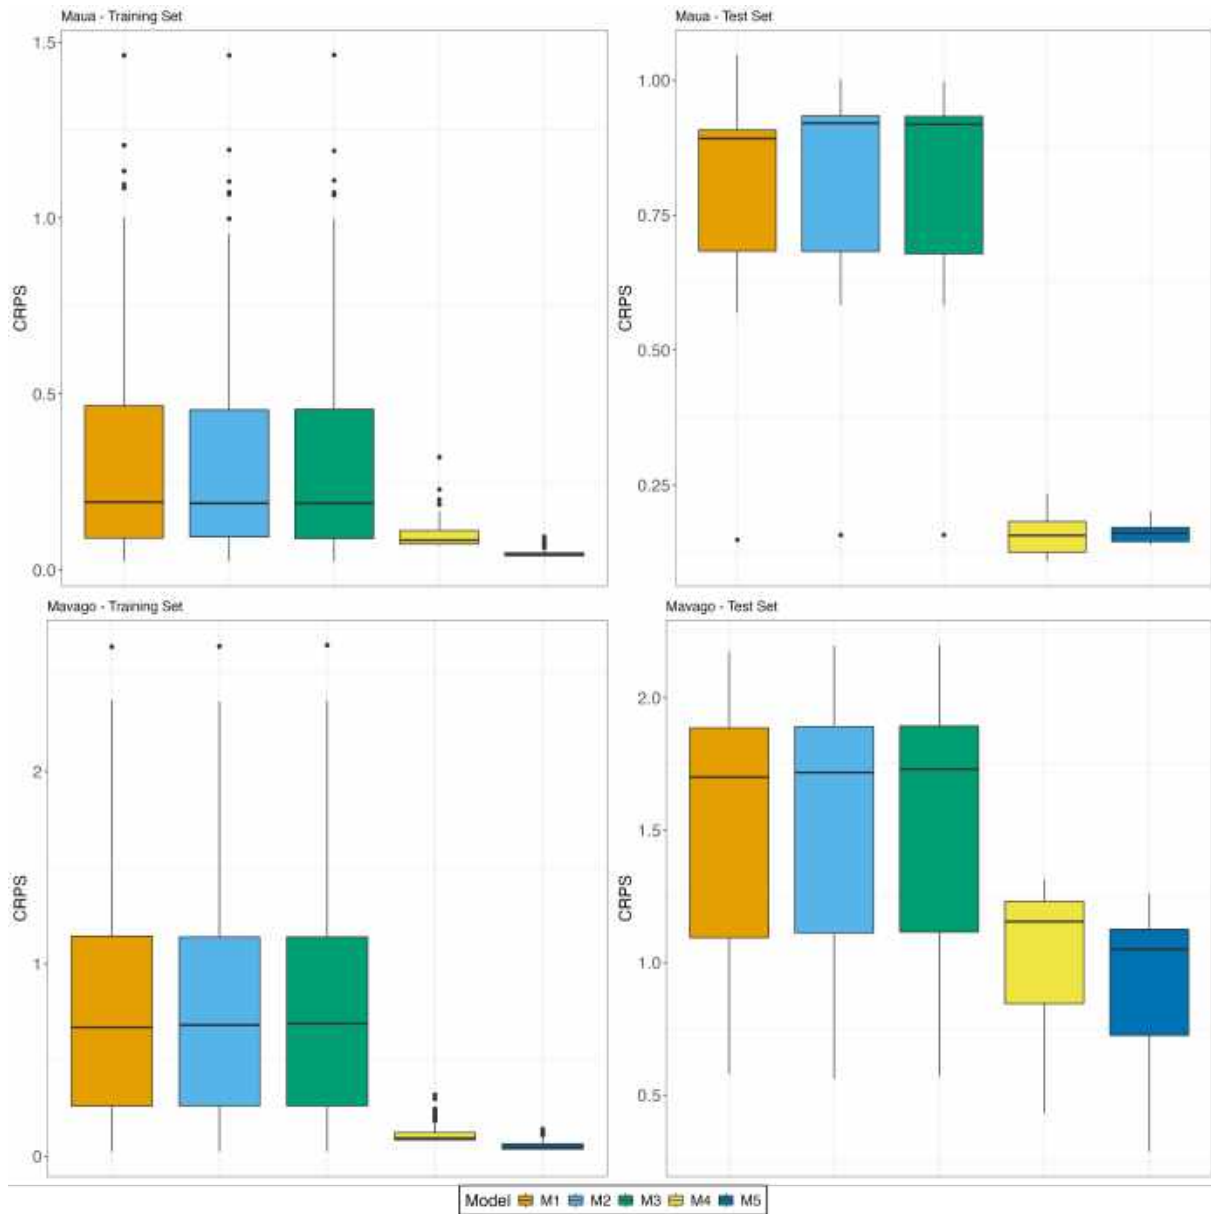

Figure S39: District distribution of the Continuous Ranked Probability Score (CRPS) for the malaria incidence example. Results are shown for the training set (**left panels**) and the test set (**right panels**), specifically the districts of Lichinga (**top panels**) and Chimbonila (**bottom panels**) in Niassa, Mozambique.

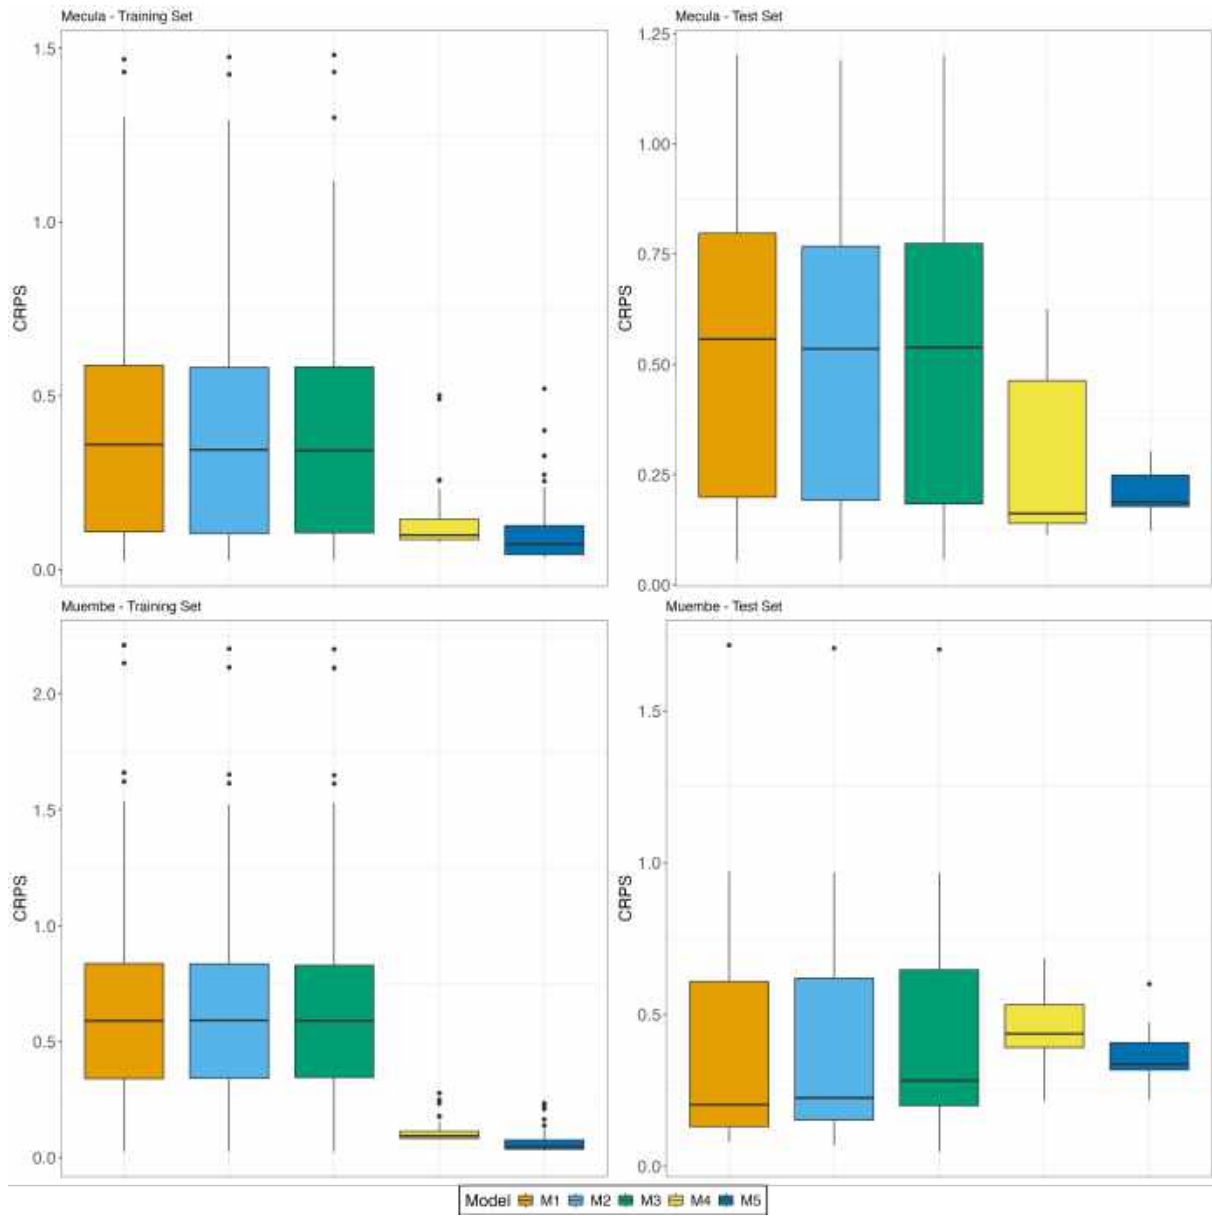

Figure S40: District distribution of the Continuous Ranked Probability Score for the malaria incidence example. Results are shown for the training set (**left panels**) and the test set (**right panels**), specifically the districts of Mavago (**top panels**) and Metarica (**bottom panels**) in Niassa, Mozambique.

### 2.3 Food security in Cameroon - Results by region

Figures S41, S42, S43, S44, S45, S46, S47 present the convergence diagnostic plots for Adamaoua. These diagnostics include the trace plot, histogram, autocorrelogram, and running Geweke plot.

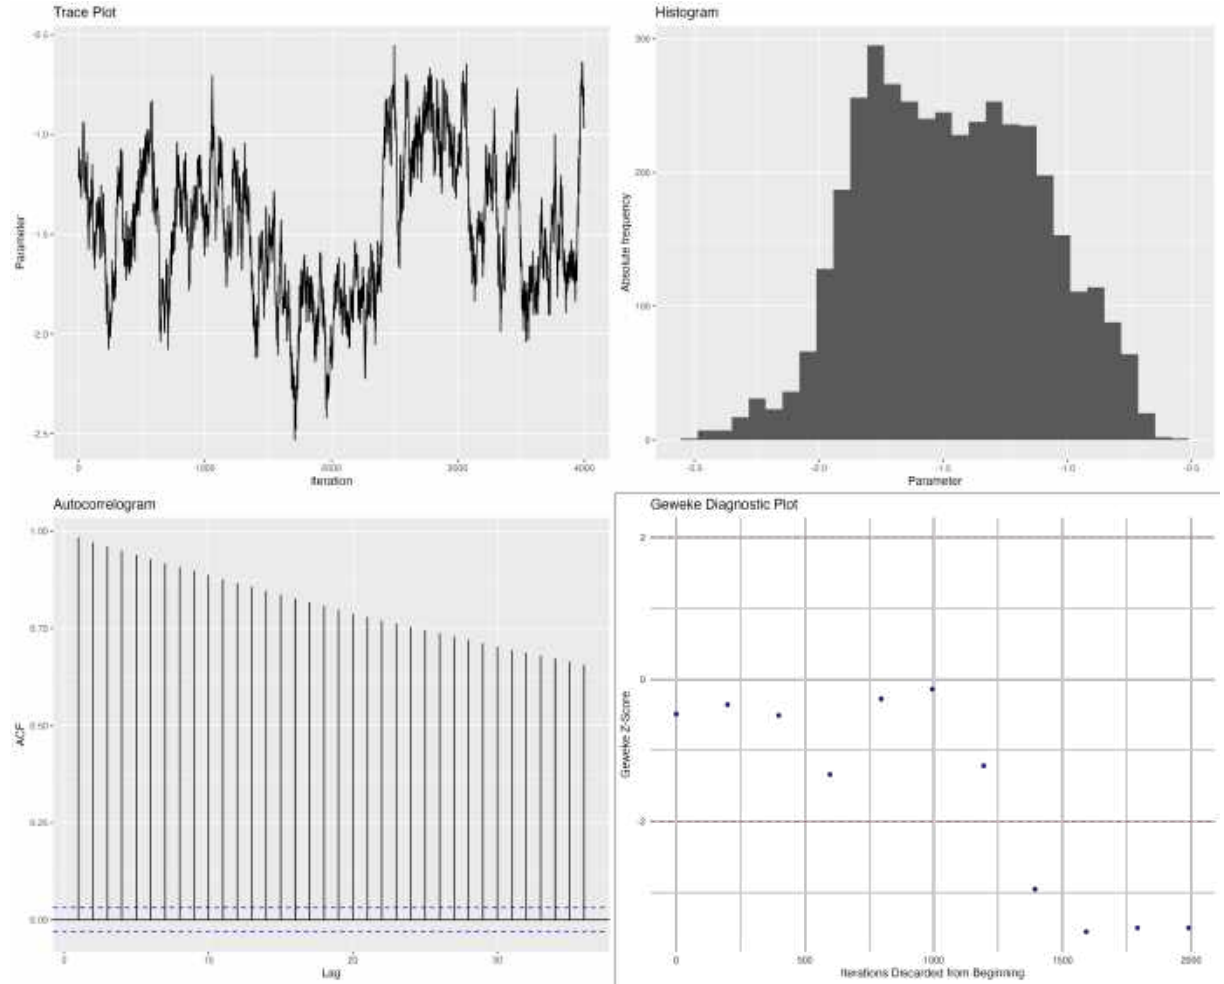

Figure S41: Convergence diagnostic plots for the parameter  $\log(\sigma^2)$  in the district of Adamaoua.

Similarly, Figures S48, S49, S50, S51, S52, S53, S54 show the convergence diagnostics for Nord.

Figures S55, S56, S57, S58, S59, S60, S61 correspond to Nord-Ouest.

Figures S62, S63, S64, S65, S66, S67, S68 correspond to Sud.

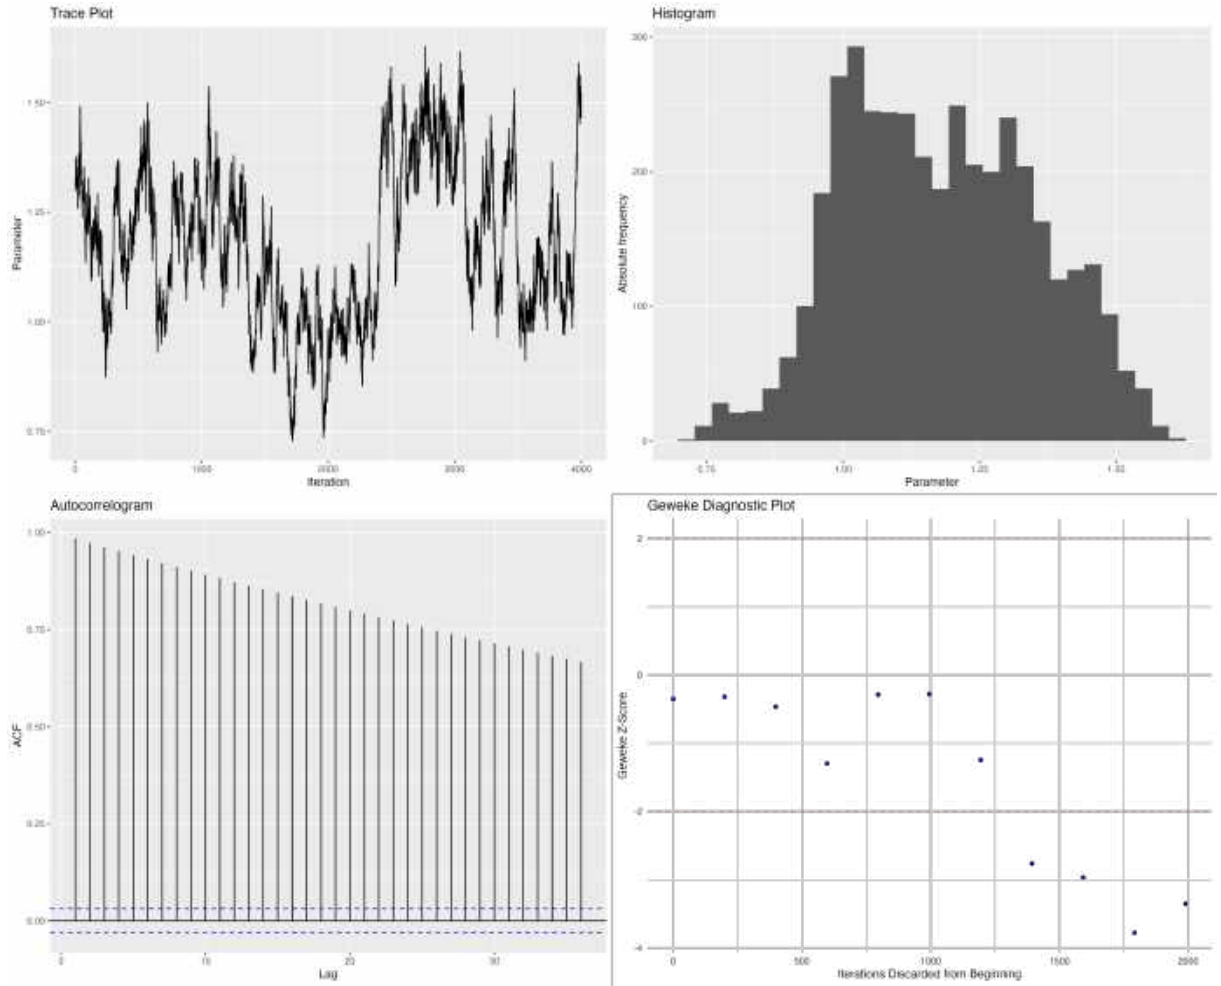

Figure S42: Convergence diagnostic plots for the parameter  $\log(\phi)$  in the district of Adamaoua.



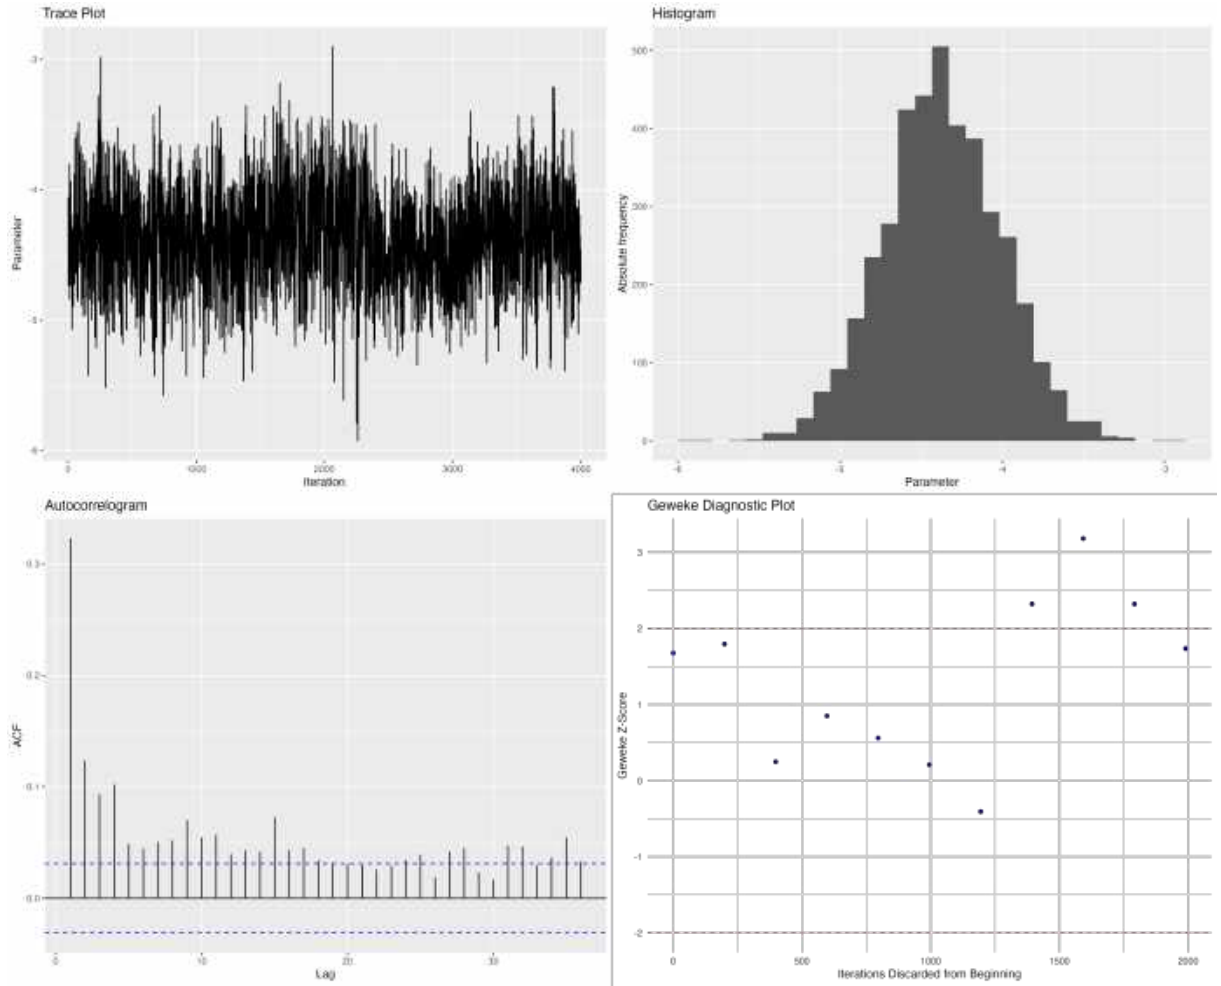

Figure S43: Convergence diagnostic plots for the parameter  $\log(\nu^2)$  in the district of Adamaoua.

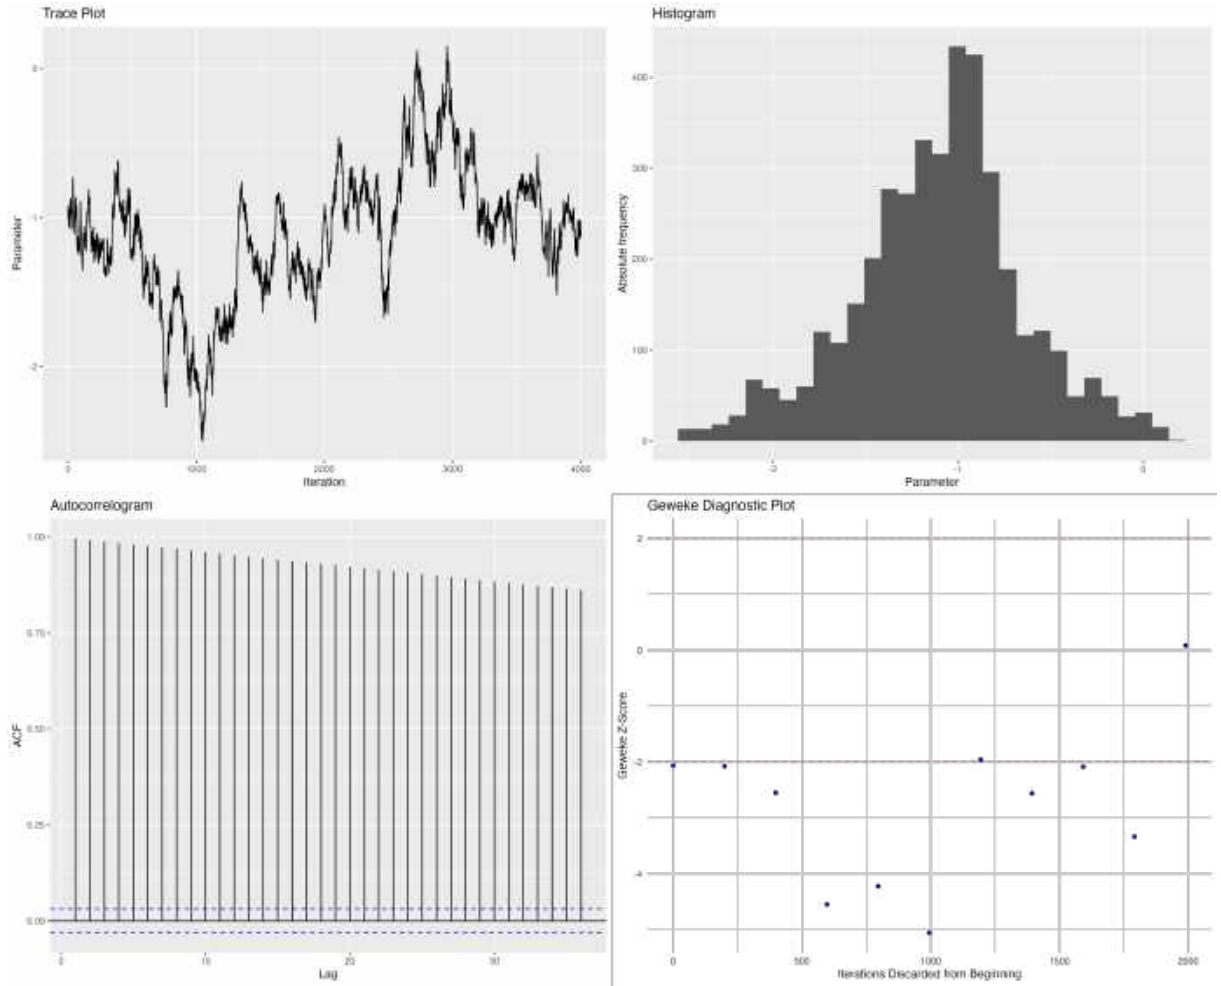

Figure S44: Convergence diagnostic plots for the parameter  $\log(\beta_0)$  in the district of Adamaoua.

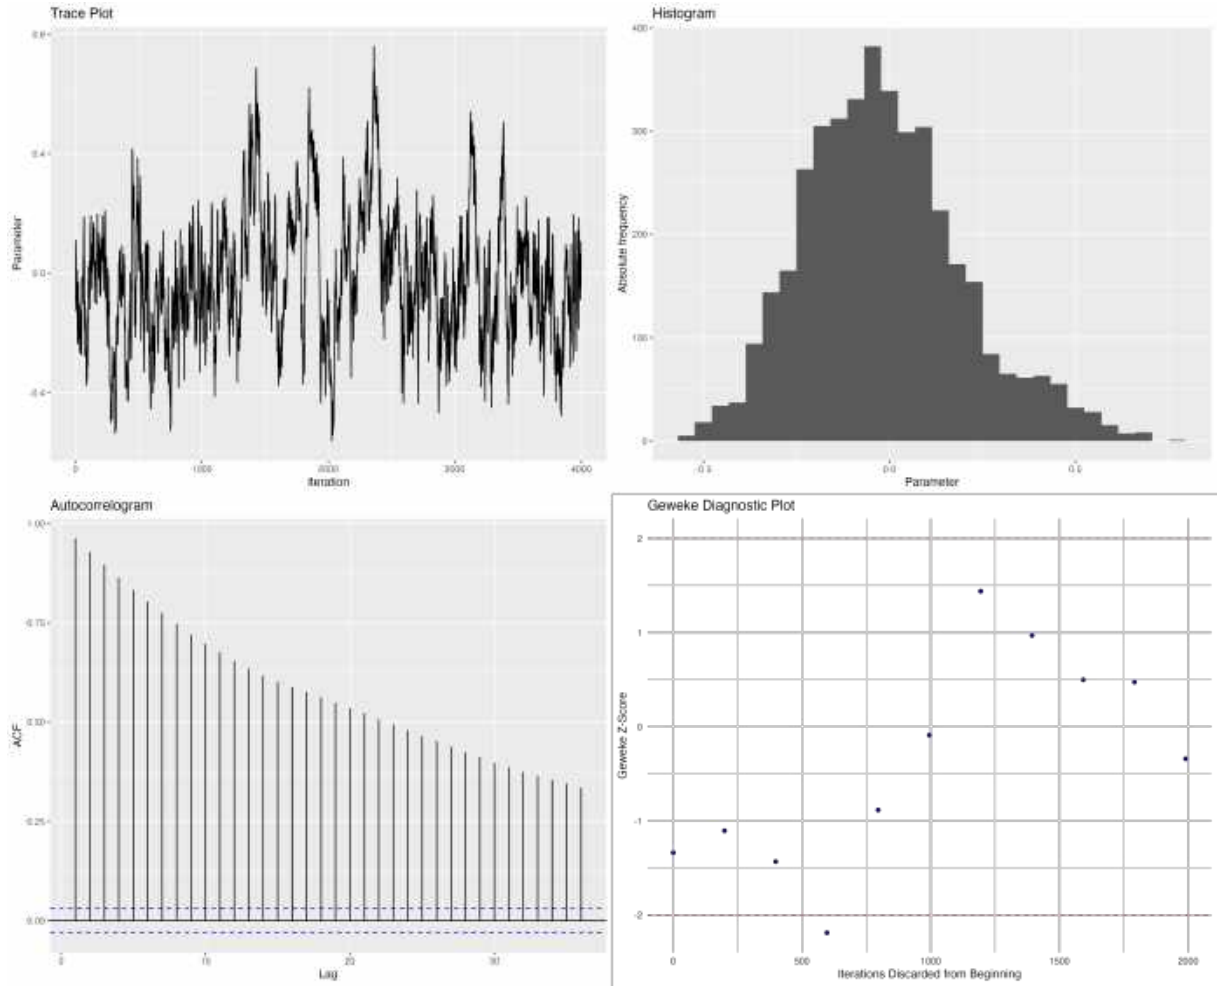

Figure S45: Convergence diagnostic plots for the parameter  $\log(\beta_1)$  in the district of Adamaoua.

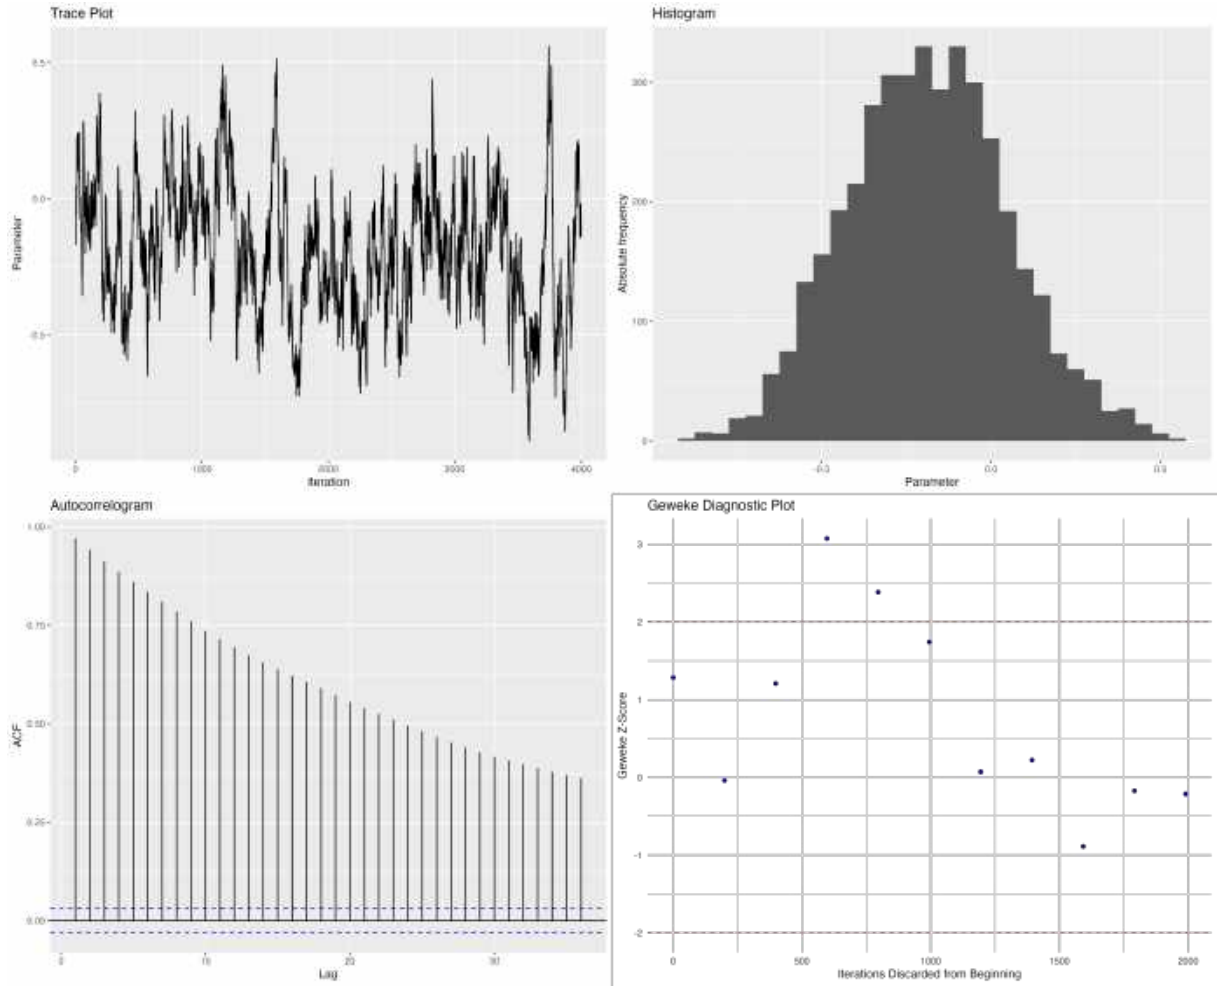

Figure S46: Convergence diagnostic plots for the parameter  $\log(\beta_2)$  in the district of Adamaoua.

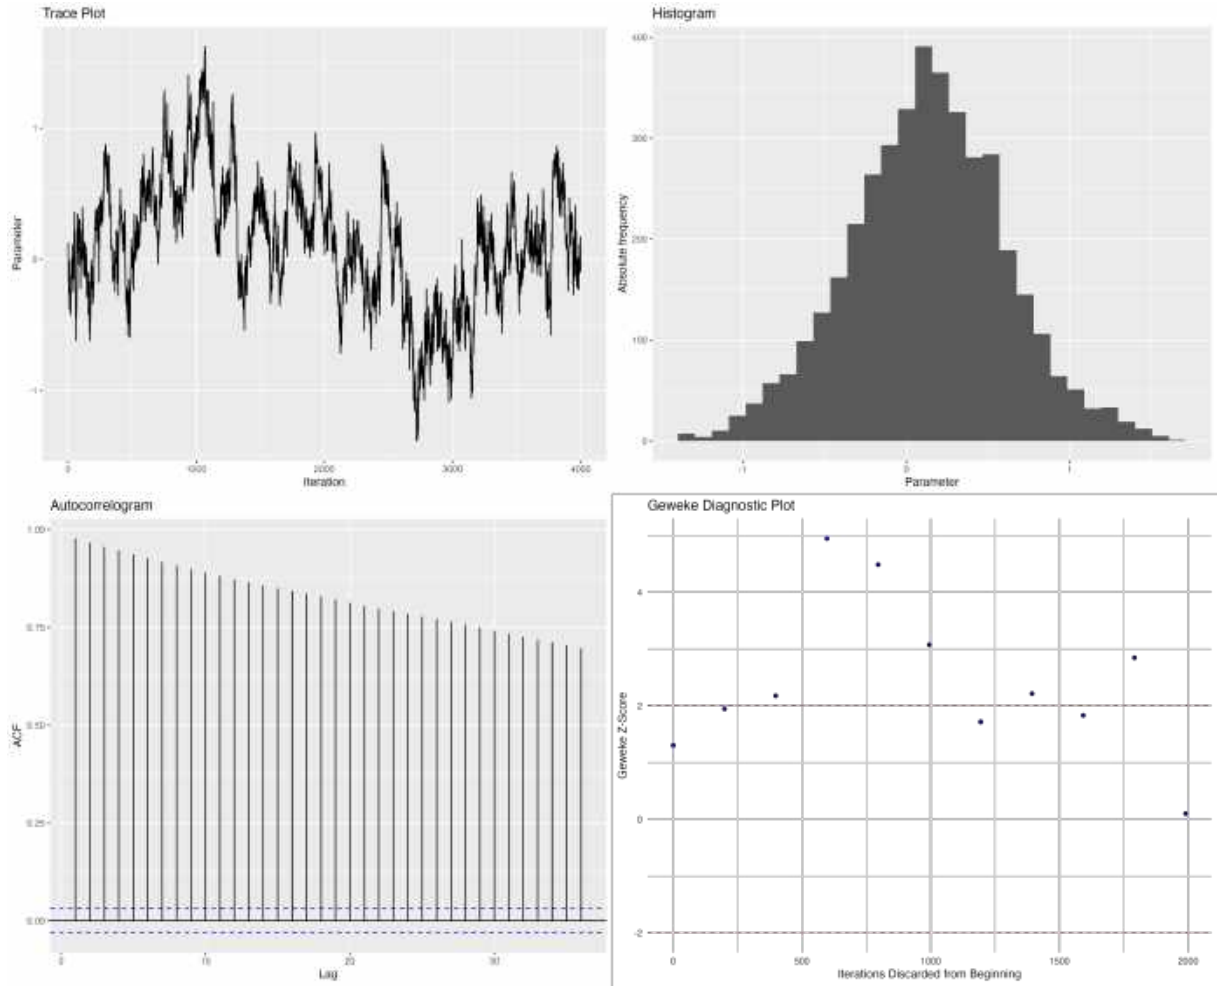

Figure S47: Convergence diagnostic plots for the parameter  $S_{11}$  in the district of Adamaoua.

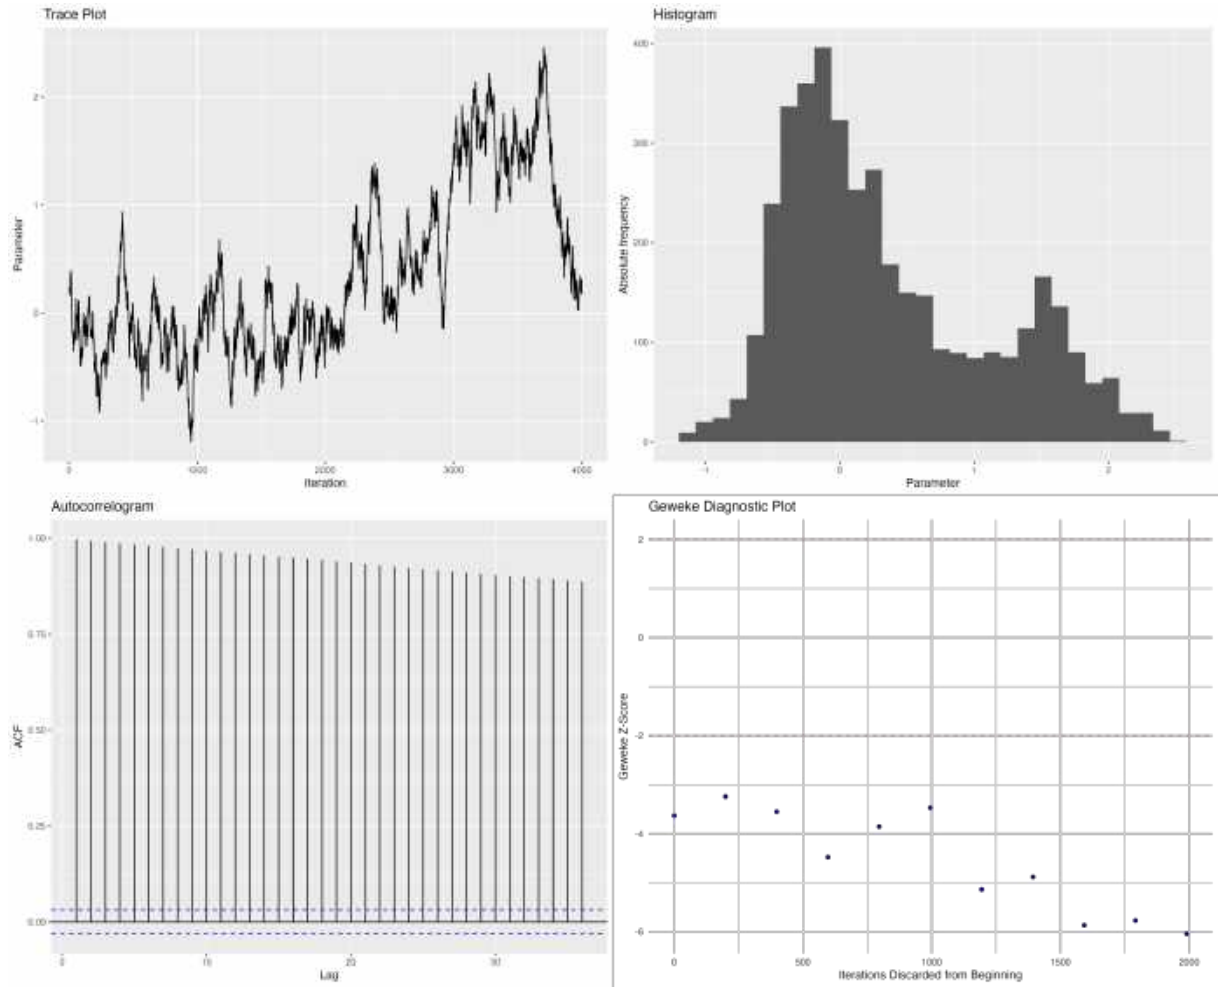

Figure S48: Convergence diagnostic plots for the parameter  $\log(\sigma^2)$  in the district of Nord.

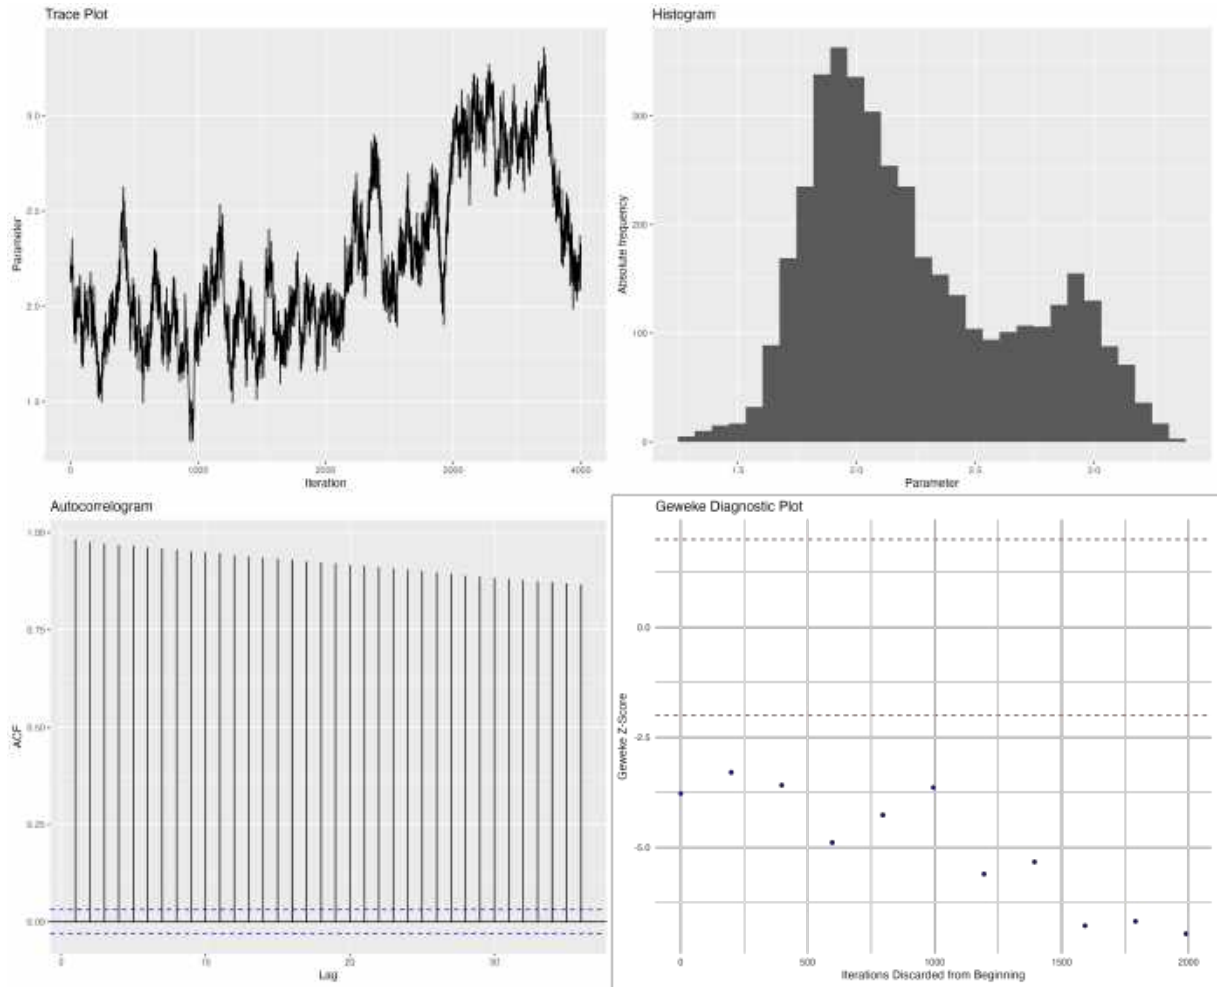

Figure S49: Convergence diagnostic plots for the parameter  $\log(\phi)$  in the district of Nord.

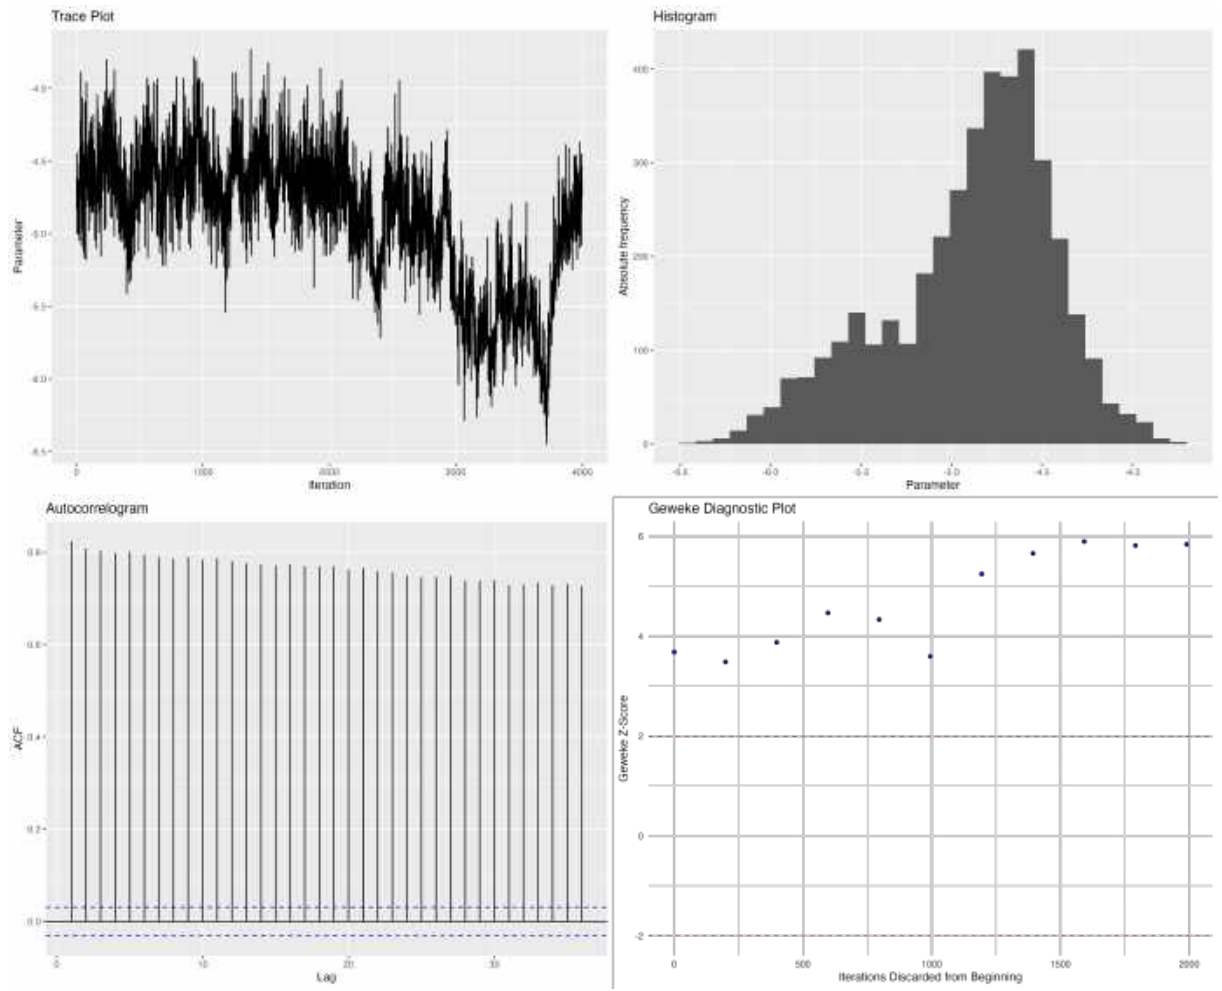

Figure S50: Convergence diagnostic plots for the parameter  $\log(\nu^2)$  in the district of Nord.



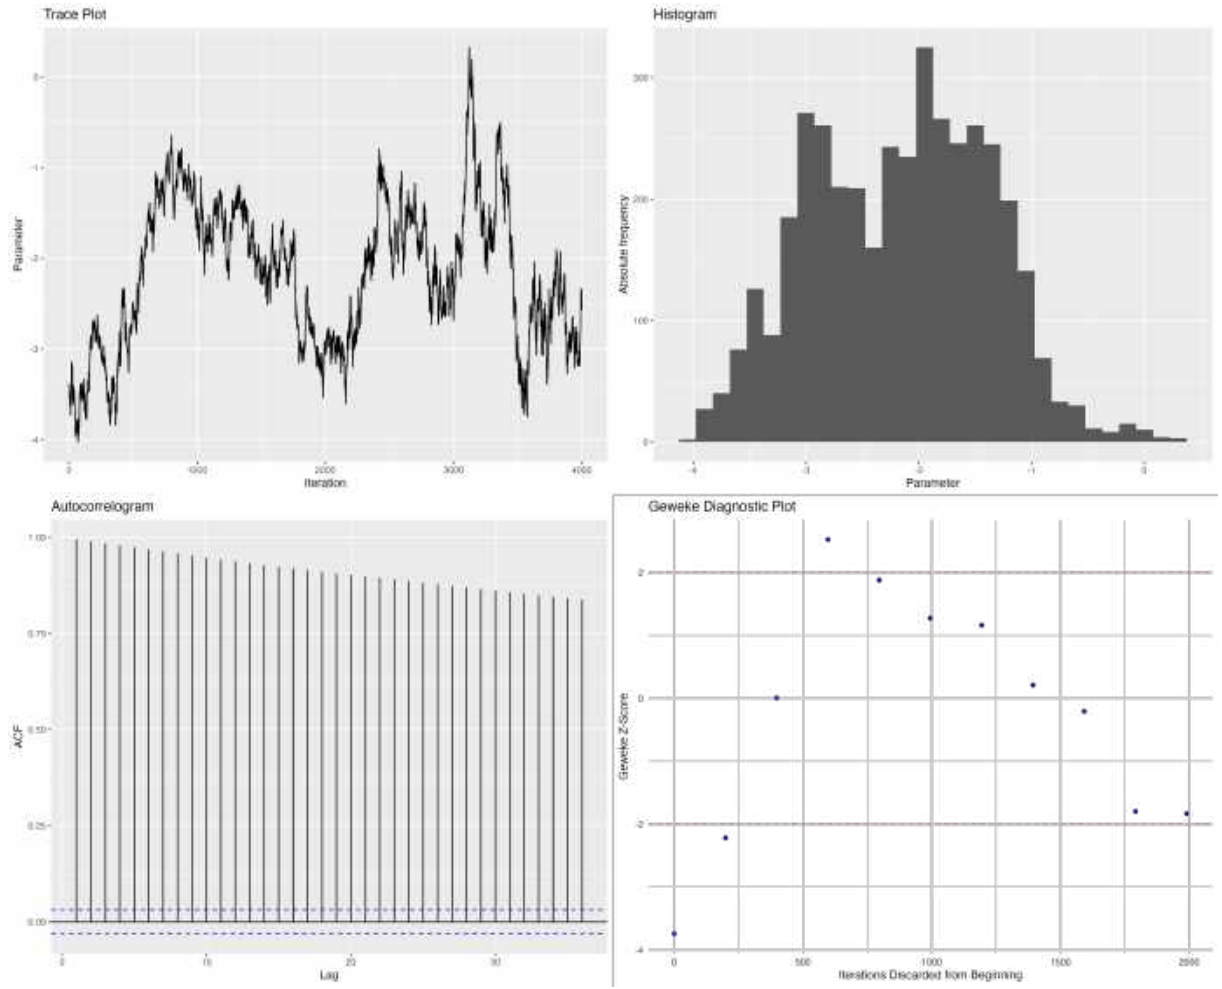

Figure S51: Convergence diagnostic plots for the parameter  $\log(\beta_0)$  in the district of Nord.

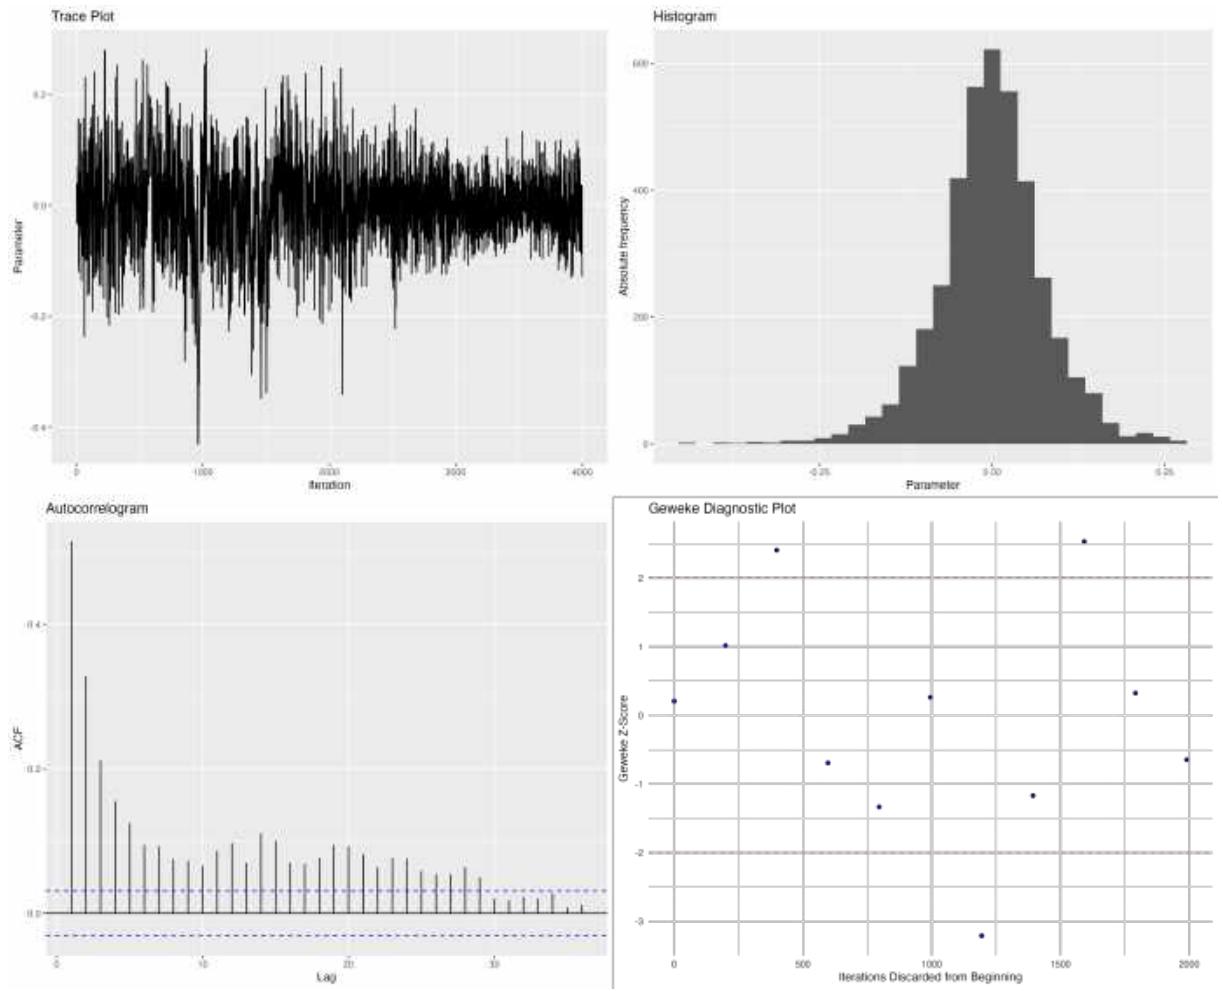

Figure S52: Convergence diagnostic plots for the parameter  $\log(\beta_1)$  in the district of Nord.

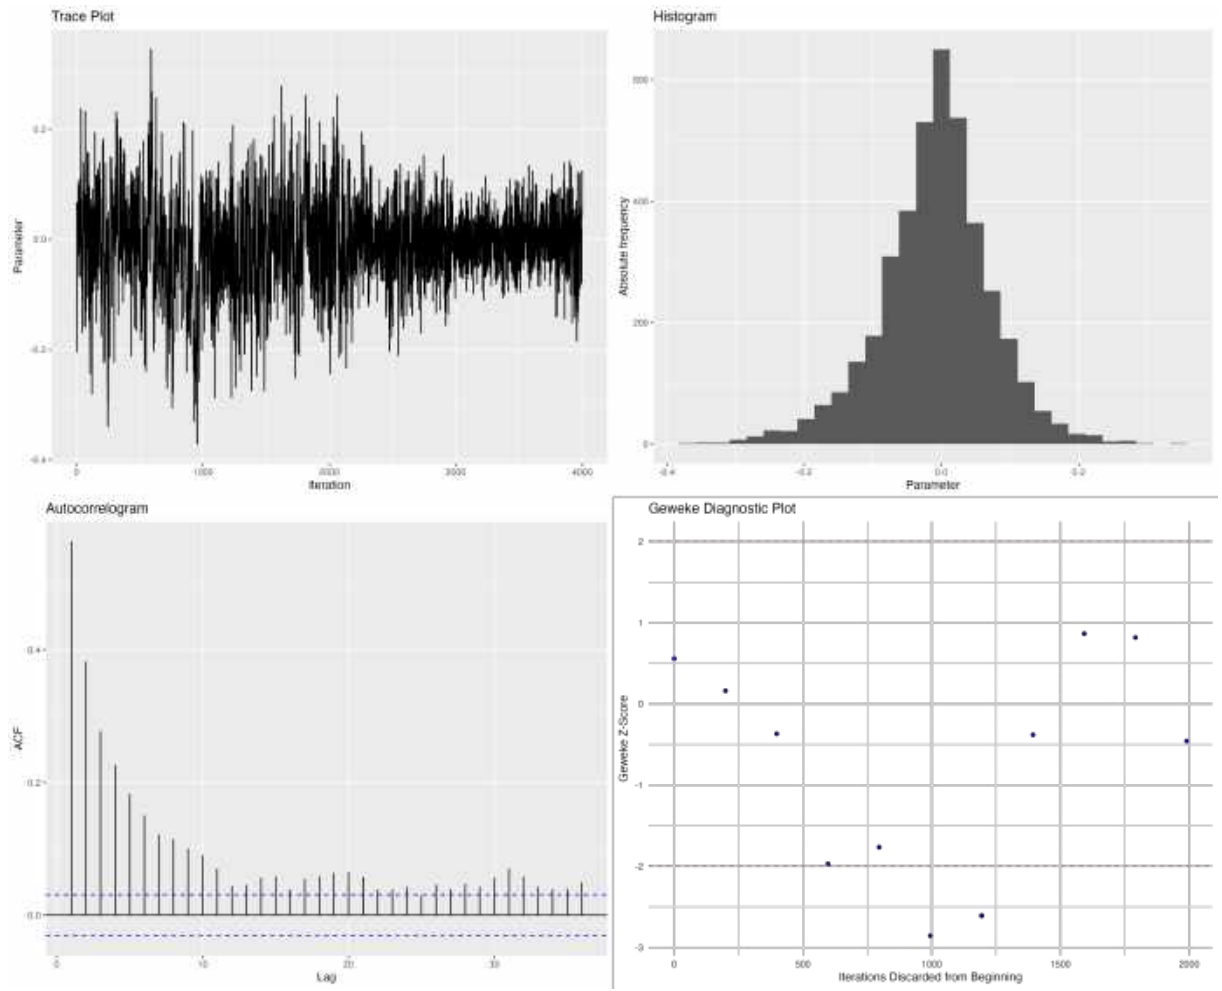

Figure S53: Convergence diagnostic plots for the parameter  $\log(\beta_2)$  in the district of Nord.

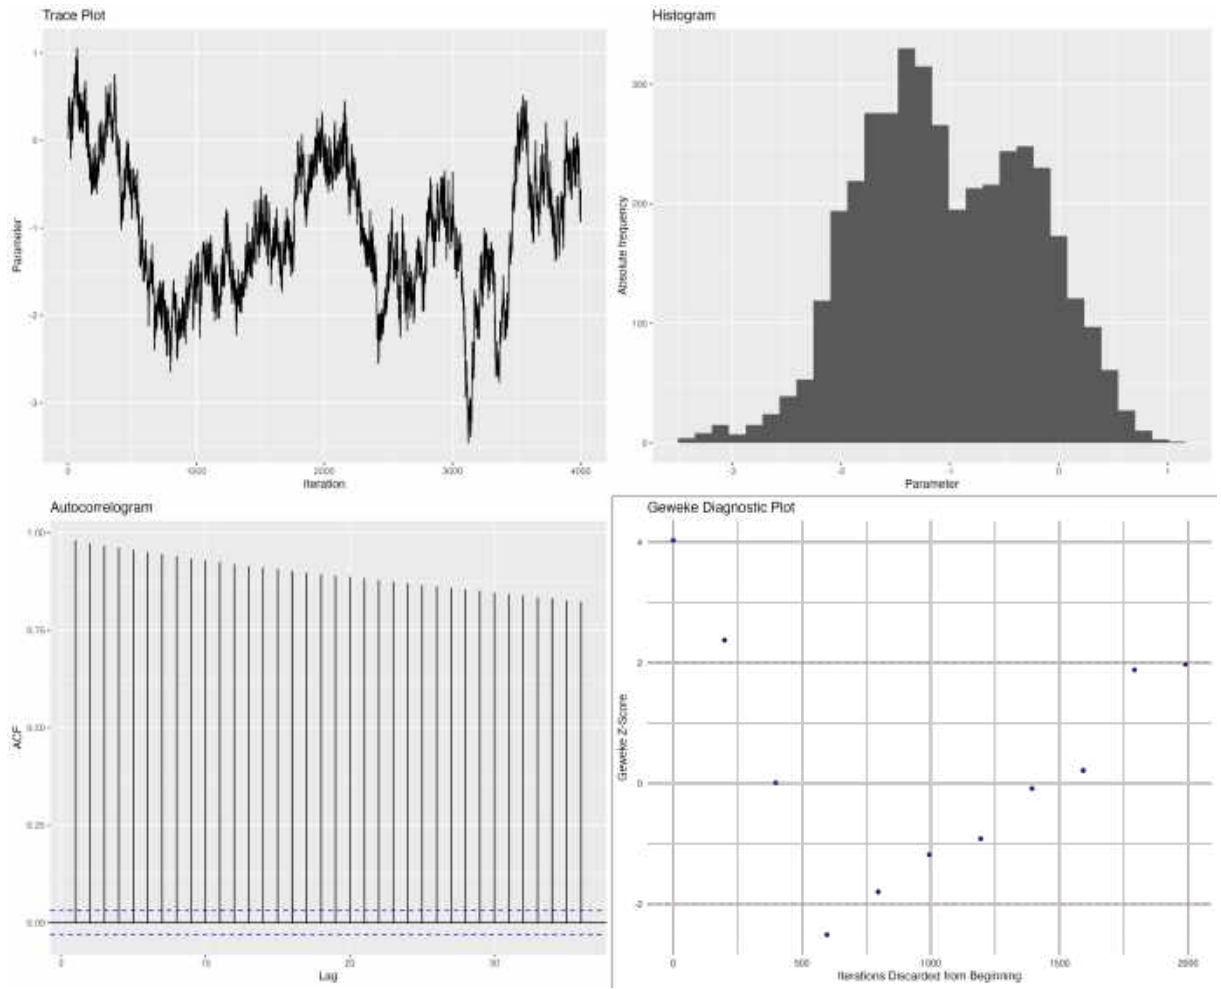

Figure S54: Convergence diagnostic plots for the parameter  $S_{11}$  in the district of Nord.

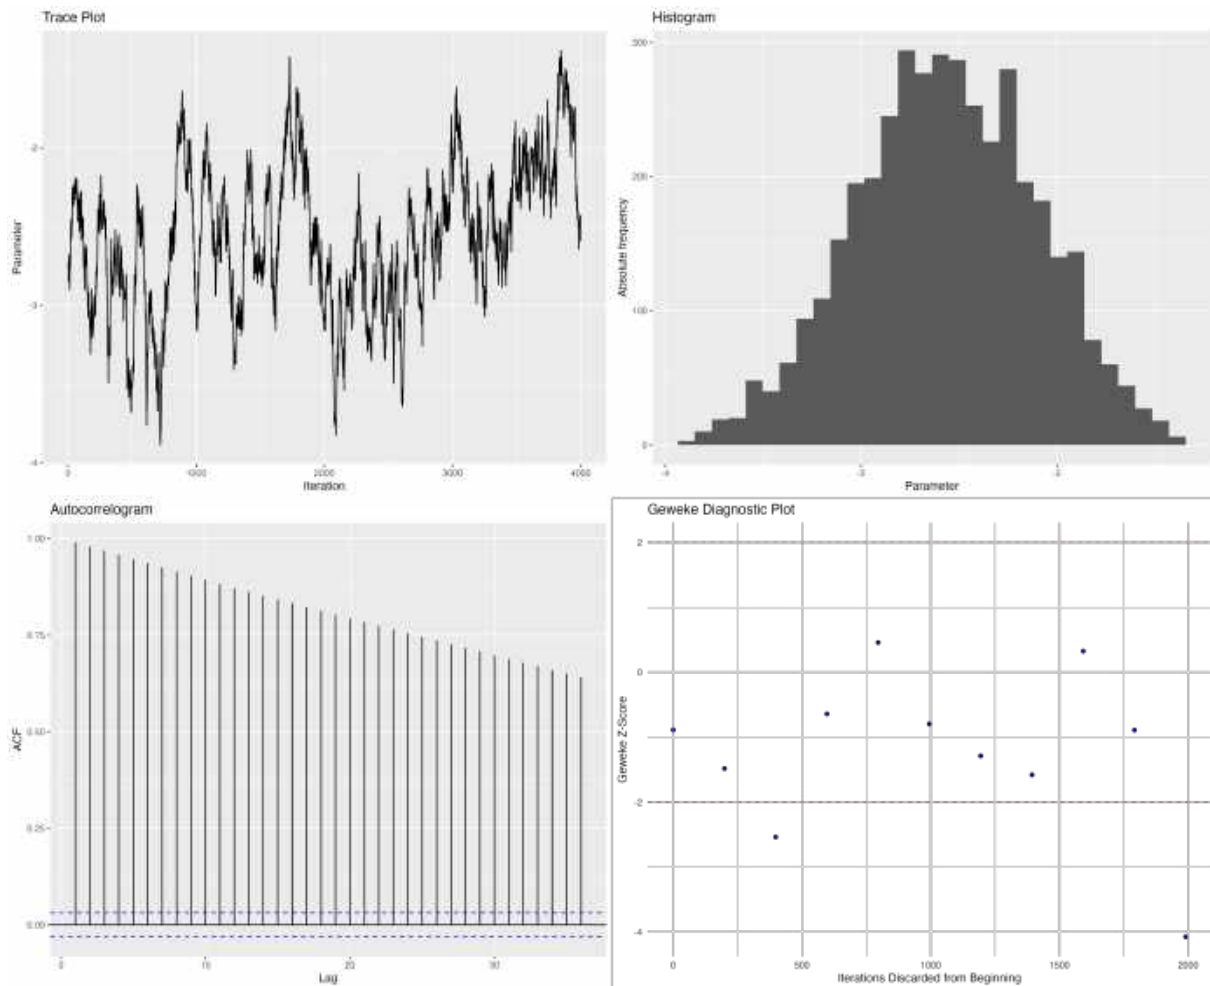

Figure S55: Convergence diagnostic plots for the parameter  $\log(\sigma^2)$  in the district of Nord-Ouest.

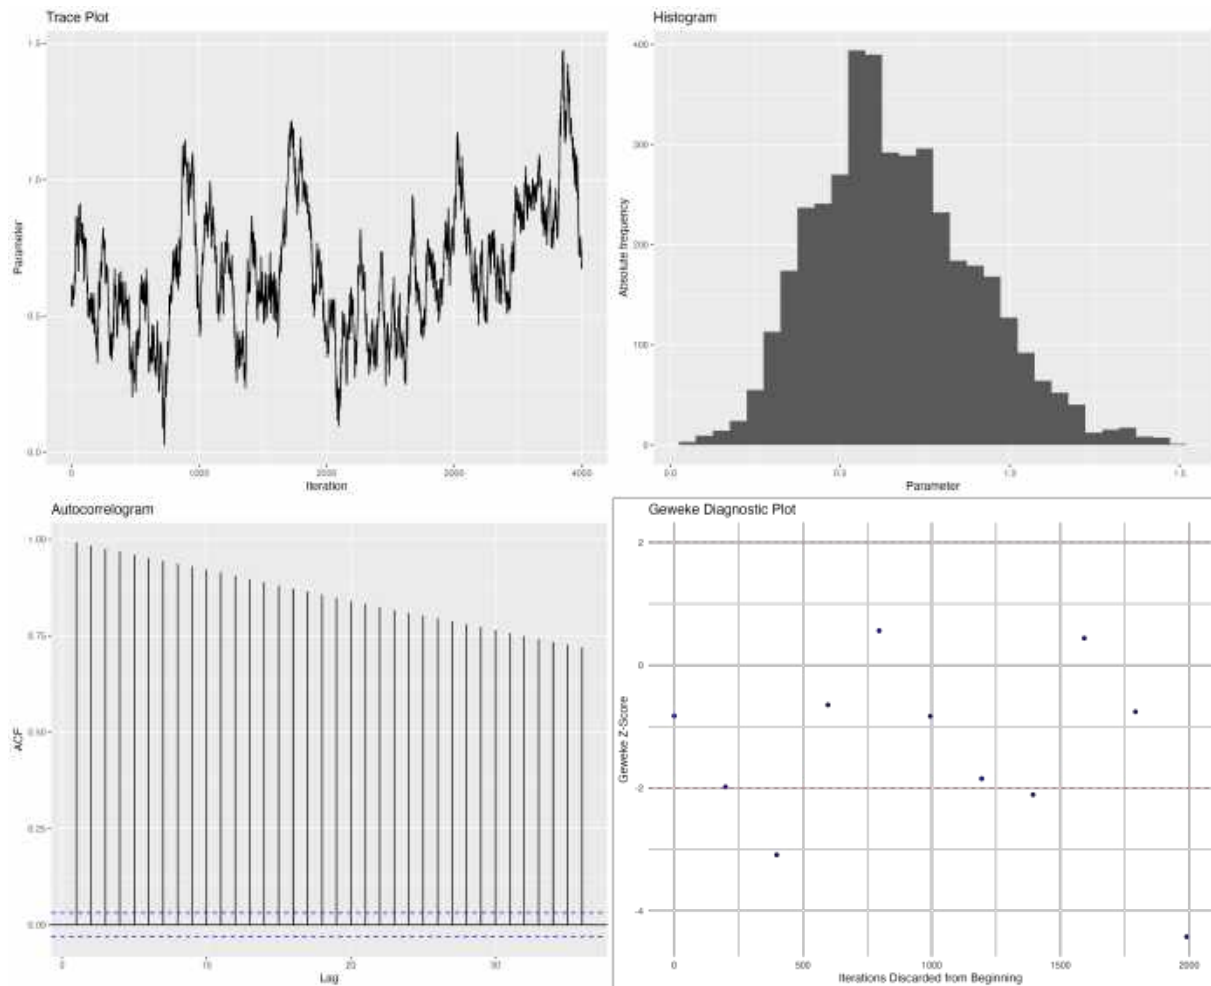

Figure S56: Convergence diagnostic plots for the parameter  $\log(\phi)$  in the district of Nord-Ouest.

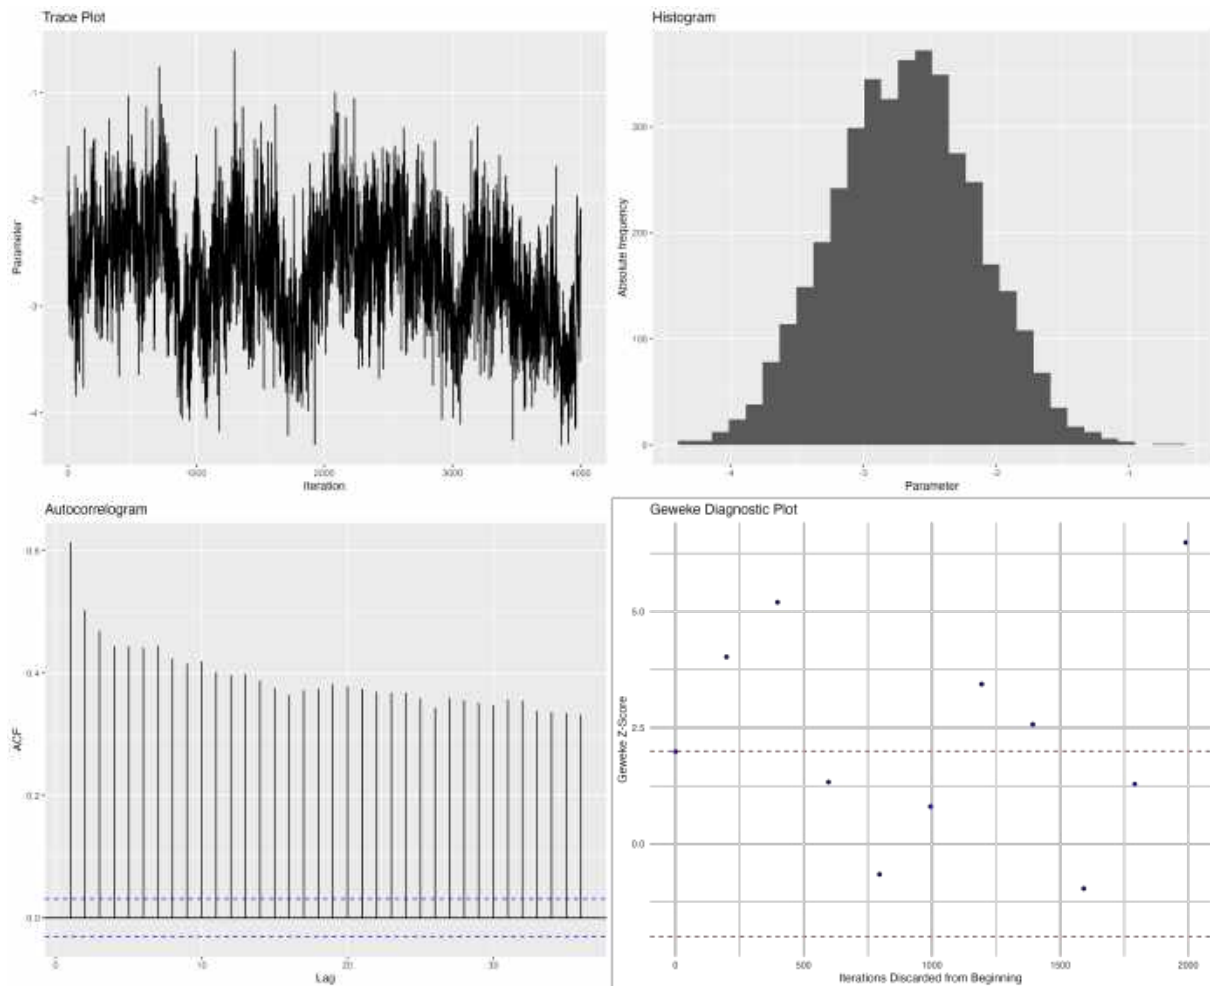

Figure S57: Convergence diagnostic plots for the parameter  $\log(\nu^2)$  in the district of Nord-Ouest.

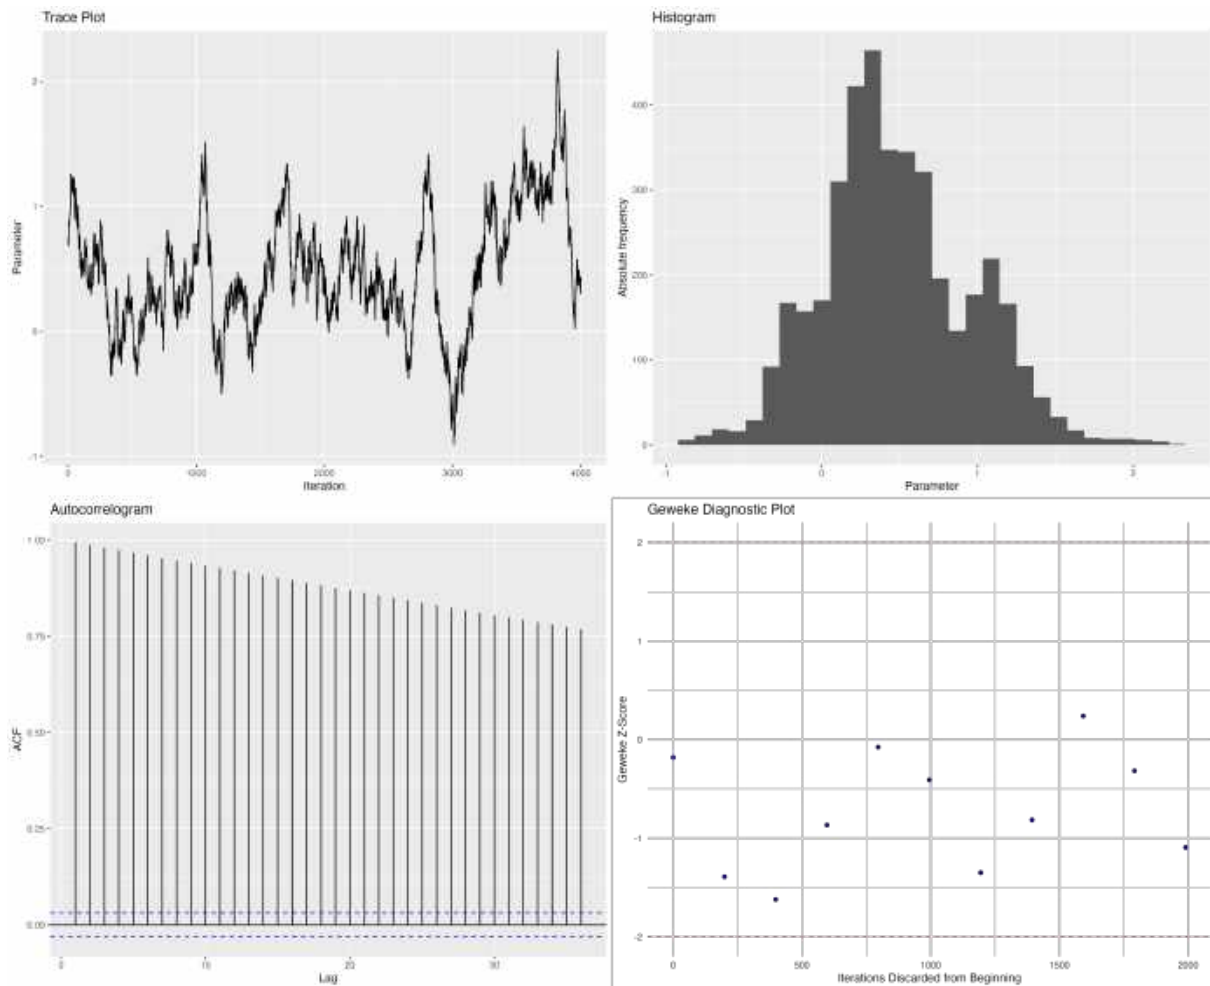

Figure S58: Convergence diagnostic plots for the parameter  $\log(\beta_0)$  in the district of Nord-Ouest.



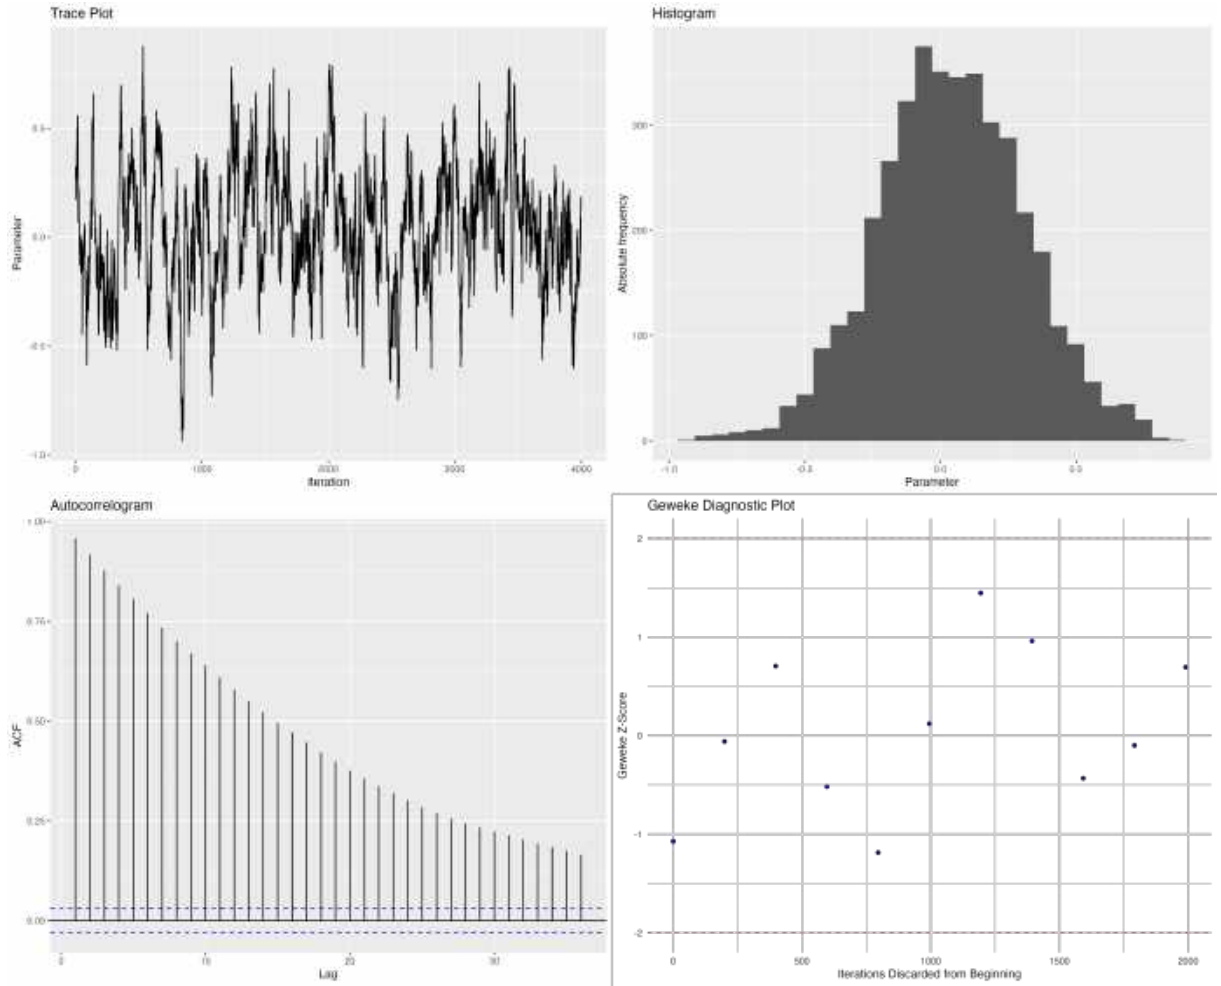

Figure S59: Convergence diagnostic plots for the parameter  $\log(\beta_1)$  in the district of Nord-Ouest.

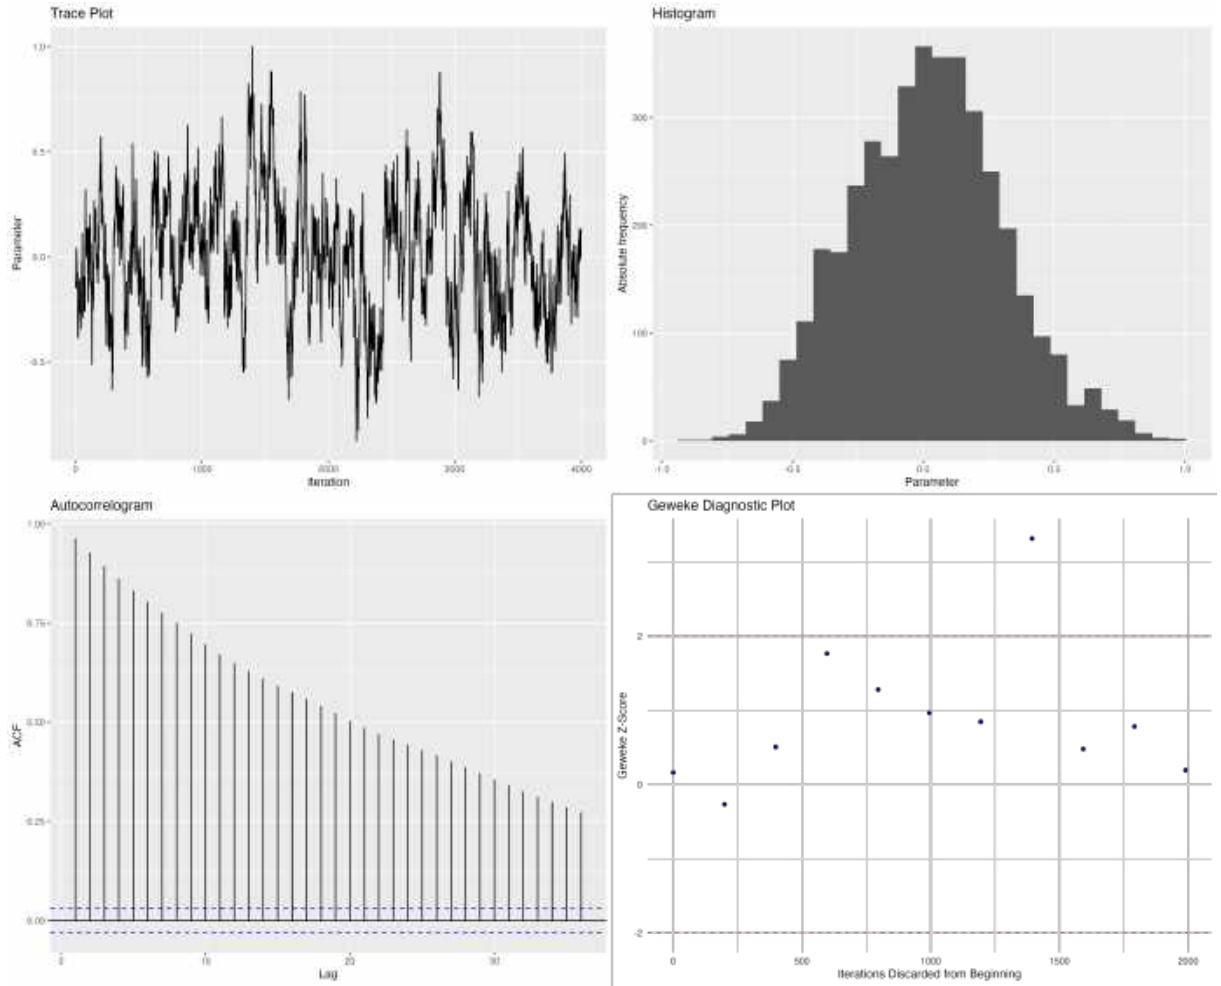

Figure S60: Convergence diagnostic plots for the parameter  $\log(\beta_2)$  in the district of Nord-Ouest.

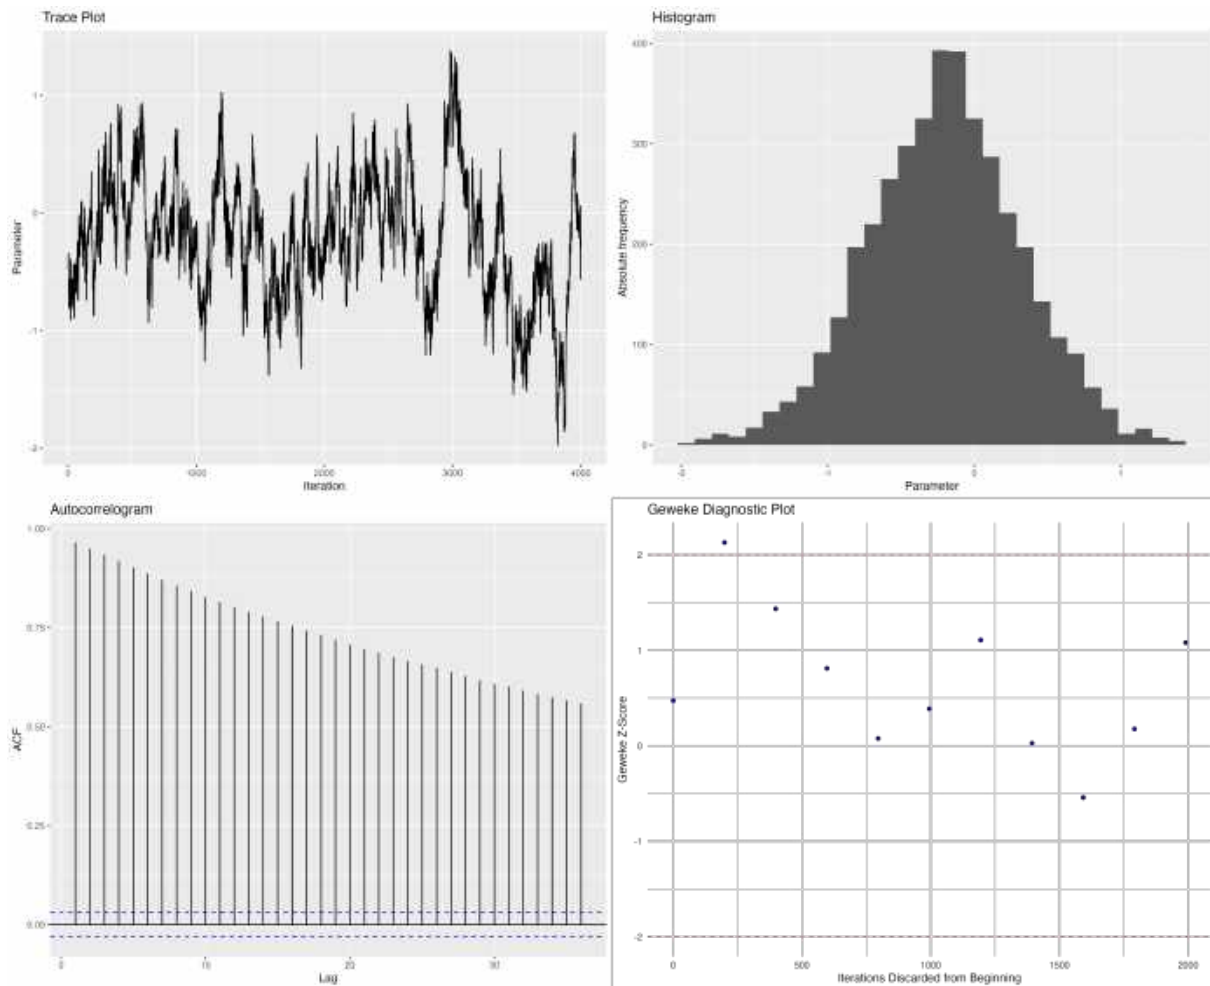

Figure S61: Convergence diagnostic plots for the parameter  $S_{i1}$  in the district of Nord-Ouest.

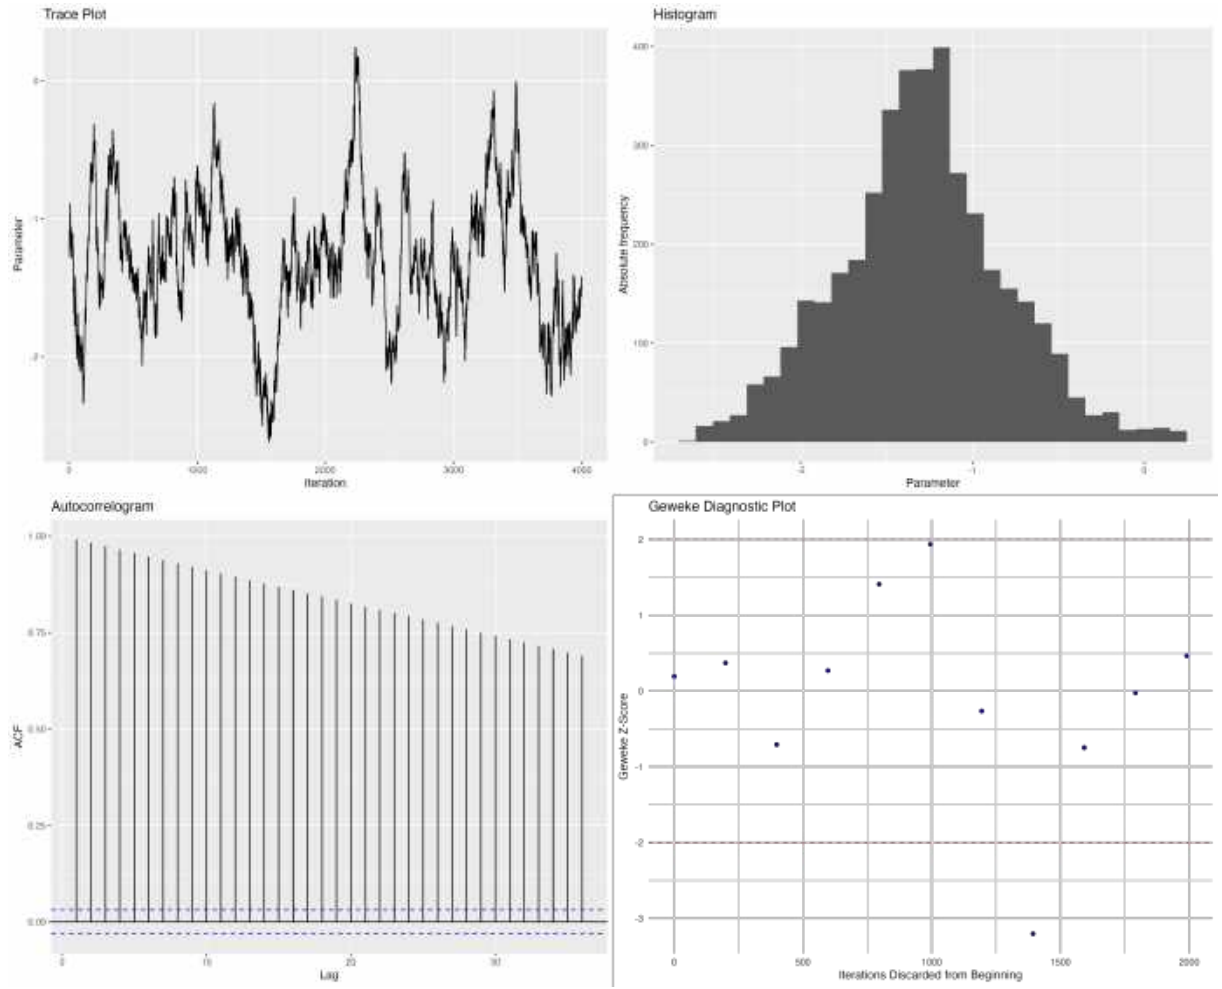

Figure S62: Convergence diagnostic plots for the parameter  $\log(\sigma^2)$  in the district of Sud.

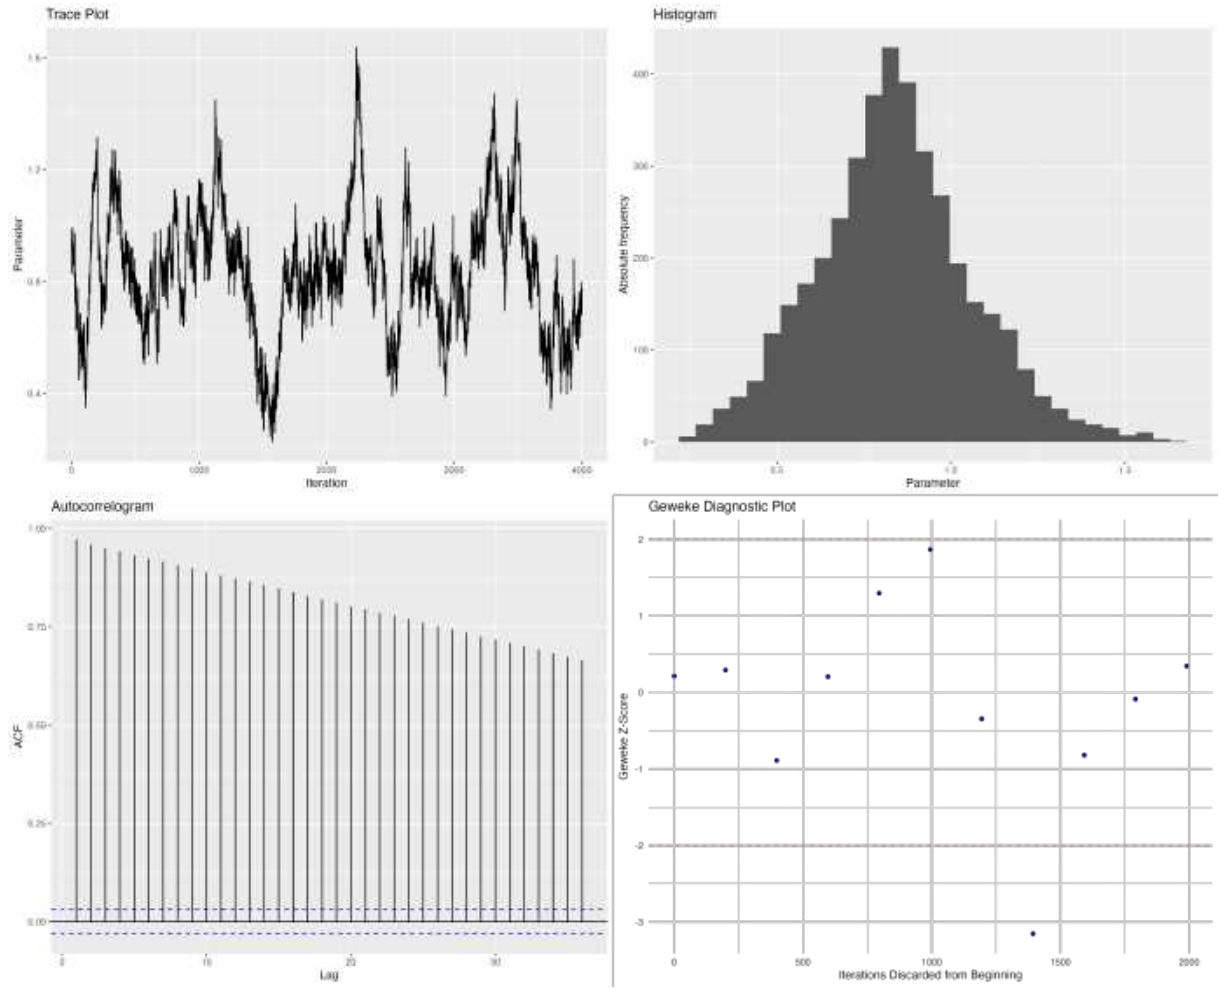

Figure S63: Convergence diagnostic plots for the parameter  $\log(\phi)$  in the district of Sud.

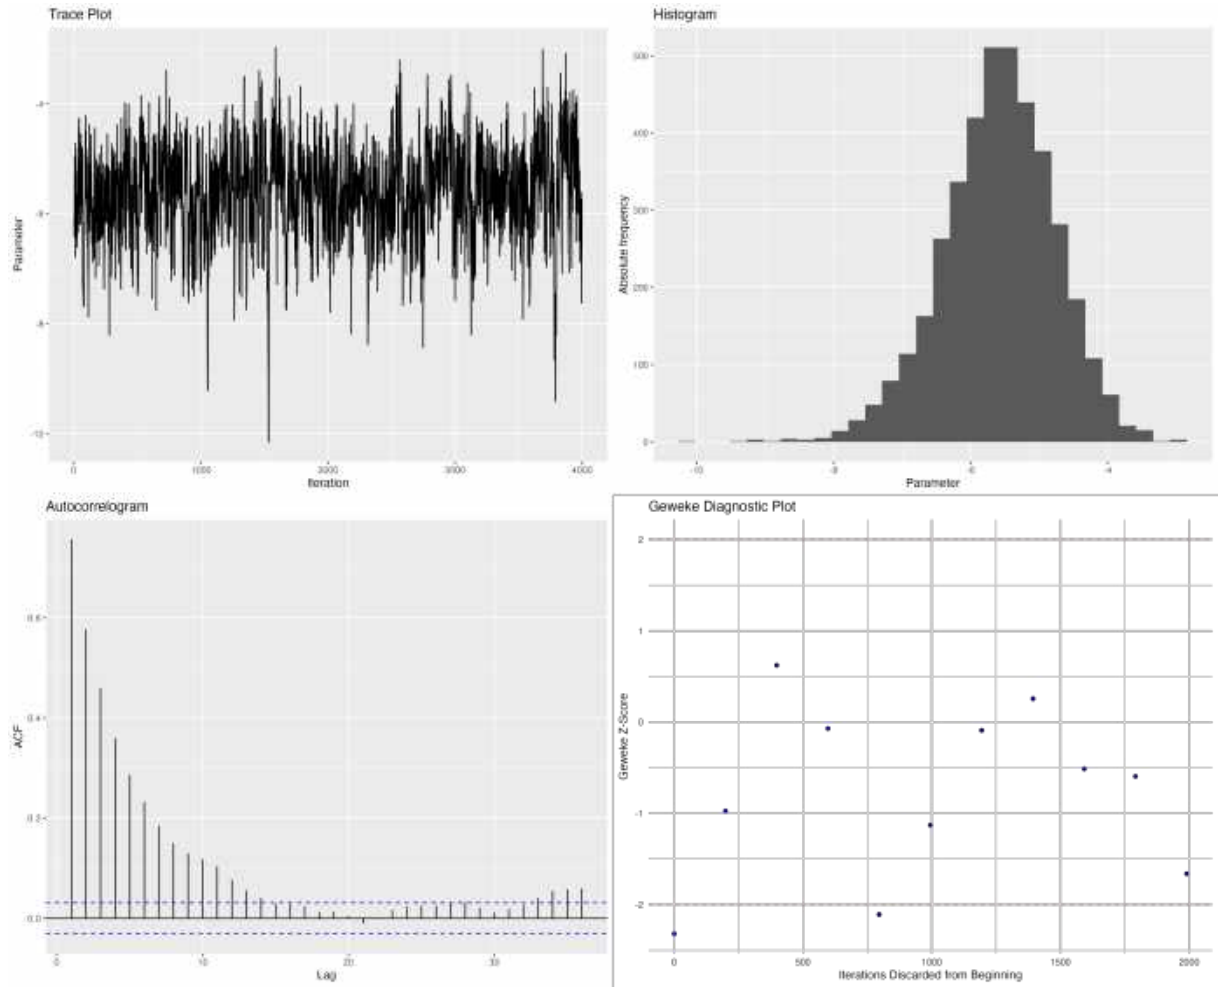

Figure S64: Convergence diagnostic plots for the parameter  $\log(\nu^2)$  in the district of Sud.

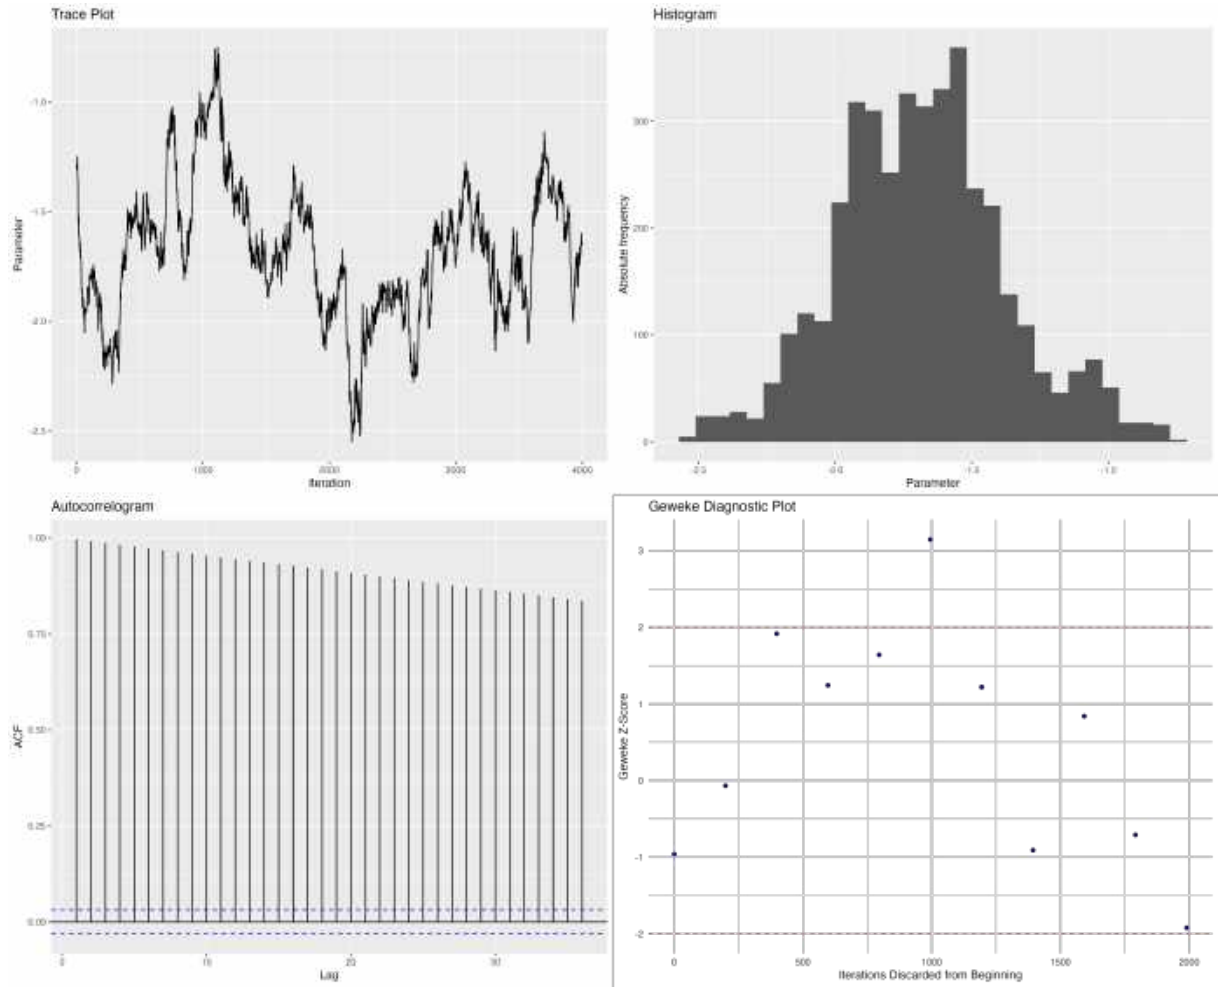

Figure S65: Convergence diagnostic plots for the parameter  $\log(\beta_0)$  in the district of Sud.

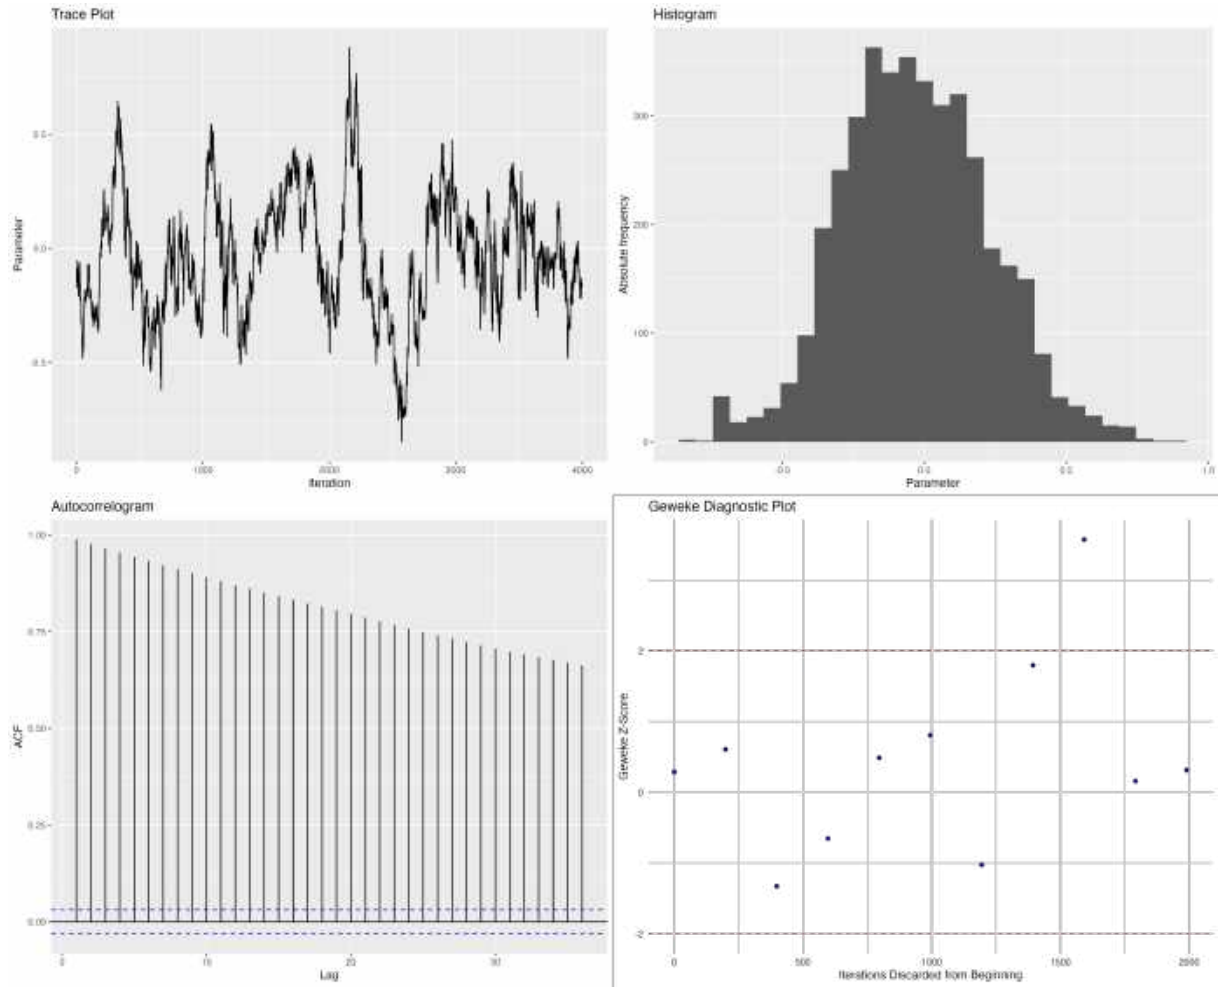

Figure S66: Convergence diagnostic plots for the parameter  $\log(\beta_1)$  in the district of Sud.



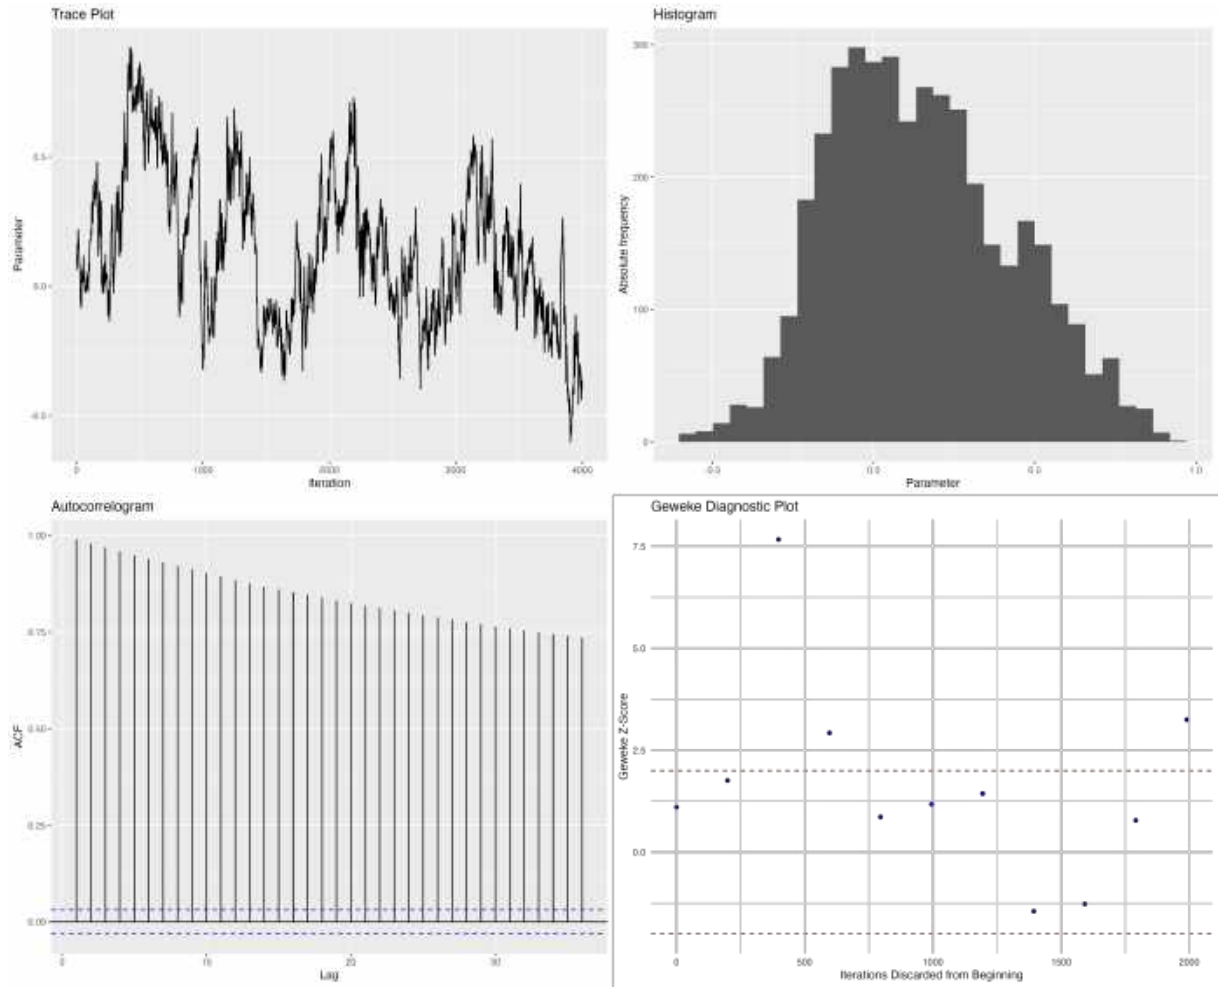

Figure S67: Convergence diagnostic plots for the parameter  $\log(\beta_2)$  in the district of Sud.

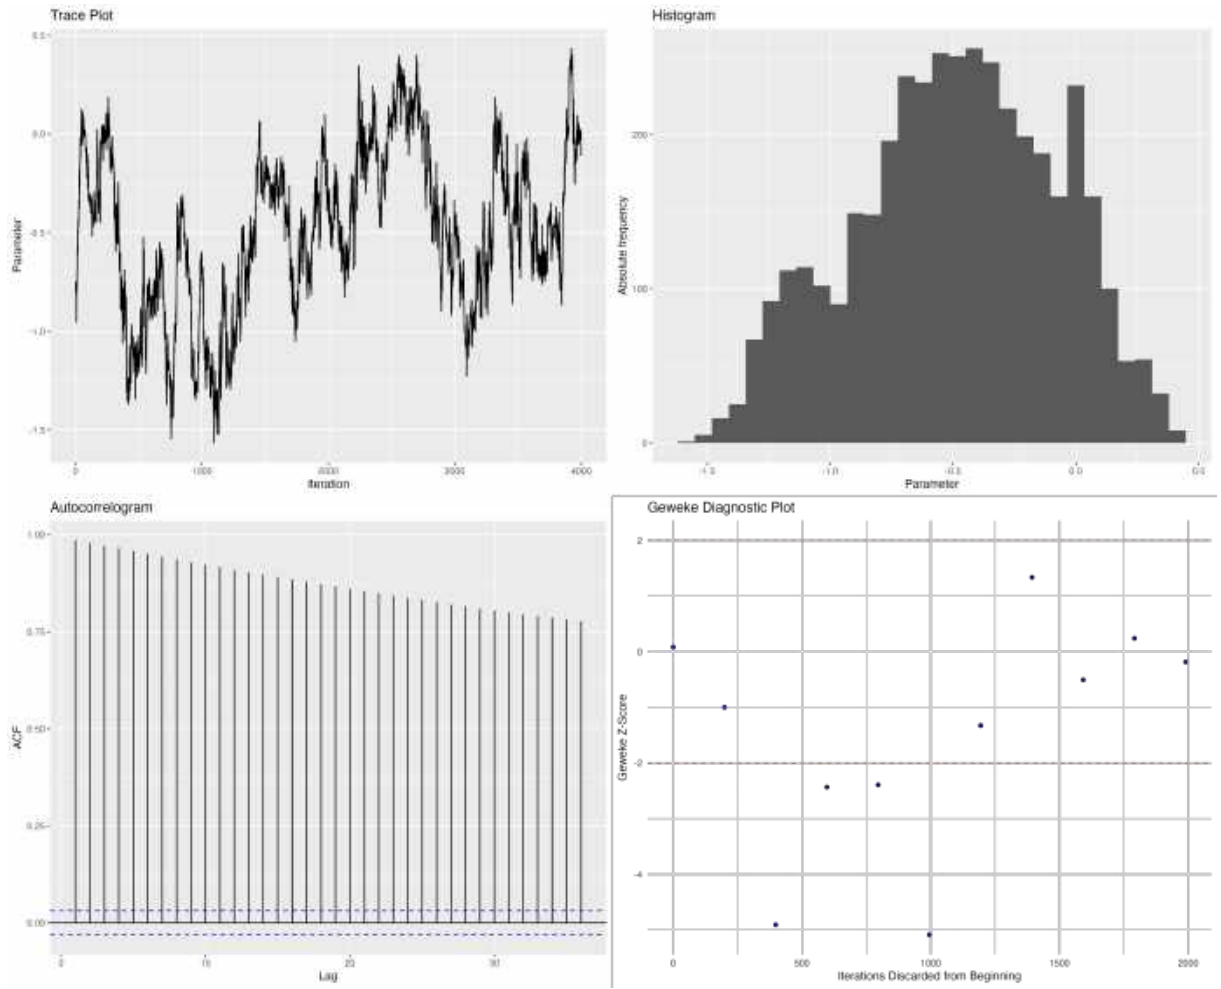

Figure S68: Convergence diagnostic plots for the parameter  $S_{i1}$  in the district of Sud.

## 2.4 Food security in Cameroon - Model comparison

Figure S69 and S70 compare the performance of the models in the training and test set using the Root Mean Squared Error (RMSE) and the Mean Absolute Error (MAE) respectively.

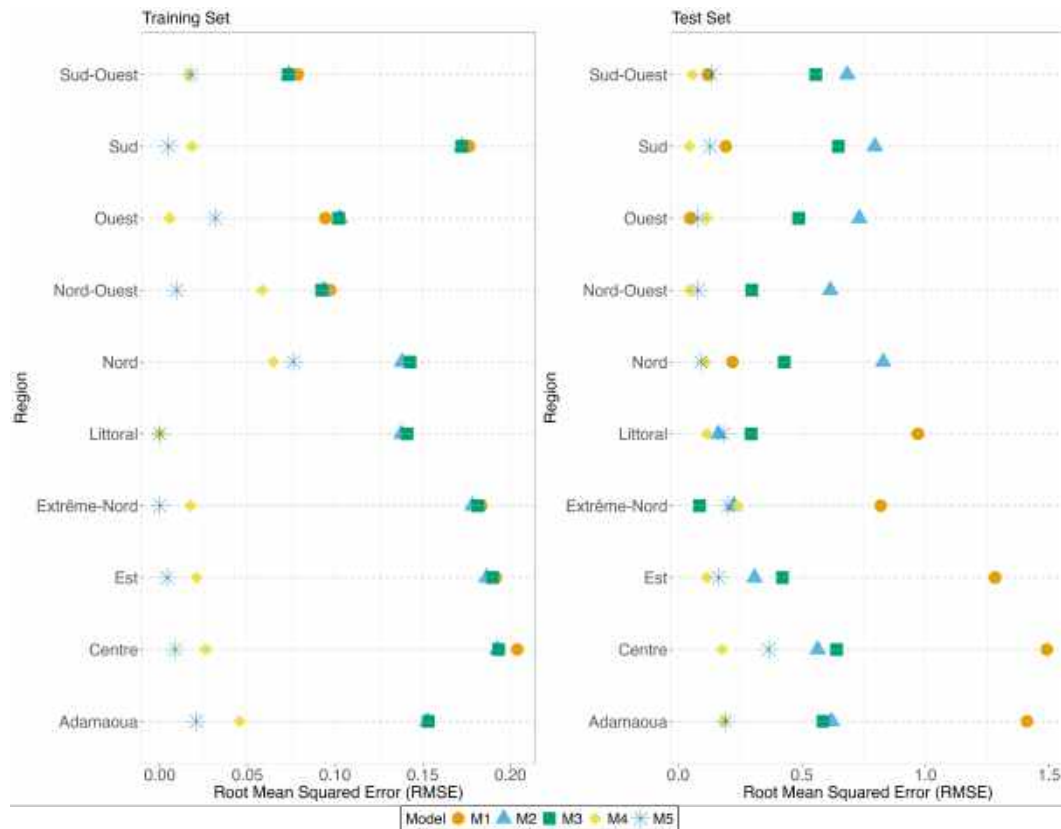

Figure S69: Comparison of model performance on the **training set** and **test set** for food security in Cameroon, using the Root Mean Squared Error.

Figure S71 displays the district-level distribution of CRPS values for the regions of Adamaoua and Est.

Figure S72 displays the district-level distribution of CRPS values for the regions of Centre and Extreme-Nord.

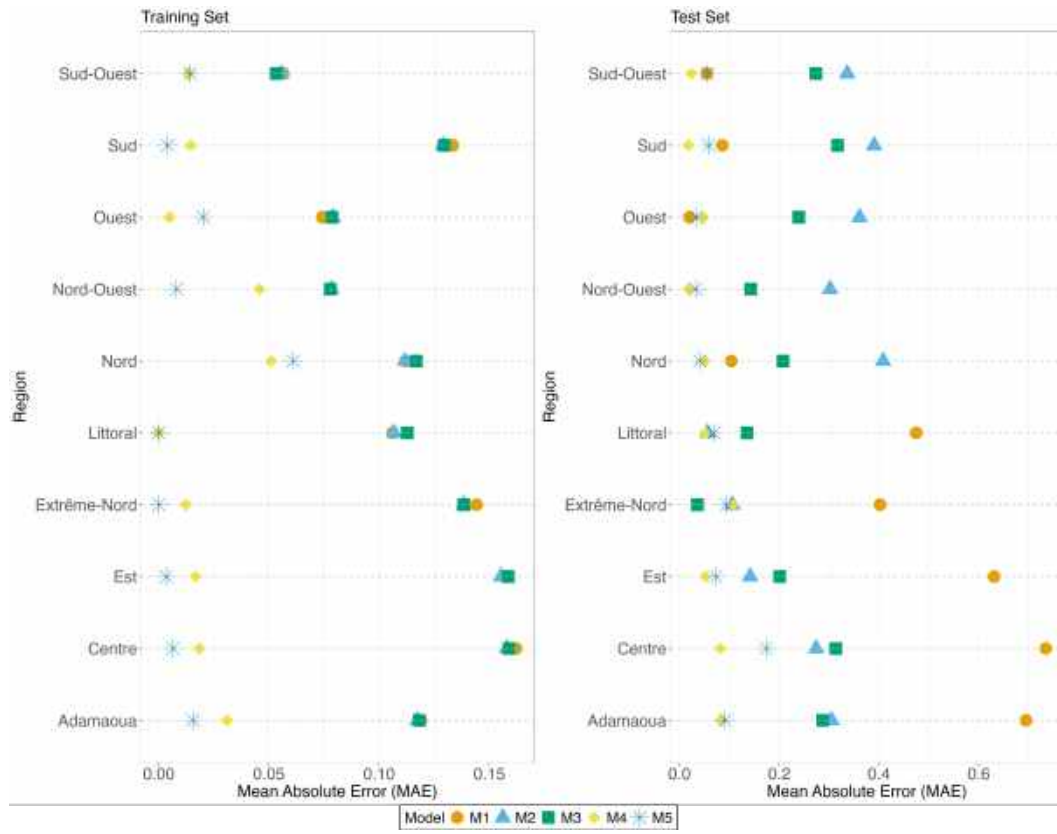

Figure S70: Comparison of model performance on the **training set** and **test set** for food security in Cameroon, using the Mean Absolute Error.

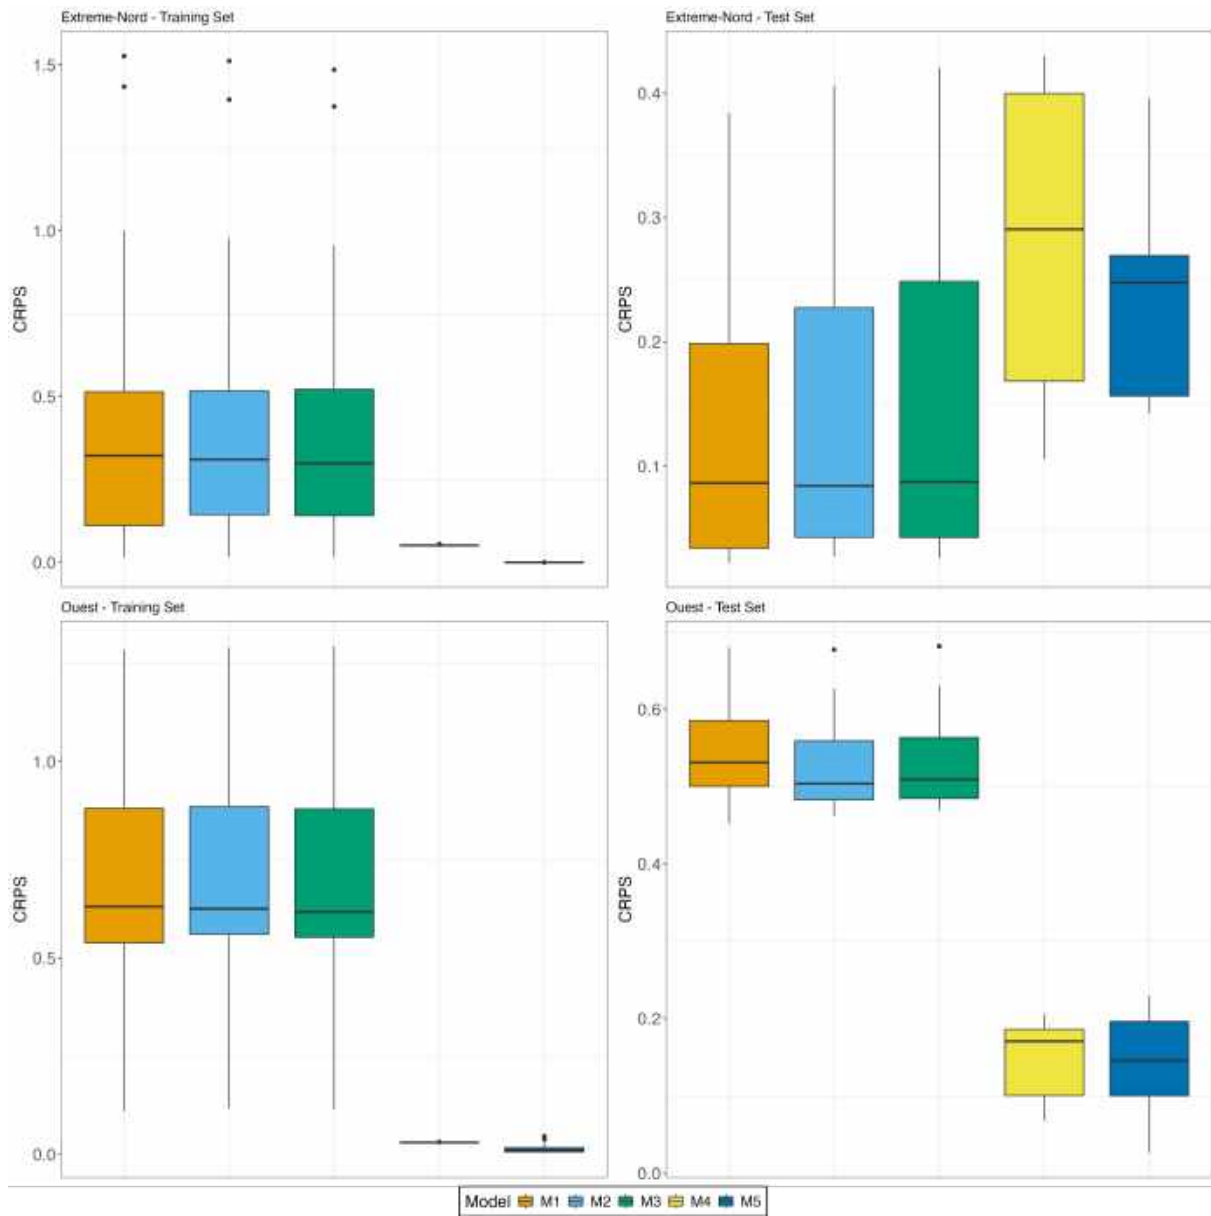

Figure S71: Regional distribution of the Continuous Ranked Probability Score (CRPS) for the food security example. Results are shown for the training set (**left panels**) and the test set (**right panels**), specifically Adamaoua (**top panels**) and Est (**bottom panels**) regions in Cameroon.

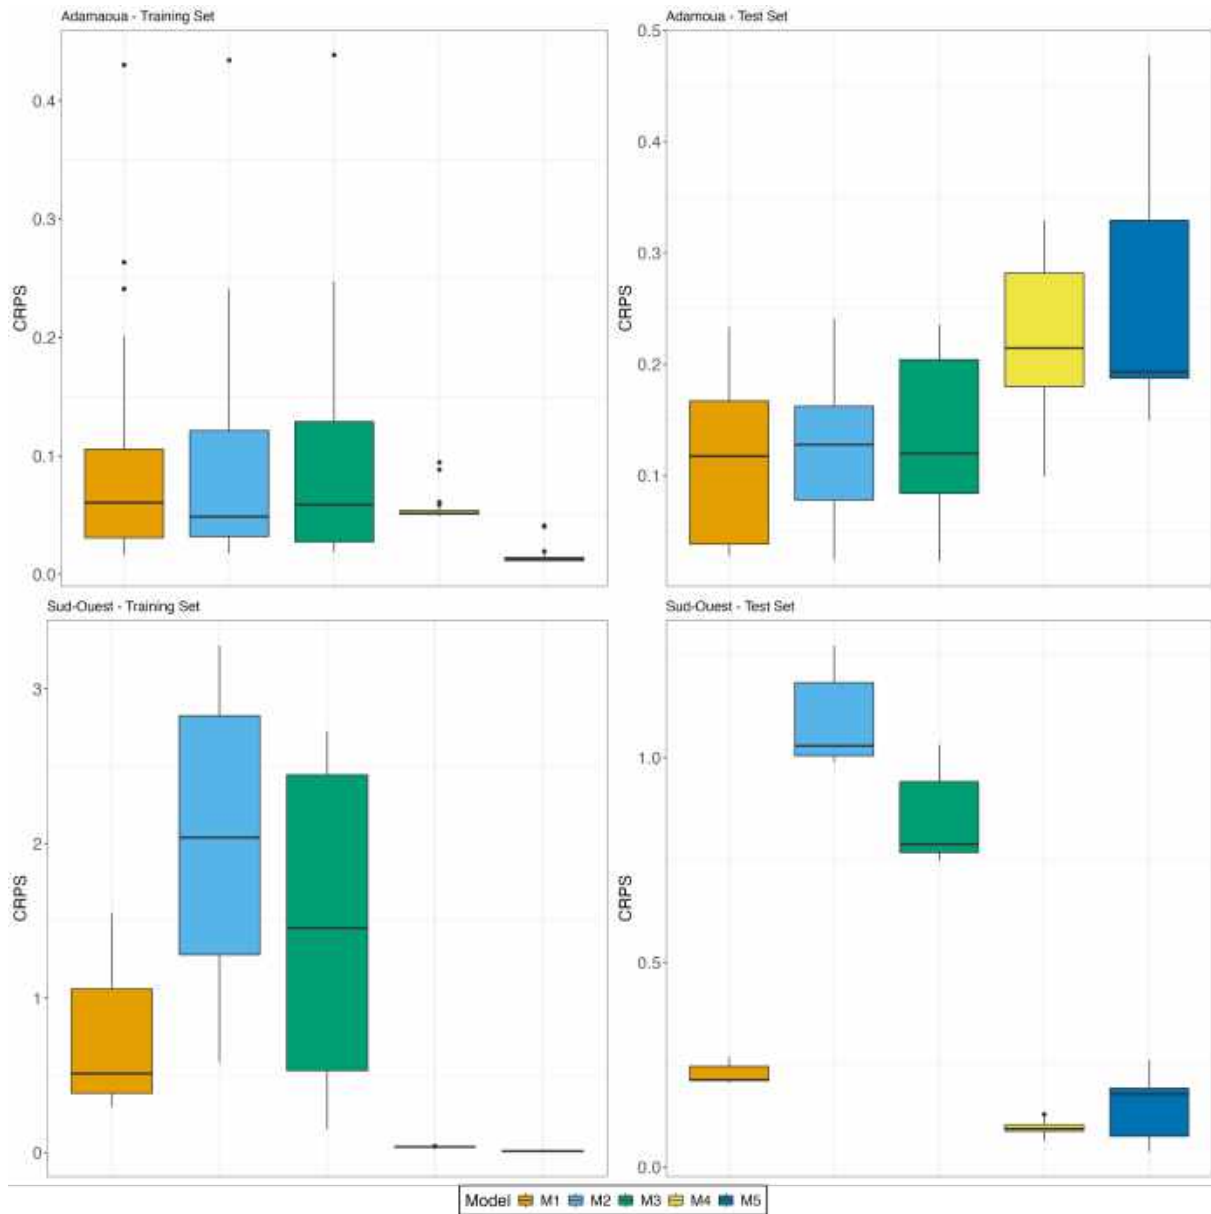

Figure S72: Regional distribution of the Continuous Ranked Probability Score (CRPS) for the food security example. Results are shown for the training set (**left panels**) and the test set (**right panels**), specifically Centre (**top panels**) and Extreme-Nord (**bottom panels**) regions in Cameroon.
